# Supplementary material for: Isomorph-based empirically modified hypernetted-chain approach for strongly coupled Yukawa one-component plasmas
Source: arXiv:1901.07131 ancillary file (2019-04-12)
Supplement: Supplementary file 1 [file Supplementary_material.pdf]

# Isomorph-based empirically modified hypernetted-chain approach for strongly coupled Yukawa one-component plasmas; Supplementary material

P. Tolias and F. Lucco Castello
*Space and Plasma Physics, Royal Institute of Technology, Stockholm, SE-100 44, Sweden*

Supplementary material for the manuscript entitled "Isomorph-based empirically modified hypernetted-chain approach for strongly coupled Yukawa one-component plasmas". Comparisons of structural and thermodynamic properties are carried out with the results of computer simulations (molecular dynamics, Langevin dynamics, Monte Carlo) and the results of other integral theory approaches (hypernetted chain approximation, soft mean spherical approximation, discretized Rogers-Young method, empirically modified hypernetted chain approximation). A thermodynamic consistency test is also performed concerning the statistical and virial routes to the reduced excess inverse isothermal compressibility.

## Contents

**Tables 1a-1g**: Some key properties of the YOCP pair correlation function according to Langevin dynamics simulations and different integral theory approaches for $\kappa = 0$ and varying coupling parameters.
**Tables 2a-2g**: Some key properties of the YOCP pair correlation function according to Langevin dynamics simulations and different integral theory approaches for $\kappa = 1$ and varying coupling parameters.
**Tables 3a-3g**: Some key properties of the YOCP pair correlation function according to Langevin dynamics simulations and different integral theory approaches for $\kappa = 2$ and varying coupling parameters.
**Table 4**: The YOCP reduced excess internal energy due to particle-particle interactions according to molecular dynamics simulations and different integral theory approaches for $\kappa = \{0, 0.2, 0.4, 0.6\}$ and varying coupling parameters.
**Table 5**: The YOCP reduced excess internal energy due to particle-particle interactions according to molecular dynamics simulations and different integral theory approaches for $\kappa = \{0.8, 1.0, 1.2\}$ and varying coupling parameters.
**Table 6**: The YOCP reduced excess internal energy due to particle-particle interactions according to molecular dynamics simulations and different integral theory approaches for $\kappa = \{1.4, 2.0, 2.6, 3.0\}$ and varying coupling parameters.
**Table 7**: The YOCP reduced excess internal energy due to particle-particle interactions according to molecular dynamics simulations and different integral theory approaches for $\kappa = \{3.6, 4.0, 4.6, 5.0\}$ and varying coupling parameters.
**Table 8**: The YOCP virial reduced excess pressure due to particle-particle interactions according to Monte Carlo simulations and different integral theory approaches for varying $(\Gamma, \kappa)$ pairs.
**Tables 9a-9o**: The YOCP reduced excess inverse isothermal compressibility owing to the particle presence resulting from the statistical route and the virial route of different integral theory approaches for $\kappa = \{0, 0.2, 0.4, 0.6, 0.8, 1.0, 1.2, 1.4, 2.0, 2.6, 3.0, 3.6, 4.0, 4.6, 5.0\}$ and varying coupling parameters.

**Table 1a.** Key properties of the pair correlation function resulting from Langevin dynamics simulations and three integral theory approaches: the hypernetted-chain approximation (HNC), isomorph-based empirically modified hypernetted-chain approximation (IEMHNC) and empirically modified hypernetted-chain approximation (EMHNC). The absolute relative deviation $\epsilon_{\mathrm{r}}$ between the theoretical and the simulation results is also reported. **Results for $\arg_r\{g(r)=0.5\}$ in the case of $\kappa=0$**. The LD results are adopted from Table 4 of *T. Ott and M. Bonitz, Contrib. Plasma Phys.* **55**, *243 (2015)*. It should be pointed out that for the OCP, the IEMHNC and the EMHNC approaches are identical.

| $\Gamma$ | $\Gamma/\Gamma_{\mathrm{m}}$ | $r_{\mathrm{cv}}^{\mathrm{LD}}/d$ | $r_{\mathrm{cv}}^{\mathrm{HNC}}/d$ | $\epsilon_{\mathrm{HNC}}(\%)$ | $r_{\mathrm{cv}}^{\mathrm{IEMHNC}}/d$ | $\epsilon_{\mathrm{IEMHNC}}(\%)$ | $r_{\mathrm{cv}}^{\mathrm{EMHNC}}/d$ | $\epsilon_{\mathrm{EMHNC}}(\%)$ |
|---|---|---|---|---|---|---|---|---|
| 15.0 | 0.09 | 1.179 | 1.150 | 2.460 | 1.165 | 1.187 | 1.165 | 1.187 |
| 20.0 | 0.12 | 1.218 | 1.187 | 2.545 | 1.207 | 0.903 | 1.207 | 0.903 |
| 25.0 | 0.15 | 1.246 | 1.214 | 2.568 | 1.237 | 0.722 | 1.237 | 0.722 |
| 30.0 | 0.17 | 1.272 | 1.235 | 2.909 | 1.262 | 0.786 | 1.262 | 0.786 |
| 35.0 | 0.20 | 1.291 | 1.253 | 2.943 | 1.282 | 0.697 | 1.282 | 0.697 |
| 40.0 | 0.23 | 1.307 | 1.268 | 2.984 | 1.299 | 0.612 | 1.299 | 0.612 |
| 45.0 | 0.26 | 1.320 | 1.282 | 2.879 | 1.314 | 0.455 | 1.314 | 0.455 |
| 50.0 | 0.29 | 1.333 | 1.293 | 3.001 | 1.327 | 0.450 | 1.327 | 0.450 |
| 55.0 | 0.32 | 1.346 | 1.304 | 3.120 | 1.338 | 0.594 | 1.338 | 0.594 |
| 60.0 | 0.35 | 1.355 | 1.313 | 3.100 | 1.349 | 0.443 | 1.349 | 0.443 |
| 65.0 | 0.38 | 1.365 | 1.322 | 3.150 | 1.359 | 0.440 | 1.359 | 0.440 |
| 70.0 | 0.41 | 1.374 | 1.330 | 3.202 | 1.367 | 0.509 | 1.367 | 0.509 |
| 75.0 | 0.44 | 1.381 | 1.337 | 3.186 | 1.376 | 0.362 | 1.376 | 0.362 |
| 80.0 | 0.47 | 1.387 | 1.344 | 3.100 | 1.383 | 0.288 | 1.383 | 0.288 |
| 85.0 | 0.49 | 1.394 | 1.350 | 3.156 | 1.390 | 0.287 | 1.390 | 0.287 |
| 90.0 | 0.52 | 1.400 | 1.356 | 3.143 | 1.397 | 0.214 | 1.397 | 0.214 |
| 95.0 | 0.55 | 1.406 | 1.362 | 3.129 | 1.403 | 0.213 | 1.403 | 0.213 |
| 100.0 | 0.58 | 1.413 | 1.367 | 3.255 | 1.409 | 0.283 | 1.409 | 0.283 |
| 105.0 | 0.61 | 1.419 | 1.372 | 3.312 | 1.415 | 0.282 | 1.415 | 0.282 |
| 110.0 | 0.64 | 1.422 | 1.376 | 3.235 | 1.420 | 0.141 | 1.420 | 0.141 |
| 115.0 | 0.67 | 1.429 | 1.381 | 3.359 | 1.425 | 0.280 | 1.425 | 0.280 |
| 120.0 | 0.70 | 1.432 | 1.385 | 3.282 | 1.430 | 0.140 | 1.430 | 0.140 |
| 125.0 | 0.73 | 1.435 | 1.389 | 3.206 | 1.434 | 0.070 | 1.434 | 0.070 |
| 130.0 | 0.76 | 1.442 | 1.393 | 3.398 | 1.439 | 0.208 | 1.439 | 0.208 |
| 135.0 | 0.79 | 1.445 | 1.397 | 3.322 | 1.443 | 0.138 | 1.443 | 0.138 |
| 140.0 | 0.81 | 1.448 | 1.401 | 3.246 | 1.447 | 0.069 | 1.447 | 0.069 |
| 145.0 | 0.84 | 1.451 | 1.404 | 3.239 | 1.451 | 0.000 | 1.451 | 0.000 |
| 150.0 | 0.87 | 1.454 | 1.407 | 3.232 | 1.455 | 0.069 | 1.455 | 0.069 |
| 155.0 | 0.90 | 1.461 | 1.411 | 3.422 | 1.458 | 0.205 | 1.458 | 0.205 |
| 160.0 | 0.93 | 1.464 | 1.414 | 3.415 | 1.462 | 0.137 | 1.462 | 0.137 |
| 165.0 | 0.96 | 1.467 | 1.417 | 3.408 | 1.465 | 0.136 | 1.465 | 0.136 |

**Table 1b.** Key properties of the pair correlation function resulting from Langevin dynamics simulations and three integral theory approaches: the hypernetted-chain approximation (HNC), isomorph-based empirically modified hypernetted-chain approximation (IEMHNC) and empirically modified hypernetted-chain approximation (EMHNC). The absolute relative deviation $\epsilon_{\mathrm{r}}$ between the theoretical and the simulation results is also reported. **Results for the magnitude of the first maximum in the case of $\boldsymbol{\kappa = 0}$**. The LD results are adopted from Table 4 of *T. Ott and M. Bonitz, Contrib. Plasma Phys.* **55**, *243 (2015)*. It should be pointed out that for the OCP, the IEMHNC and the EMHNC approaches are identical.

| $\Gamma$ | $\Gamma/\Gamma_{\mathrm{m}}$ | $g_{\mathrm{max1}}^{\mathrm{LD}}$ | $g_{\mathrm{max1}}^{\mathrm{HNC}}$ | $\epsilon_{\mathrm{HNC}}(\%)$ | $g_{\mathrm{max1}}^{\mathrm{IEMHNC}}$ | $\epsilon_{\mathrm{IEMHNC}}(\%)$ | $g_{\mathrm{max1}}^{\mathrm{EMHNC}}$ | $\epsilon_{\mathrm{EMHNC}}(\%)$ |
|---|---|---|---|---|---|---|---|---|
| 15.0 | 0.09 | 1.228 | 1.173 | 4.458 | 1.200 | 2.269 | 1.200 | 2.269 |
| 20.0 | 0.12 | 1.307 | 1.234 | 5.618 | 1.277 | 2.330 | 1.277 | 2.330 |
| 25.0 | 0.15 | 1.378 | 1.288 | 6.558 | 1.348 | 2.204 | 1.348 | 2.204 |
| 30.0 | 0.17 | 1.443 | 1.337 | 7.359 | 1.414 | 2.041 | 1.414 | 2.041 |
| 35.0 | 0.20 | 1.504 | 1.382 | 8.105 | 1.475 | 1.931 | 1.475 | 1.931 |
| 40.0 | 0.23 | 1.560 | 1.424 | 8.702 | 1.533 | 1.759 | 1.533 | 1.759 |
| 45.0 | 0.26 | 1.614 | 1.464 | 9.307 | 1.587 | 1.677 | 1.587 | 1.677 |
| 50.0 | 0.29 | 1.664 | 1.501 | 9.790 | 1.639 | 1.528 | 1.639 | 1.528 |
| 55.0 | 0.32 | 1.712 | 1.537 | 10.251 | 1.688 | 1.410 | 1.688 | 1.410 |
| 60.0 | 0.35 | 1.757 | 1.570 | 10.627 | 1.735 | 1.246 | 1.735 | 1.246 |
| 65.0 | 0.38 | 1.803 | 1.603 | 11.115 | 1.781 | 1.244 | 1.781 | 1.244 |
| 70.0 | 0.41 | 1.845 | 1.634 | 11.456 | 1.824 | 1.113 | 1.824 | 1.113 |
| 75.0 | 0.44 | 1.885 | 1.664 | 11.750 | 1.867 | 0.957 | 1.867 | 0.957 |
| 80.0 | 0.47 | 1.926 | 1.692 | 12.130 | 1.908 | 0.926 | 1.908 | 0.926 |
| 85.0 | 0.49 | 1.964 | 1.720 | 12.409 | 1.948 | 0.802 | 1.948 | 0.802 |
| 90.0 | 0.52 | 2.001 | 1.747 | 12.676 | 1.987 | 0.686 | 1.987 | 0.686 |
| 95.0 | 0.55 | 2.037 | 1.774 | 12.930 | 2.025 | 0.573 | 2.025 | 0.573 |
| 100.0 | 0.58 | 2.072 | 1.799 | 13.167 | 2.063 | 0.457 | 2.063 | 0.457 |
| 105.0 | 0.61 | 2.107 | 1.824 | 13.428 | 2.099 | 0.385 | 2.099 | 0.385 |
| 110.0 | 0.64 | 2.140 | 1.848 | 13.629 | 2.134 | 0.258 | 2.134 | 0.258 |
| 115.0 | 0.67 | 2.174 | 1.872 | 13.890 | 2.169 | 0.213 | 2.169 | 0.213 |
| 120.0 | 0.70 | 2.206 | 1.895 | 14.089 | 2.204 | 0.110 | 2.204 | 0.110 |
| 125.0 | 0.73 | 2.237 | 1.918 | 14.266 | 2.237 | 0.008 | 2.237 | 0.008 |
| 130.0 | 0.76 | 2.270 | 1.940 | 14.535 | 2.270 | 0.007 | 2.270 | 0.007 |
| 135.0 | 0.79 | 2.298 | 1.962 | 14.631 | 2.303 | 0.199 | 2.303 | 0.199 |
| 140.0 | 0.81 | 2.329 | 1.983 | 14.852 | 2.334 | 0.234 | 2.334 | 0.234 |
| 145.0 | 0.84 | 2.358 | 2.004 | 15.013 | 2.366 | 0.331 | 2.366 | 0.331 |
| 150.0 | 0.87 | 2.386 | 2.025 | 15.149 | 2.397 | 0.448 | 2.397 | 0.448 |
| 155.0 | 0.90 | 2.413 | 2.045 | 15.263 | 2.427 | 0.584 | 2.427 | 0.584 |
| 160.0 | 0.93 | 2.442 | 2.065 | 15.455 | 2.457 | 0.616 | 2.457 | 0.616 |
| 165.0 | 0.96 | 2.470 | 2.084 | 15.623 | 2.487 | 0.670 | 2.487 | 0.670 |

**Table 1c.** Key properties of the pair correlation function resulting from Langevin dynamics simulations and three integral theory approaches: the hypernetted-chain approximation (HNC), isomorph-based empirically modified hypernetted-chain approximation (IEMHNC) and empirically modified hypernetted-chain approximation (EMHNC). The absolute relative deviation $\epsilon_{\mathrm{r}}$ between the theoretical and the simulation results is also reported. **Results for the position of the first maximum in the case of $\boldsymbol{\kappa = 0}$**. The LD results are adopted from Table 4 of *T. Ott and M. Bonitz, Contrib. Plasma Phys.* **55**, *243 (2015)*. It should be pointed out that for the OCP, the IEMHNC and the EMHNC approaches are identical.

| $\Gamma$ | $\Gamma/\Gamma_{\mathrm{m}}$ | $r_{\mathrm{max1}}^{\mathrm{LD}}/d$ | $r_{\mathrm{max1}}^{\mathrm{HNC}}/d$ | $\epsilon_{\mathrm{HNC}}(\%)$ | $r_{\mathrm{max1}}^{\mathrm{IEMHNC}}/d$ | $\epsilon_{\mathrm{IEMHNC}}(\%)$ | $r_{\mathrm{max1}}^{\mathrm{EMHNC}}/d$ | $\epsilon_{\mathrm{EMHNC}}(\%)$ |
|---|---|---|---|---|---|---|---|---|
| 15.0 | 0.09 | 1.666 | 1.663 | 0.180 | 1.678 | 0.720 | 1.678 | 0.720 |
| 20.0 | 0.12 | 1.665 | 1.657 | 0.480 | 1.672 | 0.420 | 1.672 | 0.420 |
| 25.0 | 0.15 | 1.668 | 1.655 | 0.779 | 1.670 | 0.120 | 1.670 | 0.120 |
| 30.0 | 0.17 | 1.671 | 1.655 | 0.958 | 1.670 | 0.060 | 1.670 | 0.060 |
| 35.0 | 0.20 | 1.674 | 1.657 | 1.016 | 1.671 | 0.179 | 1.671 | 0.179 |
| 40.0 | 0.23 | 1.678 | 1.658 | 1.192 | 1.673 | 0.298 | 1.673 | 0.298 |
| 45.0 | 0.26 | 1.681 | 1.660 | 1.249 | 1.676 | 0.297 | 1.676 | 0.297 |
| 50.0 | 0.29 | 1.685 | 1.662 | 1.365 | 1.678 | 0.415 | 1.678 | 0.415 |
| 55.0 | 0.32 | 1.688 | 1.664 | 1.422 | 1.681 | 0.415 | 1.681 | 0.415 |
| 60.0 | 0.35 | 1.690 | 1.666 | 1.420 | 1.683 | 0.414 | 1.683 | 0.414 |
| 65.0 | 0.38 | 1.693 | 1.668 | 1.477 | 1.686 | 0.413 | 1.686 | 0.413 |
| 70.0 | 0.41 | 1.696 | 1.669 | 1.592 | 1.688 | 0.472 | 1.688 | 0.472 |
| 75.0 | 0.44 | 1.698 | 1.671 | 1.590 | 1.690 | 0.471 | 1.690 | 0.471 |
| 80.0 | 0.47 | 1.701 | 1.673 | 1.646 | 1.693 | 0.470 | 1.693 | 0.470 |
| 85.0 | 0.49 | 1.703 | 1.675 | 1.644 | 1.695 | 0.470 | 1.695 | 0.470 |
| 90.0 | 0.52 | 1.705 | 1.676 | 1.701 | 1.697 | 0.469 | 1.697 | 0.469 |
| 95.0 | 0.55 | 1.707 | 1.678 | 1.699 | 1.699 | 0.469 | 1.699 | 0.469 |
| 100.0 | 0.58 | 1.709 | 1.679 | 1.755 | 1.701 | 0.468 | 1.701 | 0.468 |
| 105.0 | 0.61 | 1.710 | 1.681 | 1.696 | 1.703 | 0.409 | 1.703 | 0.409 |
| 110.0 | 0.64 | 1.712 | 1.682 | 1.752 | 1.705 | 0.409 | 1.705 | 0.409 |
| 115.0 | 0.67 | 1.714 | 1.683 | 1.809 | 1.707 | 0.408 | 1.707 | 0.408 |
| 120.0 | 0.70 | 1.715 | 1.685 | 1.749 | 1.708 | 0.408 | 1.708 | 0.408 |
| 125.0 | 0.73 | 1.717 | 1.686 | 1.805 | 1.710 | 0.408 | 1.710 | 0.408 |
| 130.0 | 0.76 | 1.719 | 1.687 | 1.862 | 1.712 | 0.407 | 1.712 | 0.407 |
| 135.0 | 0.79 | 1.720 | 1.688 | 1.860 | 1.713 | 0.407 | 1.713 | 0.407 |
| 140.0 | 0.81 | 1.721 | 1.690 | 1.801 | 1.715 | 0.349 | 1.715 | 0.349 |
| 145.0 | 0.84 | 1.723 | 1.691 | 1.857 | 1.716 | 0.406 | 1.716 | 0.406 |
| 150.0 | 0.87 | 1.724 | 1.692 | 1.856 | 1.718 | 0.348 | 1.718 | 0.348 |
| 155.0 | 0.90 | 1.725 | 1.693 | 1.855 | 1.719 | 0.348 | 1.719 | 0.348 |
| 160.0 | 0.93 | 1.727 | 1.694 | 1.911 | 1.721 | 0.347 | 1.721 | 0.347 |
| 165.0 | 0.96 | 1.728 | 1.695 | 1.910 | 1.722 | 0.347 | 1.722 | 0.347 |

**Table 1d.** Key properties of the pair correlation function resulting from Langevin dynamics simulations and three integral theory approaches: the hypernetted-chain approximation (HNC), isomorph-based empirically modified hypernetted-chain approximation (IEMHNC) and empirically modified hypernetted-chain approximation (EMHNC). The absolute relative deviation $\epsilon_{\mathrm{r}}$ between the theoretical and the simulation results is also reported. **Results for the magnitude of the first minimum in the case of $\boldsymbol{\kappa = 0}$**. The LD results are adopted from Table 4 of *T. Ott and M. Bonitz, Contrib. Plasma Phys.* **55**, *243 (2015)*. It should be pointed out that for the OCP, the IEMHNC and the EMHNC approaches are identical.

| $\Gamma$ | $\Gamma/\Gamma_{\mathrm{m}}$ | $g_{\mathrm{min1}}^{\mathrm{LD}}$ | $g_{\mathrm{min1}}^{\mathrm{HNC}}$ | $\epsilon_{\mathrm{HNC}}(\%)$ | $g_{\mathrm{min1}}^{\mathrm{IEMHNC}}$ | $\epsilon_{\mathrm{IEMHNC}}(\%)$ | $g_{\mathrm{min1}}^{\mathrm{EMHNC}}$ | $\epsilon_{\mathrm{EMHNC}}(\%)$ |
|---|---|---|---|---|---|---|---|---|
| 15.0 | 0.09 | 0.952 | 0.971 | 1.956 | 0.959 | 0.743 | 0.959 | 0.743 |
| 20.0 | 0.12 | 0.925 | 0.953 | 3.038 | 0.935 | 1.092 | 0.935 | 1.092 |
| 25.0 | 0.15 | 0.899 | 0.936 | 4.107 | 0.912 | 1.397 | 0.912 | 1.397 |
| 30.0 | 0.17 | 0.876 | 0.920 | 4.976 | 0.889 | 1.521 | 0.889 | 1.521 |
| 35.0 | 0.20 | 0.853 | 0.904 | 6.008 | 0.869 | 1.837 | 0.869 | 1.837 |
| 40.0 | 0.23 | 0.833 | 0.890 | 6.831 | 0.850 | 1.987 | 0.850 | 1.987 |
| 45.0 | 0.26 | 0.814 | 0.877 | 7.678 | 0.832 | 2.192 | 0.832 | 2.192 |
| 50.0 | 0.29 | 0.796 | 0.864 | 8.538 | 0.815 | 2.434 | 0.815 | 2.434 |
| 55.0 | 0.32 | 0.780 | 0.852 | 9.258 | 0.800 | 2.565 | 0.800 | 2.565 |
| 60.0 | 0.35 | 0.765 | 0.841 | 9.957 | 0.786 | 2.691 | 0.786 | 2.691 |
| 65.0 | 0.38 | 0.750 | 0.831 | 10.770 | 0.772 | 2.935 | 0.772 | 2.935 |
| 70.0 | 0.41 | 0.737 | 0.821 | 11.391 | 0.759 | 3.008 | 0.759 | 3.008 |
| 75.0 | 0.44 | 0.724 | 0.812 | 12.106 | 0.747 | 3.173 | 0.747 | 3.173 |
| 80.0 | 0.47 | 0.711 | 0.803 | 12.913 | 0.735 | 3.426 | 0.735 | 3.426 |
| 85.0 | 0.49 | 0.700 | 0.794 | 13.487 | 0.724 | 3.466 | 0.724 | 3.466 |
| 90.0 | 0.52 | 0.689 | 0.786 | 14.135 | 0.714 | 3.576 | 0.714 | 3.576 |
| 95.0 | 0.55 | 0.678 | 0.779 | 14.857 | 0.703 | 3.751 | 0.703 | 3.751 |
| 100.0 | 0.58 | 0.668 | 0.771 | 15.478 | 0.694 | 3.835 | 0.694 | 3.835 |
| 105.0 | 0.61 | 0.658 | 0.764 | 16.163 | 0.684 | 3.975 | 0.684 | 3.975 |
| 110.0 | 0.64 | 0.648 | 0.758 | 16.912 | 0.675 | 4.169 | 0.675 | 4.169 |
| 115.0 | 0.67 | 0.639 | 0.751 | 17.539 | 0.666 | 4.253 | 0.666 | 4.253 |
| 120.0 | 0.70 | 0.630 | 0.745 | 18.222 | 0.658 | 4.384 | 0.658 | 4.384 |
| 125.0 | 0.73 | 0.621 | 0.739 | 18.960 | 0.649 | 4.561 | 0.649 | 4.561 |
| 130.0 | 0.76 | 0.613 | 0.733 | 19.557 | 0.641 | 4.612 | 0.641 | 4.612 |
| 135.0 | 0.79 | 0.605 | 0.727 | 20.202 | 0.633 | 4.701 | 0.633 | 4.701 |
| 140.0 | 0.81 | 0.596 | 0.722 | 21.096 | 0.626 | 5.005 | 0.626 | 5.005 |
| 145.0 | 0.84 | 0.588 | 0.716 | 21.838 | 0.618 | 5.173 | 0.618 | 5.173 |
| 150.0 | 0.87 | 0.581 | 0.711 | 22.418 | 0.611 | 5.197 | 0.611 | 5.197 |
| 155.0 | 0.90 | 0.574 | 0.706 | 23.037 | 0.604 | 5.253 | 0.604 | 5.253 |
| 160.0 | 0.93 | 0.567 | 0.701 | 23.694 | 0.597 | 5.340 | 0.597 | 5.340 |
| 165.0 | 0.96 | 0.560 | 0.697 | 24.392 | 0.591 | 5.459 | 0.591 | 5.459 |

**Table 1e.** Key properties of the pair correlation function resulting from Langevin dynamics simulations and three integral theory approaches: the hypernetted-chain approximation (HNC), isomorph-based empirically modified hypernetted-chain approximation (IEMHNC) and empirically modified hypernetted-chain approximation (EMHNC). The absolute relative deviation $\epsilon_{\mathrm{r}}$ between the theoretical and the simulation results is also reported. **Results for the position of the first minimum in the case of $\boldsymbol{\kappa = 0}$**. The LD results are adopted from Table 4 of *T. Ott and M. Bonitz, Contrib. Plasma Phys.* **55**, *243 (2015)*. It should be pointed out that for the OCP, the IEMHNC and the EMHNC approaches are identical.

| $\Gamma$ | $\Gamma/\Gamma_{\mathrm{m}}$ | $r_{\mathrm{min1}}^{\mathrm{LD}}/d$ | $r_{\mathrm{min1}}^{\mathrm{HNC}}/d$ | $\epsilon_{\mathrm{HNC}}(\%)$ | $r_{\mathrm{min1}}^{\mathrm{IEMHNC}}/d$ | $\epsilon_{\mathrm{IEMHNC}}(\%)$ | $r_{\mathrm{min1}}^{\mathrm{EMHNC}}/d$ | $\epsilon_{\mathrm{EMHNC}}(\%)$ |
|---|---|---|---|---|---|---|---|---|
| 15.0 | 0.09 | 2.489 | 2.540 | 2.049 | 2.538 | 1.969 | 2.538 | 1.969 |
| 20.0 | 0.12 | 2.472 | 2.514 | 1.699 | 2.510 | 1.537 | 2.510 | 1.537 |
| 25.0 | 0.15 | 2.467 | 2.502 | 1.419 | 2.494 | 1.094 | 2.494 | 1.094 |
| 30.0 | 0.17 | 2.463 | 2.496 | 1.340 | 2.485 | 0.893 | 2.485 | 0.893 |
| 35.0 | 0.20 | 2.461 | 2.492 | 1.260 | 2.480 | 0.772 | 2.480 | 0.772 |
| 40.0 | 0.23 | 2.461 | 2.490 | 1.178 | 2.476 | 0.610 | 2.476 | 0.610 |
| 45.0 | 0.26 | 2.459 | 2.489 | 1.220 | 2.473 | 0.569 | 2.473 | 0.569 |
| 50.0 | 0.29 | 2.459 | 2.488 | 1.179 | 2.471 | 0.488 | 2.471 | 0.488 |
| 55.0 | 0.32 | 2.456 | 2.487 | 1.262 | 2.468 | 0.489 | 2.468 | 0.489 |
| 60.0 | 0.35 | 2.455 | 2.486 | 1.263 | 2.466 | 0.448 | 2.466 | 0.448 |
| 65.0 | 0.38 | 2.454 | 2.486 | 1.304 | 2.464 | 0.407 | 2.464 | 0.407 |
| 70.0 | 0.41 | 2.453 | 2.485 | 1.305 | 2.462 | 0.367 | 2.462 | 0.367 |
| 75.0 | 0.44 | 2.451 | 2.484 | 1.346 | 2.459 | 0.326 | 2.459 | 0.326 |
| 80.0 | 0.47 | 2.449 | 2.484 | 1.429 | 2.457 | 0.327 | 2.457 | 0.327 |
| 85.0 | 0.49 | 2.448 | 2.483 | 1.430 | 2.455 | 0.286 | 2.455 | 0.286 |
| 90.0 | 0.52 | 2.446 | 2.482 | 1.472 | 2.453 | 0.286 | 2.453 | 0.286 |
| 95.0 | 0.55 | 2.443 | 2.481 | 1.555 | 2.450 | 0.287 | 2.450 | 0.287 |
| 100.0 | 0.58 | 2.441 | 2.480 | 1.598 | 2.448 | 0.287 | 2.448 | 0.287 |
| 105.0 | 0.61 | 2.439 | 2.479 | 1.640 | 2.446 | 0.287 | 2.446 | 0.287 |
| 110.0 | 0.64 | 2.439 | 2.478 | 1.599 | 2.444 | 0.205 | 2.444 | 0.205 |
| 115.0 | 0.67 | 2.437 | 2.476 | 1.600 | 2.442 | 0.205 | 2.442 | 0.205 |
| 120.0 | 0.70 | 2.435 | 2.475 | 1.643 | 2.440 | 0.205 | 2.440 | 0.205 |
| 125.0 | 0.73 | 2.434 | 2.474 | 1.643 | 2.438 | 0.164 | 2.438 | 0.164 |
| 130.0 | 0.76 | 2.432 | 2.473 | 1.686 | 2.436 | 0.164 | 2.436 | 0.164 |
| 135.0 | 0.79 | 2.431 | 2.472 | 1.687 | 2.434 | 0.123 | 2.434 | 0.123 |
| 140.0 | 0.81 | 2.428 | 2.471 | 1.771 | 2.432 | 0.165 | 2.432 | 0.165 |
| 145.0 | 0.84 | 2.428 | 2.469 | 1.689 | 2.430 | 0.082 | 2.430 | 0.082 |
| 150.0 | 0.87 | 2.426 | 2.468 | 1.731 | 2.429 | 0.124 | 2.429 | 0.124 |
| 155.0 | 0.90 | 2.425 | 2.467 | 1.732 | 2.427 | 0.082 | 2.427 | 0.082 |
| 160.0 | 0.93 | 2.424 | 2.466 | 1.733 | 2.425 | 0.041 | 2.425 | 0.041 |
| 165.0 | 0.96 | 2.423 | 2.465 | 1.733 | 2.424 | 0.041 | 2.424 | 0.041 |

**Table 1f.** Key properties of the pair correlation function resulting from Langevin dynamics simulations and three integral theory approaches: the hypernetted-chain approximation (HNC), isomorph-based empirically modified hypernetted-chain approximation (IEMHNC) and empirically modified hypernetted-chain approximation (EMHNC). The absolute relative deviation $\epsilon_{\mathrm{r}}$ between the theoretical and the simulation results is reported. **Results for the magnitude of the second maximum in the case of $\boldsymbol{\kappa = 0}$**. The LD results are adopted from Table 4 of *T. Ott and M. Bonitz, Contrib. Plasma Phys.* **55**, *243 (2015)*. It should be pointed out that for the OCP, the IEMHNC and the EMHNC approaches are identical.

| $\Gamma$ | $\Gamma/\Gamma_{\mathrm{m}}$ | $g_{\mathrm{max2}}^{\mathrm{LD}}$ | $g_{\mathrm{max2}}^{\mathrm{HNC}}$ | $\epsilon_{\mathrm{HNC}}(\%)$ | $g_{\mathrm{max2}}^{\mathrm{IEMHNC}}$ | $\epsilon_{\mathrm{IEMHNC}}(\%)$ | $g_{\mathrm{max2}}^{\mathrm{EMHNC}}$ | $\epsilon_{\mathrm{EMHNC}}(\%)$ |
|---|---|---|---|---|---|---|---|---|
| 15.0 | 0.09 | 1.012 | 1.006 | 0.594 | 1.010 | 0.189 | 1.010 | 0.189 |
| 20.0 | 0.12 | 1.023 | 1.012 | 1.106 | 1.019 | 0.369 | 1.019 | 0.369 |
| 25.0 | 0.15 | 1.035 | 1.018 | 1.609 | 1.030 | 0.493 | 1.030 | 0.493 |
| 30.0 | 0.17 | 1.047 | 1.026 | 2.047 | 1.042 | 0.523 | 1.042 | 0.523 |
| 35.0 | 0.20 | 1.060 | 1.033 | 2.536 | 1.054 | 0.597 | 1.054 | 0.597 |
| 40.0 | 0.23 | 1.073 | 1.041 | 2.997 | 1.066 | 0.645 | 1.066 | 0.645 |
| 45.0 | 0.26 | 1.085 | 1.049 | 3.351 | 1.079 | 0.590 | 1.079 | 0.590 |
| 50.0 | 0.29 | 1.098 | 1.056 | 3.783 | 1.091 | 0.627 | 1.091 | 0.627 |
| 55.0 | 0.32 | 1.110 | 1.064 | 4.121 | 1.104 | 0.580 | 1.104 | 0.580 |
| 60.0 | 0.35 | 1.122 | 1.072 | 4.456 | 1.116 | 0.542 | 1.116 | 0.542 |
| 65.0 | 0.38 | 1.133 | 1.080 | 4.707 | 1.128 | 0.429 | 1.128 | 0.429 |
| 70.0 | 0.41 | 1.145 | 1.087 | 5.043 | 1.140 | 0.419 | 1.140 | 0.419 |
| 75.0 | 0.44 | 1.156 | 1.095 | 5.299 | 1.152 | 0.338 | 1.152 | 0.338 |
| 80.0 | 0.47 | 1.166 | 1.102 | 5.478 | 1.164 | 0.188 | 1.164 | 0.188 |
| 85.0 | 0.49 | 1.176 | 1.109 | 5.662 | 1.175 | 0.056 | 1.175 | 0.056 |
| 90.0 | 0.52 | 1.186 | 1.117 | 5.853 | 1.187 | 0.057 | 1.187 | 0.057 |
| 95.0 | 0.55 | 1.196 | 1.124 | 6.048 | 1.198 | 0.152 | 1.198 | 0.152 |
| 100.0 | 0.58 | 1.205 | 1.131 | 6.172 | 1.209 | 0.311 | 1.209 | 0.311 |
| 105.0 | 0.61 | 1.213 | 1.137 | 6.226 | 1.219 | 0.535 | 1.219 | 0.535 |
| 110.0 | 0.64 | 1.222 | 1.144 | 6.364 | 1.230 | 0.658 | 1.230 | 0.658 |
| 115.0 | 0.67 | 1.231 | 1.151 | 6.509 | 1.240 | 0.761 | 1.240 | 0.761 |
| 120.0 | 0.70 | 1.238 | 1.157 | 6.509 | 1.251 | 1.011 | 1.251 | 1.011 |
| 125.0 | 0.73 | 1.246 | 1.164 | 6.592 | 1.260 | 1.159 | 1.260 | 1.159 |
| 130.0 | 0.76 | 1.253 | 1.170 | 6.608 | 1.270 | 1.371 | 1.270 | 1.371 |
| 135.0 | 0.79 | 1.260 | 1.176 | 6.632 | 1.280 | 1.565 | 1.280 | 1.565 |
| 140.0 | 0.81 | 1.267 | 1.183 | 6.662 | 1.289 | 1.741 | 1.289 | 1.741 |
| 145.0 | 0.84 | 1.273 | 1.189 | 6.627 | 1.298 | 1.980 | 1.298 | 1.980 |
| 150.0 | 0.87 | 1.279 | 1.195 | 6.599 | 1.307 | 2.202 | 1.307 | 2.202 |
| 155.0 | 0.90 | 1.285 | 1.200 | 6.579 | 1.316 | 2.407 | 1.316 | 2.407 |
| 160.0 | 0.93 | 1.291 | 1.206 | 6.566 | 1.324 | 2.594 | 1.324 | 2.594 |
| 165.0 | 0.96 | 1.297 | 1.212 | 6.559 | 1.333 | 2.766 | 1.333 | 2.766 |

**Table 1g.** Key properties of the pair correlation function resulting from Langevin dynamics simulations and three integral theory approaches: the hypernetted-chain approximation (HNC), isomorph-based empirically modified hypernetted-chain approximation (IEMHNC) and empirically modified hypernetted-chain approximation (EMHNC). The absolute relative deviation $\epsilon_{\mathrm{r}}$ between the theoretical and the simulation results is also reported. **Results for the position of the second maximum in the case of $\boldsymbol{\kappa = 0}$**. The LD results are adopted from Table 4 of *T. Ott and M. Bonitz, Contrib. Plasma Phys.* **55**, *243 (2015)*. It should be pointed out that for the OCP, the IEMHNC and the EMHNC approaches are identical.

| $\Gamma$ | $\Gamma/\Gamma_{\mathrm{m}}$ | $r_{\mathrm{max2}}^{\mathrm{LD}}/d$ | $r_{\mathrm{max2}}^{\mathrm{HNC}}/d$ | $\epsilon_{\mathrm{HNC}}(\%)$ | $r_{\mathrm{max2}}^{\mathrm{IEMHNC}}/d$ | $\epsilon_{\mathrm{IEMHNC}}(\%)$ | $r_{\mathrm{max2}}^{\mathrm{EMHNC}}/d$ | $\epsilon_{\mathrm{EMHNC}}(\%)$ |
|---|---|---|---|---|---|---|---|---|
| 15.0 | 0.09 | 3.298 | 3.402 | 3.153 | 3.384 | 2.608 | 3.384 | 2.608 |
| 20.0 | 0.12 | 3.278 | 3.350 | 2.196 | 3.332 | 1.647 | 3.332 | 1.647 |
| 25.0 | 0.15 | 3.259 | 3.322 | 1.933 | 3.300 | 1.258 | 3.300 | 1.258 |
| 30.0 | 0.17 | 3.248 | 3.304 | 1.724 | 3.280 | 0.985 | 3.280 | 0.985 |
| 35.0 | 0.20 | 3.244 | 3.292 | 1.480 | 3.267 | 0.709 | 3.267 | 0.709 |
| 40.0 | 0.23 | 3.240 | 3.283 | 1.327 | 3.259 | 0.586 | 3.259 | 0.586 |
| 45.0 | 0.26 | 3.238 | 3.277 | 1.204 | 3.253 | 0.463 | 3.253 | 0.463 |
| 50.0 | 0.29 | 3.236 | 3.272 | 1.112 | 3.249 | 0.402 | 3.249 | 0.402 |
| 55.0 | 0.32 | 3.235 | 3.268 | 1.020 | 3.247 | 0.371 | 3.247 | 0.371 |
| 60.0 | 0.35 | 3.233 | 3.265 | 0.990 | 3.245 | 0.371 | 3.245 | 0.371 |
| 65.0 | 0.38 | 3.234 | 3.263 | 0.897 | 3.244 | 0.309 | 3.244 | 0.309 |
| 70.0 | 0.41 | 3.231 | 3.261 | 0.929 | 3.243 | 0.371 | 3.243 | 0.371 |
| 75.0 | 0.44 | 3.232 | 3.259 | 0.835 | 3.243 | 0.340 | 3.243 | 0.340 |
| 80.0 | 0.47 | 3.232 | 3.258 | 0.804 | 3.243 | 0.340 | 3.243 | 0.340 |
| 85.0 | 0.49 | 3.233 | 3.257 | 0.742 | 3.243 | 0.309 | 3.243 | 0.309 |
| 90.0 | 0.52 | 3.234 | 3.256 | 0.680 | 3.244 | 0.309 | 3.244 | 0.309 |
| 95.0 | 0.55 | 3.232 | 3.255 | 0.712 | 3.244 | 0.371 | 3.244 | 0.371 |
| 100.0 | 0.58 | 3.232 | 3.255 | 0.712 | 3.245 | 0.402 | 3.245 | 0.402 |
| 105.0 | 0.61 | 3.233 | 3.254 | 0.650 | 3.246 | 0.402 | 3.246 | 0.402 |
| 110.0 | 0.64 | 3.233 | 3.254 | 0.650 | 3.246 | 0.402 | 3.246 | 0.402 |
| 115.0 | 0.67 | 3.233 | 3.254 | 0.650 | 3.247 | 0.433 | 3.247 | 0.433 |
| 120.0 | 0.70 | 3.234 | 3.254 | 0.618 | 3.248 | 0.433 | 3.248 | 0.433 |
| 125.0 | 0.73 | 3.233 | 3.254 | 0.650 | 3.249 | 0.495 | 3.249 | 0.495 |
| 130.0 | 0.76 | 3.233 | 3.254 | 0.650 | 3.250 | 0.526 | 3.250 | 0.526 |
| 135.0 | 0.79 | 3.235 | 3.254 | 0.587 | 3.251 | 0.495 | 3.251 | 0.495 |
| 140.0 | 0.81 | 3.234 | 3.254 | 0.618 | 3.252 | 0.557 | 3.252 | 0.557 |
| 145.0 | 0.84 | 3.235 | 3.254 | 0.587 | 3.253 | 0.556 | 3.253 | 0.556 |
| 150.0 | 0.87 | 3.235 | 3.254 | 0.587 | 3.254 | 0.587 | 3.254 | 0.587 |
| 155.0 | 0.90 | 3.235 | 3.255 | 0.618 | 3.255 | 0.618 | 3.255 | 0.618 |
| 160.0 | 0.93 | 3.235 | 3.255 | 0.618 | 3.256 | 0.649 | 3.256 | 0.649 |
| 165.0 | 0.96 | 3.234 | 3.255 | 0.649 | 3.257 | 0.711 | 3.257 | 0.711 |

**Table 2a.** Key properties of the pair correlation function resulting from Langevin dynamics simulations and three integral theory approaches: the hypernetted-chain approximation (HNC), isomorph-based empirically modified hypernetted-chain approximation (IEMHNC) and empirically modified hypernetted-chain approximation (EMHNC). The absolute relative deviation $\epsilon_{\mathrm{r}}$ between the theoretical and the simulation results is also reported. **Results for $\arg_r\{g(r) = 0.5\}$ in the case of $\kappa = 1$**. The LD results are adopted from Table 5 of *T. Ott and M. Bonitz, Contrib. Plasma Phys.* **55**, *243 (2015).*

| $\Gamma$ | $\Gamma/\Gamma_{\mathrm{m}}$ | $\Gamma_{\mathrm{iso}}^{\mathrm{OCP}}$ | $r_{\mathrm{cv}}^{\mathrm{LD}}/d$ | $r_{\mathrm{cv}}^{\mathrm{HNC}}/d$ | $\epsilon_{\mathrm{HNC}}(\%)$ | $r_{\mathrm{cv}}^{\mathrm{IEMHNC}}/d$ | $\epsilon_{\mathrm{IEMHNC}}(\%)$ | $r_{\mathrm{cv}}^{\mathrm{EMHNC}}/d$ | $\epsilon_{\mathrm{EMHNC}}(\%)$ |
|---|---|---|---|---|---|---|---|---|---|
| 10.0 | 0.05 | 7.80 | 1.076 | 1.054 | 2.045 | 1.057 | 1.766 | 1.062 | 1.301 |
| 15.0 | 0.07 | 11.70 | 1.139 | 1.113 | 2.283 | 1.124 | 1.317 | 1.128 | 0.966 |
| 20.0 | 0.09 | 15.61 | 1.177 | 1.152 | 2.124 | 1.168 | 0.765 | 1.172 | 0.425 |
| 25.0 | 0.11 | 19.51 | 1.211 | 1.181 | 2.477 | 1.200 | 0.908 | 1.204 | 0.578 |
| 30.0 | 0.14 | 23.41 | 1.237 | 1.204 | 2.668 | 1.226 | 0.889 | 1.230 | 0.566 |
| 35.0 | 0.16 | 27.31 | 1.254 | 1.223 | 2.472 | 1.247 | 0.558 | 1.251 | 0.239 |
| 40.0 | 0.18 | 31.21 | 1.275 | 1.239 | 2.824 | 1.265 | 0.784 | 1.269 | 0.471 |
| 45.0 | 0.21 | 35.11 | 1.288 | 1.253 | 2.717 | 1.281 | 0.543 | 1.284 | 0.311 |
| 50.0 | 0.23 | 39.01 | 1.301 | 1.265 | 2.767 | 1.295 | 0.461 | 1.298 | 0.231 |
| 55.0 | 0.25 | 42.91 | 1.313 | 1.276 | 2.818 | 1.307 | 0.457 | 1.310 | 0.228 |
| 60.0 | 0.28 | 46.82 | 1.326 | 1.286 | 3.017 | 1.318 | 0.603 | 1.321 | 0.377 |
| 65.0 | 0.30 | 50.72 | 1.334 | 1.295 | 2.924 | 1.328 | 0.450 | 1.331 | 0.225 |
| 70.0 | 0.32 | 54.62 | 1.343 | 1.303 | 2.978 | 1.337 | 0.447 | 1.340 | 0.223 |
| 75.0 | 0.34 | 58.52 | 1.351 | 1.311 | 2.961 | 1.346 | 0.370 | 1.348 | 0.222 |
| 80.0 | 0.37 | 62.42 | 1.360 | 1.318 | 3.088 | 1.354 | 0.441 | 1.356 | 0.294 |
| 85.0 | 0.39 | 66.32 | 1.364 | 1.324 | 2.933 | 1.361 | 0.220 | 1.364 | 0.000 |
| 90.0 | 0.41 | 70.22 | 1.373 | 1.330 | 3.132 | 1.368 | 0.364 | 1.370 | 0.218 |
| 95.0 | 0.44 | 74.12 | 1.377 | 1.336 | 2.977 | 1.374 | 0.218 | 1.377 | 0.000 |
| 100.0 | 0.46 | 78.03 | 1.385 | 1.342 | 3.105 | 1.381 | 0.289 | 1.383 | 0.144 |
| 105.0 | 0.48 | 81.93 | 1.390 | 1.347 | 3.094 | 1.386 | 0.288 | 1.389 | 0.072 |
| 110.0 | 0.51 | 85.83 | 1.394 | 1.352 | 3.013 | 1.392 | 0.143 | 1.394 | 0.000 |
| 115.0 | 0.53 | 89.73 | 1.402 | 1.356 | 3.281 | 1.397 | 0.357 | 1.399 | 0.214 |
| 120.0 | 0.55 | 93.63 | 1.407 | 1.361 | 3.269 | 1.402 | 0.355 | 1.404 | 0.213 |
| 125.0 | 0.57 | 97.53 | 1.411 | 1.365 | 3.260 | 1.407 | 0.283 | 1.409 | 0.142 |
| 130.0 | 0.60 | 101.43 | 1.415 | 1.369 | 3.251 | 1.411 | 0.283 | 1.414 | 0.071 |
| 135.0 | 0.62 | 105.33 | 1.419 | 1.373 | 3.242 | 1.416 | 0.211 | 1.418 | 0.070 |
| 140.0 | 0.64 | 109.24 | 1.424 | 1.377 | 3.301 | 1.420 | 0.281 | 1.422 | 0.140 |
| 145.0 | 0.67 | 113.14 | 1.428 | 1.381 | 3.291 | 1.424 | 0.280 | 1.426 | 0.140 |
| 150.0 | 0.69 | 117.04 | 1.428 | 1.384 | 3.081 | 1.428 | 0.000 | 1.430 | 0.140 |
| 155.0 | 0.71 | 120.94 | 1.432 | 1.387 | 3.142 | 1.431 | 0.070 | 1.434 | 0.140 |
| 160.0 | 0.74 | 124.84 | 1.436 | 1.391 | 3.134 | 1.435 | 0.070 | 1.438 | 0.139 |
| 165.0 | 0.76 | 128.74 | 1.441 | 1.394 | 3.262 | 1.438 | 0.208 | 1.441 | 0.000 |
| 170.0 | 0.78 | 132.64 | 1.445 | 1.397 | 3.322 | 1.442 | 0.208 | 1.444 | 0.069 |
| 175.0 | 0.80 | 136.54 | 1.445 | 1.400 | 3.114 | 1.445 | 0.000 | 1.448 | 0.208 |
| 180.0 | 0.83 | 140.45 | 1.449 | 1.402 | 3.244 | 1.448 | 0.069 | 1.451 | 0.138 |
| 185.0 | 0.85 | 144.35 | 1.453 | 1.405 | 3.304 | 1.451 | 0.138 | 1.454 | 0.069 |
| 190.0 | 0.87 | 148.25 | 1.453 | 1.408 | 3.097 | 1.454 | 0.069 | 1.457 | 0.275 |
| 195.0 | 0.90 | 152.15 | 1.458 | 1.410 | 3.292 | 1.457 | 0.069 | 1.460 | 0.137 |
| 200.0 | 0.92 | 156.05 | 1.462 | 1.413 | 3.352 | 1.460 | 0.137 | 1.463 | 0.068 |

**Table 2b.** Key properties of the pair correlation function resulting from Langevin dynamics simulations and three integral theory approaches: the hypernetted-chain approximation (HNC), isomorph-based empirically modified hypernetted-chain approximation (IEMHNC) and empirically modified hypernetted-chain approximation (EMHNC). The absolute relative deviation $\epsilon_{\mathrm{r}}$ between the theoretical and the simulation results is also reported. **Results for the magnitude of the first maximum in the case of $\boldsymbol{\kappa = 1}$**. The LD results are adopted from Table 5 of *T. Ott and M. Bonitz, Contrib. Plasma Phys.* **55**, *243 (2015)*.

| $\Gamma$ | $\Gamma/\Gamma_{\mathrm{m}}$ | $\Gamma_{\mathrm{iso}}^{\mathrm{OCP}}$ | $g_{\mathrm{max1}}^{\mathrm{LD}}$ | $g_{\mathrm{max1}}^{\mathrm{HNC}}$ | $\epsilon_{\mathrm{HNC}}(\%)$ | $g_{\mathrm{max1}}^{\mathrm{IEMHNC}}$ | $\epsilon_{\mathrm{IEMHNC}}(\%)$ | $g_{\mathrm{max1}}^{\mathrm{EMHNC}}$ | $\epsilon_{\mathrm{EMHNC}}(\%)$ |
|---|---|---|---|---|---|---|---|---|---|
| 10.0 | 0.05 | 7.80 | 1.101 | 1.079 | 1.989 | 1.084 | 1.575 | 1.089 | 1.062 |
| 15.0 | 0.07 | 11.70 | 1.175 | 1.137 | 3.198 | 1.154 | 1.805 | 1.159 | 1.347 |
| 20.0 | 0.09 | 15.61 | 1.243 | 1.190 | 4.248 | 1.217 | 2.074 | 1.225 | 1.416 |
| 25.0 | 0.11 | 19.51 | 1.304 | 1.238 | 5.058 | 1.278 | 2.029 | 1.288 | 1.264 |
| 30.0 | 0.14 | 23.41 | 1.360 | 1.282 | 5.745 | 1.335 | 1.872 | 1.345 | 1.071 |
| 35.0 | 0.16 | 27.31 | 1.413 | 1.322 | 6.412 | 1.388 | 1.754 | 1.400 | 0.949 |
| 40.0 | 0.18 | 31.21 | 1.462 | 1.360 | 6.960 | 1.439 | 1.582 | 1.450 | 0.787 |
| 45.0 | 0.21 | 35.11 | 1.509 | 1.396 | 7.502 | 1.487 | 1.469 | 1.499 | 0.687 |
| 50.0 | 0.23 | 39.01 | 1.553 | 1.429 | 7.957 | 1.532 | 1.323 | 1.544 | 0.553 |
| 55.0 | 0.25 | 42.91 | 1.595 | 1.461 | 8.378 | 1.576 | 1.190 | 1.588 | 0.431 |
| 60.0 | 0.28 | 46.82 | 1.636 | 1.492 | 8.810 | 1.618 | 1.114 | 1.630 | 0.363 |
| 65.0 | 0.30 | 50.72 | 1.675 | 1.521 | 9.190 | 1.658 | 1.019 | 1.670 | 0.273 |
| 70.0 | 0.32 | 54.62 | 1.711 | 1.549 | 9.461 | 1.697 | 0.837 | 1.709 | 0.093 |
| 75.0 | 0.34 | 58.52 | 1.749 | 1.576 | 9.882 | 1.734 | 0.849 | 1.747 | 0.107 |
| 80.0 | 0.37 | 62.42 | 1.783 | 1.602 | 10.137 | 1.770 | 0.702 | 1.784 | 0.042 |
| 85.0 | 0.39 | 66.32 | 1.817 | 1.628 | 10.428 | 1.806 | 0.617 | 1.819 | 0.129 |
| 90.0 | 0.41 | 70.22 | 1.850 | 1.652 | 10.702 | 1.840 | 0.533 | 1.854 | 0.217 |
| 95.0 | 0.44 | 74.12 | 1.882 | 1.676 | 10.956 | 1.874 | 0.444 | 1.888 | 0.311 |
| 100.0 | 0.46 | 78.03 | 1.914 | 1.699 | 11.236 | 1.906 | 0.400 | 1.921 | 0.360 |
| 105.0 | 0.48 | 81.93 | 1.944 | 1.721 | 11.447 | 1.938 | 0.293 | 1.953 | 0.474 |
| 110.0 | 0.51 | 85.83 | 1.974 | 1.743 | 11.679 | 1.970 | 0.223 | 1.985 | 0.550 |
| 115.0 | 0.53 | 89.73 | 2.003 | 1.765 | 11.886 | 2.000 | 0.138 | 2.016 | 0.643 |
| 120.0 | 0.55 | 93.63 | 2.031 | 1.786 | 12.068 | 2.030 | 0.035 | 2.046 | 0.754 |
| 125.0 | 0.57 | 97.53 | 2.058 | 1.806 | 12.225 | 2.060 | 0.087 | 2.076 | 0.884 |
| 130.0 | 0.60 | 101.43 | 2.088 | 1.826 | 12.524 | 2.089 | 0.037 | 2.106 | 0.841 |
| 135.0 | 0.62 | 105.33 | 2.114 | 1.846 | 12.669 | 2.117 | 0.154 | 2.134 | 0.967 |
| 140.0 | 0.64 | 109.24 | 2.141 | 1.865 | 12.868 | 2.145 | 0.200 | 2.163 | 1.020 |
| 145.0 | 0.67 | 113.14 | 2.166 | 1.884 | 12.999 | 2.173 | 0.316 | 2.191 | 1.144 |
| 150.0 | 0.69 | 117.04 | 2.191 | 1.903 | 13.142 | 2.200 | 0.410 | 2.218 | 1.247 |
| 155.0 | 0.71 | 120.94 | 2.217 | 1.921 | 13.336 | 2.227 | 0.439 | 2.245 | 1.283 |
| 160.0 | 0.74 | 124.84 | 2.242 | 1.939 | 13.501 | 2.253 | 0.495 | 2.272 | 1.346 |
| 165.0 | 0.76 | 128.74 | 2.266 | 1.957 | 13.637 | 2.279 | 0.577 | 2.299 | 1.436 |
| 170.0 | 0.78 | 132.64 | 2.289 | 1.974 | 13.744 | 2.305 | 0.687 | 2.325 | 1.553 |
| 175.0 | 0.80 | 136.54 | 2.314 | 1.992 | 13.936 | 2.330 | 0.692 | 2.350 | 1.564 |
| 180.0 | 0.83 | 140.45 | 2.337 | 2.008 | 14.060 | 2.355 | 0.769 | 2.376 | 1.648 |
| 185.0 | 0.85 | 144.35 | 2.359 | 2.025 | 14.157 | 2.380 | 0.875 | 2.401 | 1.760 |
| 190.0 | 0.87 | 148.25 | 2.383 | 2.041 | 14.333 | 2.404 | 0.881 | 2.425 | 1.771 |
| 195.0 | 0.90 | 152.15 | 2.404 | 2.058 | 14.408 | 2.428 | 1.000 | 2.450 | 1.897 |
| 200.0 | 0.92 | 156.05 | 2.427 | 2.074 | 14.562 | 2.452 | 1.022 | 2.474 | 1.924 |

**Table 2c.** Key properties of the pair correlation function resulting from Langevin dynamics simulations and three integral theory approaches: the hypernetted-chain approximation (HNC), isomorph-based empirically modified hypernetted-chain approximation (IEMHNC) and empirically modified hypernetted-chain approximation (EMHNC). The absolute relative deviation $\epsilon_{\mathrm{r}}$ between the theoretical and the simulation results is also reported. **Results for the position of the first maximum in the case of $\boldsymbol{\kappa = 1}$**. The LD results are adopted from Table 5 of *T. Ott and M. Bonitz, Contrib. Plasma Phys.* **55**, *243 (2015)*.

| $\Gamma$ | $\Gamma/\Gamma_{\mathrm{m}}$ | $\Gamma_{\mathrm{iso}}^{\mathrm{OCP}}$ | $r_{\mathrm{max1}}^{\mathrm{LD}}/d$ | $r_{\mathrm{max1}}^{\mathrm{HNC}}/d$ | $\epsilon_{\mathrm{HNC}}(\%)$ | $r_{\mathrm{max1}}^{\mathrm{IEMHNC}}/d$ | $\epsilon_{\mathrm{IEMHNC}}(\%)$ | $r_{\mathrm{max1}}^{\mathrm{EMHNC}}/d$ | $\epsilon_{\mathrm{EMHNC}}(\%)$ |
|---|---|---|---|---|---|---|---|---|---|
| 10.0 | 0.05 | 7.80 | 1.660 | 1.666 | 0.361 | 1.664 | 0.241 | 1.675 | 0.904 |
| 15.0 | 0.07 | 11.70 | 1.648 | 1.643 | 0.303 | 1.659 | 0.667 | 1.662 | 0.850 |
| 20.0 | 0.09 | 15.61 | 1.648 | 1.637 | 0.667 | 1.657 | 0.546 | 1.656 | 0.485 |
| 25.0 | 0.11 | 19.51 | 1.650 | 1.636 | 0.848 | 1.656 | 0.364 | 1.655 | 0.303 |
| 30.0 | 0.14 | 23.41 | 1.655 | 1.637 | 1.088 | 1.656 | 0.060 | 1.656 | 0.060 |
| 35.0 | 0.16 | 27.31 | 1.659 | 1.639 | 1.206 | 1.658 | 0.060 | 1.657 | 0.121 |
| 40.0 | 0.18 | 31.21 | 1.662 | 1.641 | 1.264 | 1.660 | 0.120 | 1.660 | 0.120 |
| 45.0 | 0.21 | 35.11 | 1.666 | 1.643 | 1.381 | 1.662 | 0.240 | 1.662 | 0.240 |
| 50.0 | 0.23 | 39.01 | 1.669 | 1.646 | 1.378 | 1.665 | 0.240 | 1.665 | 0.240 |
| 55.0 | 0.25 | 42.91 | 1.673 | 1.648 | 1.494 | 1.667 | 0.359 | 1.668 | 0.299 |
| 60.0 | 0.28 | 46.82 | 1.676 | 1.650 | 1.551 | 1.669 | 0.418 | 1.670 | 0.358 |
| 65.0 | 0.30 | 50.72 | 1.679 | 1.652 | 1.608 | 1.672 | 0.417 | 1.673 | 0.357 |
| 70.0 | 0.32 | 54.62 | 1.681 | 1.654 | 1.606 | 1.674 | 0.416 | 1.675 | 0.357 |
| 75.0 | 0.34 | 58.52 | 1.684 | 1.656 | 1.663 | 1.677 | 0.416 | 1.678 | 0.356 |
| 80.0 | 0.37 | 62.42 | 1.687 | 1.658 | 1.719 | 1.679 | 0.474 | 1.680 | 0.415 |
| 85.0 | 0.39 | 66.32 | 1.689 | 1.660 | 1.717 | 1.681 | 0.474 | 1.683 | 0.355 |
| 90.0 | 0.41 | 70.22 | 1.691 | 1.662 | 1.715 | 1.683 | 0.473 | 1.685 | 0.355 |
| 95.0 | 0.44 | 74.12 | 1.693 | 1.663 | 1.772 | 1.685 | 0.473 | 1.687 | 0.354 |
| 100.0 | 0.46 | 78.03 | 1.695 | 1.665 | 1.770 | 1.687 | 0.472 | 1.689 | 0.354 |
| 105.0 | 0.48 | 81.93 | 1.697 | 1.667 | 1.768 | 1.689 | 0.471 | 1.691 | 0.354 |
| 110.0 | 0.51 | 85.83 | 1.699 | 1.668 | 1.825 | 1.691 | 0.471 | 1.693 | 0.353 |
| 115.0 | 0.53 | 89.73 | 1.701 | 1.670 | 1.822 | 1.693 | 0.470 | 1.695 | 0.353 |
| 120.0 | 0.55 | 93.63 | 1.702 | 1.671 | 1.821 | 1.695 | 0.411 | 1.697 | 0.294 |
| 125.0 | 0.57 | 97.53 | 1.704 | 1.672 | 1.878 | 1.696 | 0.469 | 1.699 | 0.293 |
| 130.0 | 0.60 | 101.43 | 1.706 | 1.674 | 1.876 | 1.698 | 0.469 | 1.700 | 0.352 |
| 135.0 | 0.62 | 105.33 | 1.707 | 1.675 | 1.875 | 1.700 | 0.410 | 1.702 | 0.293 |
| 140.0 | 0.64 | 109.24 | 1.709 | 1.676 | 1.931 | 1.701 | 0.468 | 1.704 | 0.293 |
| 145.0 | 0.67 | 113.14 | 1.710 | 1.677 | 1.930 | 1.703 | 0.409 | 1.705 | 0.292 |
| 150.0 | 0.69 | 117.04 | 1.712 | 1.679 | 1.928 | 1.704 | 0.467 | 1.707 | 0.292 |
| 155.0 | 0.71 | 120.94 | 1.713 | 1.680 | 1.926 | 1.706 | 0.409 | 1.708 | 0.292 |
| 160.0 | 0.74 | 124.84 | 1.715 | 1.681 | 1.983 | 1.707 | 0.466 | 1.710 | 0.292 |
| 165.0 | 0.76 | 128.74 | 1.715 | 1.682 | 1.924 | 1.709 | 0.350 | 1.711 | 0.233 |
| 170.0 | 0.78 | 132.64 | 1.717 | 1.683 | 1.980 | 1.710 | 0.408 | 1.713 | 0.233 |
| 175.0 | 0.80 | 136.54 | 1.718 | 1.684 | 1.979 | 1.711 | 0.407 | 1.714 | 0.233 |
| 180.0 | 0.83 | 140.45 | 1.719 | 1.685 | 1.978 | 1.713 | 0.349 | 1.715 | 0.233 |
| 185.0 | 0.85 | 144.35 | 1.720 | 1.686 | 1.977 | 1.714 | 0.349 | 1.717 | 0.174 |
| 190.0 | 0.87 | 148.25 | 1.721 | 1.687 | 1.976 | 1.715 | 0.349 | 1.718 | 0.174 |
| 195.0 | 0.90 | 152.15 | 1.722 | 1.688 | 1.974 | 1.716 | 0.348 | 1.719 | 0.174 |
| 200.0 | 0.92 | 156.05 | 1.723 | 1.689 | 1.973 | 1.717 | 0.348 | 1.720 | 0.174 |

**Table 2d.** Key properties of the pair correlation function resulting from Langevin dynamics simulations and three integral theory approaches: the hypernetted-chain approximation (HNC), isomorph-based empirically modified hypernetted-chain approximation (IEMHNC) and empirically modified hypernetted-chain approximation (EMHNC). The absolute relative deviation $\epsilon_{\mathrm{r}}$ between the theoretical and the simulation results is also reported. **Results for the magnitude of the first minimum in the case of $\boldsymbol{\kappa = 1}$**. The LD results are adopted from Table 5 of *T. Ott and M. Bonitz, Contrib. Plasma Phys.* **55**, *243 (2015)*.

| $\Gamma$ | $\Gamma/\Gamma_{\mathrm{m}}$ | $\Gamma_{\mathrm{iso}}^{\mathrm{OCP}}$ | $g_{\mathrm{min1}}^{\mathrm{LD}}$ | $g_{\mathrm{min1}}^{\mathrm{HNC}}$ | $\epsilon_{\mathrm{HNC}}(\%)$ | $g_{\mathrm{min1}}^{\mathrm{IEMHNC}}$ | $\epsilon_{\mathrm{IEMHNC}}(\%)$ | $g_{\mathrm{min1}}^{\mathrm{EMHNC}}$ | $\epsilon_{\mathrm{EMHNC}}(\%)$ |
|---|---|---|---|---|---|---|---|---|---|
| 10.0 | 0.05 | 7.8 | 0.987 | 0.992 | 0.525 | 0.991 | 0.429 | 0.989 | 0.201 |
| 15.0 | 0.07 | 11.70 | 0.969 | 0.980 | 1.162 | 0.973 | 0.447 | 0.972 | 0.271 |
| 20.0 | 0.09 | 15.61 | 0.948 | 0.967 | 1.965 | 0.955 | 0.707 | 0.953 | 0.482 |
| 25.0 | 0.11 | 19.51 | 0.927 | 0.953 | 2.768 | 0.936 | 0.937 | 0.933 | 0.643 |
| 30.0 | 0.14 | 23.41 | 0.907 | 0.939 | 3.525 | 0.917 | 1.096 | 0.914 | 0.753 |
| 35.0 | 0.16 | 27.31 | 0.887 | 0.926 | 4.375 | 0.899 | 1.349 | 0.896 | 0.973 |
| 40.0 | 0.18 | 31.21 | 0.869 | 0.913 | 5.095 | 0.882 | 1.493 | 0.878 | 1.091 |
| 45.0 | 0.21 | 35.11 | 0.853 | 0.901 | 5.672 | 0.866 | 1.523 | 0.862 | 1.099 |
| 50.0 | 0.23 | 39.01 | 0.836 | 0.890 | 6.474 | 0.851 | 1.792 | 0.847 | 1.345 |
| 55.0 | 0.25 | 42.91 | 0.822 | 0.879 | 6.991 | 0.837 | 1.809 | 0.833 | 1.338 |
| 60.0 | 0.28 | 46.82 | 0.807 | 0.869 | 7.728 | 0.824 | 2.052 | 0.820 | 1.555 |
| 65.0 | 0.30 | 50.72 | 0.794 | 0.860 | 8.285 | 0.811 | 2.139 | 0.807 | 1.615 |
| 70.0 | 0.32 | 54.62 | 0.781 | 0.851 | 8.921 | 0.799 | 2.313 | 0.795 | 1.758 |
| 75.0 | 0.34 | 58.52 | 0.769 | 0.842 | 9.493 | 0.788 | 2.435 | 0.783 | 1.849 |
| 80.0 | 0.37 | 62.42 | 0.758 | 0.834 | 9.991 | 0.777 | 2.495 | 0.772 | 1.877 |
| 85.0 | 0.39 | 66.32 | 0.747 | 0.826 | 10.553 | 0.767 | 2.621 | 0.762 | 1.968 |
| 90.0 | 0.41 | 70.22 | 0.736 | 0.818 | 11.178 | 0.757 | 2.809 | 0.752 | 2.120 |
| 95.0 | 0.44 | 74.12 | 0.726 | 0.811 | 11.711 | 0.747 | 2.915 | 0.742 | 2.190 |
| 100.0 | 0.46 | 78.03 | 0.716 | 0.804 | 12.300 | 0.738 | 3.073 | 0.733 | 2.310 |
| 105.0 | 0.48 | 81.93 | 0.707 | 0.797 | 12.783 | 0.729 | 3.137 | 0.724 | 2.334 |
| 110.0 | 0.51 | 85.83 | 0.698 | 0.791 | 13.315 | 0.721 | 3.245 | 0.715 | 2.402 |
| 115.0 | 0.53 | 89.73 | 0.689 | 0.785 | 13.894 | 0.712 | 3.395 | 0.706 | 2.513 |
| 120.0 | 0.55 | 93.63 | 0.681 | 0.779 | 14.351 | 0.704 | 3.437 | 0.698 | 2.513 |
| 125.0 | 0.57 | 97.53 | 0.672 | 0.773 | 15.020 | 0.697 | 3.668 | 0.690 | 2.701 |
| 130.0 | 0.60 | 101.43 | 0.664 | 0.767 | 15.561 | 0.689 | 3.783 | 0.682 | 2.774 |
| 135.0 | 0.62 | 105.33 | 0.657 | 0.762 | 15.965 | 0.682 | 3.774 | 0.675 | 2.724 |
| 140.0 | 0.64 | 109.24 | 0.649 | 0.757 | 16.583 | 0.675 | 3.955 | 0.668 | 2.861 |
| 145.0 | 0.67 | 113.14 | 0.642 | 0.752 | 17.057 | 0.668 | 4.007 | 0.660 | 2.870 |
| 150.0 | 0.69 | 117.04 | 0.634 | 0.747 | 17.750 | 0.661 | 4.252 | 0.653 | 3.070 |
| 155.0 | 0.71 | 120.94 | 0.627 | 0.742 | 18.294 | 0.654 | 4.362 | 0.647 | 3.137 |
| 160.0 | 0.74 | 124.84 | 0.620 | 0.737 | 18.870 | 0.648 | 4.500 | 0.640 | 3.230 |
| 165.0 | 0.76 | 128.74 | 0.614 | 0.732 | 19.286 | 0.642 | 4.495 | 0.634 | 3.183 |
| 170.0 | 0.78 | 132.64 | 0.608 | 0.728 | 19.728 | 0.635 | 4.513 | 0.627 | 3.157 |
| 175.0 | 0.80 | 136.54 | 0.601 | 0.724 | 20.398 | 0.629 | 4.727 | 0.621 | 3.326 |
| 180.0 | 0.83 | 140.45 | 0.595 | 0.719 | 20.898 | 0.624 | 4.791 | 0.615 | 3.346 |
| 185.0 | 0.85 | 144.35 | 0.588 | 0.715 | 21.631 | 0.618 | 5.056 | 0.609 | 3.563 |
| 190.0 | 0.87 | 148.25 | 0.582 | 0.711 | 22.188 | 0.612 | 5.166 | 0.603 | 3.629 |
| 195.0 | 0.90 | 152.15 | 0.577 | 0.707 | 22.559 | 0.607 | 5.115 | 0.597 | 3.535 |
| 200.0 | 0.92 | 156.05 | 0.571 | 0.703 | 23.168 | 0.601 | 5.266 | 0.592 | 3.641 |

**Table 2e.** Key properties of the pair correlation function resulting from Langevin dynamics simulations and three integral theory approaches: the hypernetted-chain approximation (HNC), isomorph-based empirically modified hypernetted-chain approximation (IEMHNC) and empirically modified hypernetted-chain approximation (EMHNC). The absolute relative deviation $\epsilon_{\mathrm{r}}$ between the theoretical and the simulation results is also reported. **Results for the position of the first minimum in the case of $\boldsymbol{\kappa = 1}$**. The LD results are adopted from Table 5 of *T. Ott and M. Bonitz, Contrib. Plasma Phys.* **55**, *243 (2015)*.

| $\Gamma$ | $\Gamma/\Gamma_{\mathrm{m}}$ | $\Gamma_{\mathrm{iso}}^{\mathrm{OCP}}$ | $r_{\mathrm{min1}}^{\mathrm{LD}}/d$ | $r_{\mathrm{min1}}^{\mathrm{HNC}}/d$ | $\epsilon_{\mathrm{HNC}}(\%)$ | $r_{\mathrm{min1}}^{\mathrm{IEMHNC}}/d$ | $\epsilon_{\mathrm{IEMHNC}}(\%)$ | $r_{\mathrm{min1}}^{\mathrm{EMHNC}}/d$ | $\epsilon_{\mathrm{EMHNC}}(\%)$ |
|---|---|---|---|---|---|---|---|---|---|
| 10.0 | 0.05 | 7.80 | 2.520 | 2.594 | 2.937 | 2.576 | 2.222 | 2.574 | 2.143 |
| 15.0 | 0.07 | 11.70 | 2.482 | 2.523 | 1.652 | 2.526 | 1.773 | 2.529 | 1.894 |
| 20.0 | 0.09 | 15.61 | 2.464 | 2.495 | 1.258 | 2.505 | 1.664 | 2.499 | 1.420 |
| 25.0 | 0.11 | 19.51 | 2.457 | 2.483 | 1.058 | 2.489 | 1.302 | 2.482 | 1.018 |
| 30.0 | 0.14 | 23.41 | 2.454 | 2.477 | 0.937 | 2.479 | 1.019 | 2.473 | 0.774 |
| 35.0 | 0.16 | 27.31 | 2.452 | 2.474 | 0.897 | 2.473 | 0.856 | 2.468 | 0.653 |
| 40.0 | 0.18 | 31.21 | 2.452 | 2.473 | 0.856 | 2.469 | 0.693 | 2.466 | 0.571 |
| 45.0 | 0.21 | 35.11 | 2.454 | 2.472 | 0.733 | 2.467 | 0.530 | 2.464 | 0.407 |
| 50.0 | 0.23 | 39.01 | 2.452 | 2.472 | 0.816 | 2.465 | 0.530 | 2.463 | 0.449 |
| 55.0 | 0.25 | 42.91 | 2.452 | 2.472 | 0.816 | 2.464 | 0.489 | 2.461 | 0.367 |
| 60.0 | 0.28 | 46.82 | 2.452 | 2.473 | 0.856 | 2.462 | 0.408 | 2.460 | 0.326 |
| 65.0 | 0.30 | 50.72 | 2.452 | 2.473 | 0.856 | 2.461 | 0.367 | 2.459 | 0.285 |
| 70.0 | 0.32 | 54.62 | 2.451 | 2.473 | 0.898 | 2.460 | 0.367 | 2.458 | 0.286 |
| 75.0 | 0.34 | 58.52 | 2.450 | 2.473 | 0.939 | 2.458 | 0.327 | 2.457 | 0.286 |
| 80.0 | 0.37 | 62.42 | 2.449 | 2.473 | 0.980 | 2.457 | 0.327 | 2.456 | 0.286 |
| 85.0 | 0.39 | 66.32 | 2.448 | 2.473 | 1.021 | 2.456 | 0.327 | 2.454 | 0.245 |
| 90.0 | 0.41 | 70.22 | 2.447 | 2.473 | 1.063 | 2.454 | 0.286 | 2.453 | 0.245 |
| 95.0 | 0.44 | 74.12 | 2.446 | 2.473 | 1.104 | 2.453 | 0.286 | 2.452 | 0.245 |
| 100.0 | 0.46 | 78.03 | 2.445 | 2.473 | 1.145 | 2.451 | 0.245 | 2.450 | 0.204 |
| 105.0 | 0.48 | 81.93 | 2.443 | 2.472 | 1.187 | 2.450 | 0.287 | 2.449 | 0.246 |
| 110.0 | 0.51 | 85.83 | 2.442 | 2.472 | 1.229 | 2.448 | 0.246 | 2.447 | 0.205 |
| 115.0 | 0.53 | 89.73 | 2.442 | 2.471 | 1.188 | 2.446 | 0.164 | 2.445 | 0.123 |
| 120.0 | 0.55 | 93.63 | 2.440 | 2.471 | 1.270 | 2.445 | 0.205 | 2.444 | 0.164 |
| 125.0 | 0.57 | 97.53 | 2.438 | 2.470 | 1.313 | 2.443 | 0.205 | 2.442 | 0.164 |
| 130.0 | 0.60 | 101.43 | 2.437 | 2.469 | 1.313 | 2.442 | 0.205 | 2.441 | 0.164 |
| 135.0 | 0.62 | 105.33 | 2.437 | 2.469 | 1.313 | 2.440 | 0.123 | 2.439 | 0.082 |
| 140.0 | 0.64 | 109.24 | 2.436 | 2.468 | 1.314 | 2.439 | 0.123 | 2.438 | 0.082 |
| 145.0 | 0.67 | 113.14 | 2.434 | 2.467 | 1.356 | 2.437 | 0.123 | 2.436 | 0.082 |
| 150.0 | 0.69 | 117.04 | 2.432 | 2.466 | 1.398 | 2.436 | 0.164 | 2.435 | 0.123 |
| 155.0 | 0.71 | 120.94 | 2.432 | 2.466 | 1.398 | 2.434 | 0.082 | 2.433 | 0.041 |
| 160.0 | 0.74 | 124.84 | 2.430 | 2.465 | 1.440 | 2.433 | 0.123 | 2.432 | 0.082 |
| 165.0 | 0.76 | 128.74 | 2.429 | 2.464 | 1.441 | 2.431 | 0.082 | 2.431 | 0.082 |
| 170.0 | 0.78 | 132.64 | 2.428 | 2.463 | 1.442 | 2.430 | 0.082 | 2.429 | 0.041 |
| 175.0 | 0.80 | 136.54 | 2.427 | 2.462 | 1.442 | 2.428 | 0.041 | 2.428 | 0.041 |
| 180.0 | 0.83 | 140.45 | 2.426 | 2.462 | 1.484 | 2.427 | 0.041 | 2.427 | 0.041 |
| 185.0 | 0.85 | 144.35 | 2.425 | 2.461 | 1.485 | 2.426 | 0.041 | 2.425 | 0.000 |
| 190.0 | 0.87 | 148.25 | 2.424 | 2.460 | 1.485 | 2.425 | 0.041 | 2.424 | 0.000 |
| 195.0 | 0.90 | 152.15 | 2.423 | 2.459 | 1.486 | 2.423 | 0.000 | 2.423 | 0.000 |
| 200.0 | 0.92 | 156.05 | 2.422 | 2.458 | 1.486 | 2.422 | 0.000 | 2.422 | 0.000 |

**Table 2f.** Key properties of the pair correlation function resulting from Langevin dynamics simulations and three integral theory approaches: the hypernetted-chain approximation (HNC), isomorph-based empirically modified hypernetted-chain approximation (IEMHNC) and empirically modified hypernetted-chain approximation (EMHNC). The absolute relative deviation $\epsilon_{\mathrm{r}}$ between the theoretical and the simulation results is also reported. **Results for the magnitude of the second maximum in the case of $\boldsymbol{\kappa = 1}$.** The LD results are adopted from Table 5 of *T. Ott and M. Bonitz, Contrib. Plasma Phys.* **55**, *243 (2015)*.

| $\Gamma$ | $\Gamma/\Gamma_{\mathrm{m}}$ | $\Gamma_{\mathrm{iso}}^{\mathrm{OCP}}$ | $g_{\mathrm{max2}}^{\mathrm{LD}}$ | $g_{\mathrm{max2}}^{\mathrm{HNC}}$ | $\epsilon_{\mathrm{HNC}}(\%)$ | $g_{\mathrm{max2}}^{\mathrm{IEMHNC}}$ | $\epsilon_{\mathrm{IEMHNC}}(\%)$ | $g_{\mathrm{max2}}^{\mathrm{EMHNC}}$ | $\epsilon_{\mathrm{EMHNC}}(\%)$ |
|---|---|---|---|---|---|---|---|---|---|
| 10.0 | 0.05 | 7.80 | 1.002 | 1.001 | 0.110 | 1.001 | 0.093 | 1.002 | 0.043 |
| 15.0 | 0.07 | 11.70 | 1.007 | 1.003 | 0.362 | 1.005 | 0.152 | 1.006 | 0.099 |
| 20.0 | 0.09 | 15.61 | 1.014 | 1.007 | 0.680 | 1.012 | 0.245 | 1.012 | 0.176 |
| 25.0 | 0.11 | 19.51 | 1.022 | 1.012 | 1.004 | 1.019 | 0.309 | 1.020 | 0.204 |
| 30.0 | 0.14 | 23.41 | 1.031 | 1.017 | 1.361 | 1.027 | 0.372 | 1.029 | 0.234 |
| 35.0 | 0.16 | 27.31 | 1.041 | 1.023 | 1.770 | 1.036 | 0.466 | 1.038 | 0.299 |
| 40.0 | 0.18 | 31.21 | 1.050 | 1.028 | 2.053 | 1.046 | 0.424 | 1.048 | 0.231 |
| 45.0 | 0.21 | 35.11 | 1.060 | 1.034 | 2.409 | 1.055 | 0.453 | 1.057 | 0.237 |
| 50.0 | 0.23 | 39.01 | 1.070 | 1.041 | 2.749 | 1.065 | 0.468 | 1.068 | 0.230 |
| 55.0 | 0.25 | 42.91 | 1.080 | 1.047 | 3.079 | 1.075 | 0.477 | 1.078 | 0.217 |
| 60.0 | 0.28 | 46.82 | 1.090 | 1.053 | 3.400 | 1.085 | 0.485 | 1.088 | 0.204 |
| 65.0 | 0.30 | 50.72 | 1.100 | 1.059 | 3.716 | 1.095 | 0.495 | 1.098 | 0.193 |
| 70.0 | 0.32 | 54.62 | 1.109 | 1.065 | 3.943 | 1.104 | 0.420 | 1.108 | 0.096 |
| 75.0 | 0.34 | 58.52 | 1.118 | 1.071 | 4.168 | 1.114 | 0.352 | 1.118 | 0.007 |
| 80.0 | 0.37 | 62.42 | 1.127 | 1.077 | 4.394 | 1.124 | 0.292 | 1.128 | 0.074 |
| 85.0 | 0.39 | 66.32 | 1.137 | 1.084 | 4.705 | 1.133 | 0.330 | 1.138 | 0.057 |
| 90.0 | 0.41 | 70.22 | 1.145 | 1.089 | 4.849 | 1.143 | 0.201 | 1.147 | 0.206 |
| 95.0 | 0.44 | 74.12 | 1.153 | 1.095 | 4.997 | 1.152 | 0.084 | 1.157 | 0.344 |
| 100.0 | 0.46 | 78.03 | 1.162 | 1.101 | 5.229 | 1.161 | 0.064 | 1.166 | 0.384 |
| 105.0 | 0.48 | 81.93 | 1.170 | 1.107 | 5.383 | 1.170 | 0.031 | 1.176 | 0.500 |
| 110.0 | 0.51 | 85.83 | 1.178 | 1.113 | 5.540 | 1.179 | 0.115 | 1.185 | 0.603 |
| 115.0 | 0.53 | 89.73 | 1.185 | 1.118 | 5.621 | 1.188 | 0.272 | 1.194 | 0.779 |
| 120.0 | 0.55 | 93.63 | 1.193 | 1.124 | 5.786 | 1.197 | 0.332 | 1.203 | 0.858 |
| 125.0 | 0.57 | 97.53 | 1.200 | 1.129 | 5.876 | 1.206 | 0.466 | 1.212 | 1.010 |
| 130.0 | 0.60 | 101.43 | 1.207 | 1.135 | 5.970 | 1.214 | 0.587 | 1.221 | 1.149 |
| 135.0 | 0.62 | 105.33 | 1.214 | 1.140 | 6.069 | 1.222 | 0.697 | 1.229 | 1.276 |
| 140.0 | 0.64 | 109.24 | 1.220 | 1.146 | 6.095 | 1.231 | 0.877 | 1.238 | 1.474 |
| 145.0 | 0.67 | 113.14 | 1.227 | 1.151 | 6.202 | 1.239 | 0.964 | 1.246 | 1.577 |
| 150.0 | 0.69 | 117.04 | 1.233 | 1.156 | 6.238 | 1.247 | 1.122 | 1.255 | 1.750 |
| 155.0 | 0.71 | 120.94 | 1.239 | 1.161 | 6.278 | 1.255 | 1.267 | 1.263 | 1.911 |
| 160.0 | 0.74 | 124.84 | 1.246 | 1.166 | 6.399 | 1.262 | 1.321 | 1.271 | 1.978 |
| 165.0 | 0.76 | 128.74 | 1.251 | 1.171 | 6.373 | 1.270 | 1.525 | 1.278 | 2.197 |
| 170.0 | 0.78 | 132.64 | 1.256 | 1.176 | 6.353 | 1.278 | 1.718 | 1.286 | 2.404 |
| 175.0 | 0.80 | 136.54 | 1.262 | 1.181 | 6.411 | 1.285 | 1.820 | 1.294 | 2.518 |
| 180.0 | 0.83 | 140.45 | 1.267 | 1.186 | 6.400 | 1.292 | 1.991 | 1.301 | 2.702 |
| 185.0 | 0.85 | 144.35 | 1.272 | 1.191 | 6.394 | 1.299 | 2.151 | 1.309 | 2.874 |
| 190.0 | 0.87 | 148.25 | 1.277 | 1.195 | 6.393 | 1.306 | 2.301 | 1.316 | 3.034 |
| 195.0 | 0.90 | 152.15 | 1.281 | 1.200 | 6.323 | 1.313 | 2.520 | 1.323 | 3.264 |
| 200.0 | 0.92 | 156.05 | 1.286 | 1.205 | 6.330 | 1.320 | 2.649 | 1.330 | 3.403 |

**Table 2g.** Key properties of the pair correlation function resulting from Langevin dynamics simulations and three integral theory approaches: the hypernetted-chain approximation (HNC), isomorph-based empirically modified hypernetted-chain approximation (IEMHNC) and empirically modified hypernetted-chain approximation (EMHNC). The absolute relative deviation $\epsilon_{\mathrm{r}}$ between the theoretical and the simulation results is also reported. **Results for the position of the second maximum in the case of $\boldsymbol{\kappa = 1}$**. The LD results are adopted from Table 5 of *T. Ott and M. Bonitz, Contrib. Plasma Phys.* **55**, *243 (2015)*.

| $\Gamma$ | $\Gamma/\Gamma_{\mathrm{m}}$ | $\Gamma_{\mathrm{iso}}^{\mathrm{OCP}}$ | $r_{\mathrm{max2}}^{\mathrm{LD}}/d$ | $r_{\mathrm{max2}}^{\mathrm{HNC}}/d$ | $\epsilon_{\mathrm{HNC}}(\%)$ | $r_{\mathrm{max2}}^{\mathrm{IEMHNC}}/d$ | $\epsilon_{\mathrm{IEMHNC}}(\%)$ | $r_{\mathrm{max2}}^{\mathrm{EMHNC}}/d$ | $\epsilon_{\mathrm{EMHNC}}(\%)$ |
|---|---|---|---|---|---|---|---|---|---|
| 10.0 | 0.05 | 7.80 | 3.437 | 3.513 | 2.211 | 3.480 | 1.251 | 3.464 | 0.786 |
| 15.0 | 0.07 | 11.70 | 3.322 | 3.389 | 2.017 | 3.378 | 1.686 | 3.382 | 1.806 |
| 20.0 | 0.09 | 15.61 | 3.277 | 3.335 | 1.770 | 3.336 | 1.800 | 3.326 | 1.495 |
| 25.0 | 0.11 | 19.51 | 3.253 | 3.306 | 1.629 | 3.303 | 1.537 | 3.292 | 1.199 |
| 30.0 | 0.14 | 23.41 | 3.241 | 3.289 | 1.481 | 3.281 | 1.234 | 3.272 | 0.956 |
| 35.0 | 0.16 | 27.31 | 3.236 | 3.277 | 1.267 | 3.266 | 0.927 | 3.258 | 0.680 |
| 40.0 | 0.18 | 31.21 | 3.237 | 3.269 | 0.989 | 3.256 | 0.587 | 3.250 | 0.402 |
| 45.0 | 0.21 | 35.11 | 3.230 | 3.263 | 1.022 | 3.249 | 0.588 | 3.244 | 0.433 |
| 50.0 | 0.23 | 39.01 | 3.228 | 3.258 | 0.929 | 3.244 | 0.496 | 3.240 | 0.372 |
| 55.0 | 0.25 | 42.91 | 3.228 | 3.255 | 0.836 | 3.240 | 0.372 | 3.237 | 0.279 |
| 60.0 | 0.28 | 46.82 | 3.224 | 3.252 | 0.868 | 3.238 | 0.434 | 3.235 | 0.341 |
| 65.0 | 0.30 | 50.72 | 3.227 | 3.250 | 0.713 | 3.236 | 0.279 | 3.234 | 0.217 |
| 70.0 | 0.32 | 54.62 | 3.224 | 3.248 | 0.744 | 3.235 | 0.341 | 3.234 | 0.310 |
| 75.0 | 0.34 | 58.52 | 3.226 | 3.246 | 0.620 | 3.234 | 0.248 | 3.233 | 0.217 |
| 80.0 | 0.37 | 62.42 | 3.224 | 3.245 | 0.651 | 3.234 | 0.310 | 3.233 | 0.279 |
| 85.0 | 0.39 | 66.32 | 3.225 | 3.244 | 0.589 | 3.234 | 0.279 | 3.233 | 0.248 |
| 90.0 | 0.41 | 70.22 | 3.224 | 3.244 | 0.620 | 3.234 | 0.310 | 3.234 | 0.310 |
| 95.0 | 0.44 | 74.12 | 3.224 | 3.243 | 0.589 | 3.234 | 0.310 | 3.234 | 0.310 |
| 100.0 | 0.46 | 78.03 | 3.226 | 3.243 | 0.527 | 3.235 | 0.279 | 3.235 | 0.279 |
| 105.0 | 0.48 | 81.93 | 3.226 | 3.242 | 0.496 | 3.235 | 0.279 | 3.235 | 0.279 |
| 110.0 | 0.51 | 85.83 | 3.226 | 3.242 | 0.496 | 3.236 | 0.310 | 3.236 | 0.310 |
| 115.0 | 0.53 | 89.73 | 3.227 | 3.242 | 0.465 | 3.236 | 0.279 | 3.237 | 0.310 |
| 120.0 | 0.55 | 93.63 | 3.227 | 3.242 | 0.465 | 3.237 | 0.310 | 3.238 | 0.341 |
| 125.0 | 0.57 | 97.53 | 3.227 | 3.242 | 0.465 | 3.238 | 0.341 | 3.239 | 0.372 |
| 130.0 | 0.60 | 101.43 | 3.227 | 3.242 | 0.465 | 3.239 | 0.372 | 3.240 | 0.403 |
| 135.0 | 0.62 | 105.33 | 3.227 | 3.242 | 0.465 | 3.240 | 0.403 | 3.240 | 0.403 |
| 140.0 | 0.64 | 109.24 | 3.228 | 3.242 | 0.434 | 3.241 | 0.403 | 3.241 | 0.403 |
| 145.0 | 0.67 | 113.14 | 3.228 | 3.243 | 0.465 | 3.241 | 0.403 | 3.242 | 0.434 |
| 150.0 | 0.69 | 117.04 | 3.229 | 3.243 | 0.434 | 3.242 | 0.403 | 3.243 | 0.434 |
| 155.0 | 0.71 | 120.94 | 3.228 | 3.243 | 0.465 | 3.243 | 0.465 | 3.244 | 0.496 |
| 160.0 | 0.74 | 124.84 | 3.228 | 3.243 | 0.465 | 3.244 | 0.496 | 3.245 | 0.527 |
| 165.0 | 0.76 | 128.74 | 3.229 | 3.244 | 0.465 | 3.245 | 0.496 | 3.246 | 0.526 |
| 170.0 | 0.78 | 132.64 | 3.229 | 3.244 | 0.465 | 3.246 | 0.526 | 3.247 | 0.557 |
| 175.0 | 0.80 | 136.54 | 3.230 | 3.244 | 0.433 | 3.247 | 0.526 | 3.248 | 0.557 |
| 180.0 | 0.83 | 140.45 | 3.230 | 3.244 | 0.433 | 3.248 | 0.557 | 3.249 | 0.588 |
| 185.0 | 0.85 | 144.35 | 3.231 | 3.245 | 0.433 | 3.249 | 0.557 | 3.250 | 0.588 |
| 190.0 | 0.87 | 148.25 | 3.230 | 3.245 | 0.464 | 3.250 | 0.619 | 3.251 | 0.650 |
| 195.0 | 0.90 | 152.15 | 3.231 | 3.246 | 0.464 | 3.251 | 0.619 | 3.252 | 0.650 |
| 200.0 | 0.92 | 156.05 | 3.232 | 3.246 | 0.433 | 3.252 | 0.619 | 3.253 | 0.650 |

**Table 3a.** Key properties of the pair correlation function resulting from Langevin dynamics simulations and three integral theory approaches: the hypernetted-chain approximation (HNC), isomorph-based empirically modified hypernetted-chain approximation (IEMHNC) and empirically modified hypernetted-chain approximation (EMHNC). The absolute relative deviation $\epsilon_{\mathrm{r}}$ between the theoretical and the simulation results is also reported. **Results for $\arg_r\{g(r)=0.5\}$ in the case of $\kappa=2$**. The LD results are adopted from Table 6 of *T. Ott and M. Bonitz, Contrib. Plasma Phys.* **55**, *243 (2015).*

| $\Gamma$ | $\Gamma/\Gamma_{\mathrm{m}}$ | $\Gamma_{\mathrm{iso}}^{\mathrm{OCP}}$ | $r_{\mathrm{cv}}^{\mathrm{LD}}/d$ | $r_{\mathrm{cv}}^{\mathrm{HNC}}/d$ | $\epsilon_{\mathrm{HNC}}(\%)$ | $r_{\mathrm{cv}}^{\mathrm{IEMHNC}}/d$ | $\epsilon_{\mathrm{IEMHNC}}(\%)$ | $r_{\mathrm{cv}}^{\mathrm{EMHNC}}/d$ | $\epsilon_{\mathrm{EMHNC}}(\%)$ |
|---|---|---|---|---|---|---|---|---|---|
| 30.0 | 0.07 | 11.25 | 1.135 | 1.113 | 1.938 | 1.123 | 1.057 | 1.136 | 0.088 |
| 40.0 | 0.09 | 15.00 | 1.176 | 1.153 | 1.956 | 1.167 | 0.765 | 1.179 | 0.255 |
| 50.0 | 0.11 | 18.75 | 1.209 | 1.182 | 2.233 | 1.200 | 0.744 | 1.211 | 0.165 |
| 60.0 | 0.14 | 22.50 | 1.234 | 1.205 | 2.350 | 1.226 | 0.648 | 1.236 | 0.162 |
| 70.0 | 0.16 | 26.24 | 1.254 | 1.225 | 2.313 | 1.247 | 0.558 | 1.257 | 0.239 |
| 80.0 | 0.18 | 29.99 | 1.272 | 1.241 | 2.437 | 1.266 | 0.472 | 1.275 | 0.236 |
| 90.0 | 0.20 | 33.74 | 1.288 | 1.255 | 2.562 | 1.281 | 0.543 | 1.291 | 0.233 |
| 100.0 | 0.23 | 37.49 | 1.301 | 1.268 | 2.537 | 1.295 | 0.461 | 1.304 | 0.231 |
| 110.0 | 0.25 | 41.24 | 1.313 | 1.279 | 2.589 | 1.308 | 0.381 | 1.317 | 0.305 |
| 120.0 | 0.27 | 44.99 | 1.324 | 1.289 | 2.644 | 1.319 | 0.378 | 1.328 | 0.302 |
| 130.0 | 0.30 | 48.74 | 1.333 | 1.298 | 2.626 | 1.329 | 0.300 | 1.338 | 0.375 |
| 140.0 | 0.32 | 52.49 | 1.342 | 1.307 | 2.608 | 1.338 | 0.298 | 1.347 | 0.373 |
| 150.0 | 0.34 | 56.24 | 1.351 | 1.315 | 2.665 | 1.347 | 0.296 | 1.356 | 0.370 |
| 160.0 | 0.36 | 59.99 | 1.358 | 1.322 | 2.651 | 1.355 | 0.221 | 1.363 | 0.368 |
| 170.0 | 0.39 | 63.74 | 1.366 | 1.329 | 2.709 | 1.362 | 0.293 | 1.371 | 0.366 |
| 180.0 | 0.41 | 67.49 | 1.373 | 1.335 | 2.768 | 1.369 | 0.291 | 1.378 | 0.364 |
| 190.0 | 0.43 | 71.23 | 1.378 | 1.341 | 2.685 | 1.376 | 0.145 | 1.384 | 0.435 |
| 200.0 | 0.45 | 74.98 | 1.384 | 1.346 | 2.746 | 1.382 | 0.145 | 1.391 | 0.506 |
| 210.0 | 0.48 | 78.73 | 1.389 | 1.352 | 2.664 | 1.388 | 0.072 | 1.397 | 0.576 |
| 220.0 | 0.50 | 82.48 | 1.396 | 1.357 | 2.794 | 1.393 | 0.215 | 1.402 | 0.430 |
| 230.0 | 0.52 | 86.23 | 1.400 | 1.361 | 2.786 | 1.398 | 0.143 | 1.407 | 0.500 |
| 240.0 | 0.55 | 89.98 | 1.405 | 1.366 | 2.776 | 1.403 | 0.142 | 1.412 | 0.498 |
| 250.0 | 0.57 | 93.73 | 1.409 | 1.370 | 2.768 | 1.408 | 0.071 | 1.417 | 0.568 |
| 260.0 | 0.59 | 97.48 | 1.414 | 1.374 | 2.829 | 1.413 | 0.071 | 1.422 | 0.566 |
| 270.0 | 0.61 | 101.23 | 1.418 | 1.378 | 2.821 | 1.417 | 0.071 | 1.426 | 0.564 |
| 280.0 | 0.64 | 104.98 | 1.423 | 1.382 | 2.881 | 1.421 | 0.141 | 1.431 | 0.562 |
| 290.0 | 0.66 | 108.73 | 1.427 | 1.386 | 2.873 | 1.425 | 0.140 | 1.435 | 0.561 |
| 300.0 | 0.68 | 112.48 | 1.429 | 1.389 | 2.799 | 1.429 | 0.000 | 1.439 | 0.700 |
| 310.0 | 0.70 | 116.23 | 1.434 | 1.393 | 2.859 | 1.433 | 0.070 | 1.442 | 0.558 |
| 320.0 | 0.73 | 119.97 | 1.436 | 1.396 | 2.786 | 1.436 | 0.000 | 1.446 | 0.696 |
| 330.0 | 0.75 | 123.72 | 1.441 | 1.399 | 2.915 | 1.440 | 0.069 | 1.449 | 0.555 |
| 340.0 | 0.77 | 127.47 | 1.443 | 1.402 | 2.841 | 1.443 | 0.000 | 1.453 | 0.693 |
| 350.0 | 0.80 | 131.22 | 1.447 | 1.405 | 2.903 | 1.447 | 0.000 | 1.456 | 0.622 |
| 360.0 | 0.82 | 134.97 | 1.450 | 1.408 | 2.897 | 1.450 | 0.000 | 1.459 | 0.621 |
| 370.0 | 0.84 | 138.72 | 1.452 | 1.411 | 2.824 | 1.453 | 0.069 | 1.462 | 0.689 |
| 380.0 | 0.86 | 142.47 | 1.456 | 1.414 | 2.885 | 1.456 | 0.000 | 1.465 | 0.618 |
| 390.0 | 0.89 | 146.22 | 1.459 | 1.416 | 2.947 | 1.459 | 0.000 | 1.468 | 0.617 |
| 400.0 | 0.91 | 149.97 | 1.461 | 1.419 | 2.875 | 1.461 | 0.000 | 1.471 | 0.684 |

**Table 3b.** Key properties of the pair correlation function resulting from Langevin dynamics simulations and three integral theory approaches: the hypernetted-chain approximation (HNC), isomorph-based empirically modified hypernetted-chain approximation (IEMHNC) and empirically modified hypernetted-chain approximation (EMHNC). The absolute relative deviation $\epsilon_{\mathrm{r}}$ between the theoretical and the simulation results is also reported. **Results for the magnitude of the first maximum in the case of $\boldsymbol{\kappa = 2}$**. The LD results are adopted from Table 6 of *T. Ott and M. Bonitz, Contrib. Plasma Phys.* **55**, *243 (2015)*.

| $\Gamma$ | $\Gamma/\Gamma_{\mathrm{m}}$ | $\Gamma_{\mathrm{iso}}^{\mathrm{OCP}}$ | $g_{\mathrm{max1}}^{\mathrm{LD}}$ | $g_{\mathrm{max1}}^{\mathrm{HNC}}$ | $\epsilon_{\mathrm{HNC}}(\%)$ | $g_{\mathrm{max1}}^{\mathrm{IEMHNC}}$ | $\epsilon_{\mathrm{IEMHNC}}(\%)$ | $g_{\mathrm{max1}}^{\mathrm{EMHNC}}$ | $\epsilon_{\mathrm{EMHNC}}(\%)$ |
|---|---|---|---|---|---|---|---|---|---|
| 30.0 | 0.07 | 11.25 | 1.202 | 1.169 | 2.711 | 1.180 | 1.808 | 1.201 | 0.067 |
| 40.0 | 0.09 | 15.00 | 1.270 | 1.225 | 3.508 | 1.244 | 2.015 | 1.273 | 0.202 |
| 50.0 | 0.11 | 18.75 | 1.331 | 1.276 | 4.148 | 1.306 | 1.911 | 1.337 | 0.482 |
| 60.0 | 0.14 | 22.50 | 1.388 | 1.322 | 4.777 | 1.363 | 1.772 | 1.397 | 0.655 |
| 70.0 | 0.16 | 26.24 | 1.440 | 1.364 | 5.271 | 1.418 | 1.537 | 1.453 | 0.877 |
| 80.0 | 0.18 | 29.99 | 1.490 | 1.404 | 5.797 | 1.469 | 1.393 | 1.505 | 0.993 |
| 90.0 | 0.20 | 33.74 | 1.536 | 1.441 | 6.201 | 1.518 | 1.179 | 1.554 | 1.183 |
| 100.0 | 0.23 | 37.49 | 1.582 | 1.476 | 6.710 | 1.564 | 1.130 | 1.601 | 1.212 |
| 110.0 | 0.25 | 41.24 | 1.624 | 1.509 | 7.068 | 1.608 | 0.969 | 1.646 | 1.365 |
| 120.0 | 0.27 | 44.99 | 1.664 | 1.541 | 7.389 | 1.651 | 0.808 | 1.689 | 1.526 |
| 130.0 | 0.30 | 48.74 | 1.702 | 1.572 | 7.665 | 1.691 | 0.634 | 1.731 | 1.709 |
| 140.0 | 0.32 | 52.49 | 1.741 | 1.601 | 8.050 | 1.730 | 0.609 | 1.771 | 1.745 |
| 150.0 | 0.34 | 56.24 | 1.777 | 1.629 | 8.324 | 1.768 | 0.490 | 1.810 | 1.883 |
| 160.0 | 0.36 | 59.99 | 1.812 | 1.656 | 8.589 | 1.805 | 0.385 | 1.848 | 2.010 |
| 170.0 | 0.39 | 63.74 | 1.847 | 1.683 | 8.892 | 1.841 | 0.342 | 1.885 | 2.077 |
| 180.0 | 0.41 | 67.49 | 1.879 | 1.708 | 9.081 | 1.875 | 0.192 | 1.921 | 2.256 |
| 190.0 | 0.43 | 71.23 | 1.912 | 1.733 | 9.350 | 1.909 | 0.147 | 1.957 | 2.330 |
| 200.0 | 0.45 | 74.98 | 1.944 | 1.757 | 9.597 | 1.942 | 0.093 | 1.991 | 2.413 |
| 210.0 | 0.48 | 78.73 | 1.974 | 1.781 | 9.777 | 1.974 | 0.022 | 2.025 | 2.560 |
| 220.0 | 0.50 | 82.48 | 2.004 | 1.804 | 9.981 | 2.006 | 0.099 | 2.057 | 2.668 |
| 230.0 | 0.52 | 86.23 | 2.034 | 1.826 | 10.204 | 2.037 | 0.142 | 2.090 | 2.740 |
| 240.0 | 0.55 | 89.98 | 2.062 | 1.848 | 10.359 | 2.067 | 0.251 | 2.121 | 2.881 |
| 250.0 | 0.57 | 93.73 | 2.091 | 1.870 | 10.576 | 2.097 | 0.282 | 2.152 | 2.940 |
| 260.0 | 0.59 | 97.48 | 2.119 | 1.891 | 10.765 | 2.126 | 0.334 | 2.183 | 3.021 |
| 270.0 | 0.61 | 101.23 | 2.145 | 1.911 | 10.886 | 2.155 | 0.454 | 2.213 | 3.171 |
| 280.0 | 0.64 | 104.98 | 2.173 | 1.932 | 11.104 | 2.183 | 0.457 | 2.243 | 3.199 |
| 290.0 | 0.66 | 108.73 | 2.198 | 1.952 | 11.212 | 2.211 | 0.577 | 2.272 | 3.346 |
| 300.0 | 0.68 | 112.48 | 2.225 | 1.971 | 11.414 | 2.238 | 0.584 | 2.300 | 3.375 |
| 310.0 | 0.70 | 116.23 | 2.250 | 1.990 | 11.547 | 2.265 | 0.661 | 2.328 | 3.475 |
| 320.0 | 0.73 | 119.97 | 2.274 | 2.009 | 11.653 | 2.291 | 0.764 | 2.356 | 3.601 |
| 330.0 | 0.75 | 123.72 | 2.299 | 2.028 | 11.808 | 2.318 | 0.805 | 2.383 | 3.660 |
| 340.0 | 0.77 | 127.47 | 2.324 | 2.046 | 11.973 | 2.343 | 0.829 | 2.410 | 3.701 |
| 350.0 | 0.80 | 131.22 | 2.347 | 2.064 | 12.071 | 2.369 | 0.925 | 2.436 | 3.813 |
| 360.0 | 0.82 | 134.97 | 2.371 | 2.081 | 12.215 | 2.394 | 0.961 | 2.463 | 3.863 |
| 370.0 | 0.84 | 138.72 | 2.394 | 2.099 | 12.330 | 2.419 | 1.026 | 2.488 | 3.940 |
| 380.0 | 0.86 | 142.47 | 2.417 | 2.116 | 12.453 | 2.443 | 1.076 | 2.514 | 4.001 |
| 390.0 | 0.89 | 146.22 | 2.438 | 2.133 | 12.512 | 2.467 | 1.196 | 2.539 | 4.132 |
| 400.0 | 0.91 | 149.97 | 2.462 | 2.150 | 12.686 | 2.491 | 1.179 | 2.563 | 4.120 |

**Table 3c.** Key properties of the pair correlation function resulting from Langevin dynamics simulations and three integral theory approaches: the hypernetted-chain approximation (HNC), isomorph-based empirically modified hypernetted-chain approximation (IEMHNC) and empirically modified hypernetted-chain approximation (EMHNC). The absolute relative deviation $\epsilon_{\rm r}$ between the theoretical and the simulation results is also reported. **Results for the position of the first maximum in the case of $\boldsymbol{\kappa = 2}$**. The LD results are adopted from Table 6 of *T. Ott and M. Bonitz, Contrib. Plasma Phys.* **55**, *243 (2015)*.

| $\Gamma$ | $\Gamma/\Gamma_{\rm m}$ | $\Gamma_{\rm iso}^{\rm OCP}$ | $r_{\rm max1}^{\rm LD}/d$ | $r_{\rm max1}^{\rm HNC}/d$ | $\epsilon_{\rm HNC}(\%)$ | $r_{\rm max1}^{\rm IEMHNC}/d$ | $\epsilon_{\rm IEMHNC}(\%)$ | $r_{\rm max1}^{\rm EMHNC}/d$ | $\epsilon_{\rm EMHNC}(\%)$ |
|---|---|---|---|---|---|---|---|---|---|
| 30.0 | 0.07 | 11.25 | 1.598 | 1.581 | 1.064 | 1.599 | 0.063 | 1.609 | 0.688 |
| 40.0 | 0.09 | 15.00 | 1.609 | 1.587 | 1.367 | 1.611 | 0.124 | 1.615 | 0.373 |
| 50.0 | 0.11 | 18.75 | 1.619 | 1.594 | 1.544 | 1.619 | 0.000 | 1.622 | 0.185 |
| 60.0 | 0.14 | 22.50 | 1.627 | 1.600 | 1.659 | 1.625 | 0.123 | 1.629 | 0.123 |
| 70.0 | 0.16 | 26.24 | 1.633 | 1.605 | 1.715 | 1.631 | 0.122 | 1.635 | 0.122 |
| 80.0 | 0.18 | 29.99 | 1.640 | 1.610 | 1.829 | 1.636 | 0.244 | 1.640 | 0.000 |
| 90.0 | 0.20 | 33.74 | 1.646 | 1.615 | 1.883 | 1.640 | 0.365 | 1.645 | 0.061 |
| 100.0 | 0.23 | 37.49 | 1.651 | 1.619 | 1.938 | 1.645 | 0.363 | 1.650 | 0.061 |
| 110.0 | 0.25 | 41.24 | 1.656 | 1.623 | 1.993 | 1.649 | 0.423 | 1.655 | 0.060 |
| 120.0 | 0.27 | 44.99 | 1.660 | 1.627 | 1.988 | 1.653 | 0.422 | 1.659 | 0.060 |
| 130.0 | 0.30 | 48.74 | 1.664 | 1.630 | 2.043 | 1.656 | 0.481 | 1.663 | 0.060 |
| 140.0 | 0.32 | 52.49 | 1.668 | 1.633 | 2.098 | 1.659 | 0.540 | 1.667 | 0.060 |
| 150.0 | 0.34 | 56.24 | 1.671 | 1.636 | 2.095 | 1.662 | 0.539 | 1.671 | 0.000 |
| 160.0 | 0.36 | 59.99 | 1.674 | 1.639 | 2.091 | 1.665 | 0.538 | 1.674 | 0.000 |
| 170.0 | 0.39 | 63.74 | 1.677 | 1.642 | 2.087 | 1.668 | 0.537 | 1.677 | 0.000 |
| 180.0 | 0.41 | 67.49 | 1.680 | 1.644 | 2.143 | 1.671 | 0.536 | 1.680 | 0.000 |
| 190.0 | 0.43 | 71.23 | 1.683 | 1.647 | 2.139 | 1.674 | 0.535 | 1.683 | 0.000 |
| 200.0 | 0.45 | 74.98 | 1.685 | 1.649 | 2.136 | 1.676 | 0.534 | 1.686 | 0.059 |
| 210.0 | 0.48 | 78.73 | 1.687 | 1.651 | 2.134 | 1.678 | 0.533 | 1.689 | 0.119 |
| 220.0 | 0.50 | 82.48 | 1.690 | 1.653 | 2.189 | 1.681 | 0.533 | 1.691 | 0.059 |
| 230.0 | 0.52 | 86.23 | 1.691 | 1.655 | 2.129 | 1.683 | 0.473 | 1.694 | 0.177 |
| 240.0 | 0.55 | 89.98 | 1.693 | 1.657 | 2.126 | 1.685 | 0.473 | 1.696 | 0.177 |
| 250.0 | 0.57 | 93.73 | 1.696 | 1.659 | 2.182 | 1.687 | 0.531 | 1.698 | 0.118 |
| 260.0 | 0.59 | 97.48 | 1.698 | 1.660 | 2.238 | 1.689 | 0.530 | 1.701 | 0.177 |
| 270.0 | 0.61 | 101.23 | 1.699 | 1.662 | 2.178 | 1.691 | 0.471 | 1.703 | 0.235 |
| 280.0 | 0.64 | 104.98 | 1.701 | 1.664 | 2.175 | 1.693 | 0.470 | 1.705 | 0.235 |
| 290.0 | 0.66 | 108.73 | 1.703 | 1.665 | 2.231 | 1.694 | 0.528 | 1.707 | 0.235 |
| 300.0 | 0.68 | 112.48 | 1.704 | 1.667 | 2.171 | 1.696 | 0.469 | 1.709 | 0.293 |
| 310.0 | 0.70 | 116.23 | 1.706 | 1.668 | 2.227 | 1.698 | 0.469 | 1.710 | 0.234 |
| 320.0 | 0.73 | 119.97 | 1.708 | 1.670 | 2.225 | 1.699 | 0.527 | 1.712 | 0.234 |
| 330.0 | 0.75 | 123.72 | 1.709 | 1.671 | 2.224 | 1.701 | 0.468 | 1.714 | 0.293 |
| 340.0 | 0.77 | 127.47 | 1.711 | 1.672 | 2.279 | 1.702 | 0.526 | 1.716 | 0.292 |
| 350.0 | 0.80 | 131.22 | 1.712 | 1.674 | 2.220 | 1.704 | 0.467 | 1.717 | 0.292 |
| 360.0 | 0.82 | 134.97 | 1.713 | 1.675 | 2.218 | 1.705 | 0.467 | 1.719 | 0.350 |
| 370.0 | 0.84 | 138.72 | 1.715 | 1.676 | 2.274 | 1.707 | 0.466 | 1.720 | 0.292 |
| 380.0 | 0.86 | 142.47 | 1.716 | 1.677 | 2.273 | 1.708 | 0.466 | 1.722 | 0.350 |
| 390.0 | 0.89 | 146.22 | 1.717 | 1.678 | 2.271 | 1.709 | 0.466 | 1.723 | 0.349 |
| 400.0 | 0.91 | 149.97 | 1.718 | 1.679 | 2.270 | 1.711 | 0.407 | 1.724 | 0.349 |

**Table 3d.** Key properties of the pair correlation function resulting from Langevin dynamics simulations and three integral theory approaches: the hypernetted-chain approximation (HNC), isomorph-based empirically modified hypernetted-chain approximation (IEMHNC) and empirically modified hypernetted-chain approximation (EMHNC). The absolute relative deviation $\epsilon_{\rm r}$ between the theoretical and the simulation results is also reported. **Results for the magnitude of the first minimum in the case of $\boldsymbol{\kappa = 2}$**. The LD results are adopted from Table 6 of *T. Ott and M. Bonitz, Contrib. Plasma Phys.* **55**, *243 (2015)*.

| $\Gamma$ | $\Gamma/\Gamma_{\rm m}$ | $\Gamma_{\rm iso}^{\rm OCP}$ | $g_{\rm min1}^{\rm LD}$ | $g_{\rm min1}^{\rm HNC}$ | $\epsilon_{\rm HNC}(\%)$ | $g_{\rm min1}^{\rm IEMHNC}$ | $\epsilon_{\rm IEMHNC}(\%)$ | $g_{\rm min1}^{\rm EMHNC}$ | $\epsilon_{\rm EMHNC}(\%)$ |
|---|---|---|---|---|---|---|---|---|---|
| 30.0 | 0.07 | 11.25 | 0.963 | 0.974 | 1.108 | 0.968 | 0.546 | 0.962 | 0.091 |
| 40.0 | 0.09 | 15.00 | 0.941 | 0.959 | 1.867 | 0.949 | 0.853 | 0.940 | 0.061 |
| 50.0 | 0.11 | 18.75 | 0.920 | 0.944 | 2.577 | 0.930 | 1.035 | 0.919 | 0.070 |
| 60.0 | 0.14 | 22.50 | 0.900 | 0.929 | 3.277 | 0.911 | 1.171 | 0.899 | 0.062 |
| 70.0 | 0.16 | 26.24 | 0.881 | 0.916 | 3.980 | 0.893 | 1.311 | 0.881 | 0.028 |
| 80.0 | 0.18 | 29.99 | 0.863 | 0.903 | 4.684 | 0.876 | 1.471 | 0.863 | 0.030 |
| 90.0 | 0.20 | 33.74 | 0.846 | 0.892 | 5.383 | 0.860 | 1.648 | 0.847 | 0.099 |
| 100.0 | 0.23 | 37.49 | 0.831 | 0.880 | 5.940 | 0.845 | 1.710 | 0.831 | 0.047 |
| 110.0 | 0.25 | 41.24 | 0.816 | 0.870 | 6.596 | 0.831 | 1.887 | 0.817 | 0.099 |
| 120.0 | 0.27 | 44.99 | 0.802 | 0.860 | 7.216 | 0.818 | 2.046 | 0.803 | 0.125 |
| 130.0 | 0.30 | 48.74 | 0.789 | 0.850 | 7.789 | 0.806 | 2.173 | 0.790 | 0.110 |
| 140.0 | 0.32 | 52.49 | 0.776 | 0.842 | 8.444 | 0.795 | 2.387 | 0.777 | 0.175 |
| 150.0 | 0.34 | 56.24 | 0.764 | 0.833 | 9.035 | 0.783 | 2.549 | 0.765 | 0.182 |
| 160.0 | 0.36 | 59.99 | 0.753 | 0.825 | 9.552 | 0.773 | 2.647 | 0.754 | 0.122 |
| 170.0 | 0.39 | 63.74 | 0.742 | 0.817 | 10.134 | 0.763 | 2.811 | 0.743 | 0.121 |
| 180.0 | 0.41 | 67.49 | 0.732 | 0.810 | 10.627 | 0.753 | 2.896 | 0.732 | 0.040 |
| 190.0 | 0.43 | 71.23 | 0.721 | 0.803 | 11.331 | 0.744 | 3.179 | 0.722 | 0.147 |
| 200.0 | 0.45 | 74.98 | 0.712 | 0.796 | 11.781 | 0.735 | 3.228 | 0.712 | 0.024 |
| 210.0 | 0.48 | 78.73 | 0.702 | 0.789 | 12.440 | 0.726 | 3.470 | 0.703 | 0.087 |
| 220.0 | 0.50 | 82.48 | 0.693 | 0.783 | 12.988 | 0.718 | 3.611 | 0.693 | 0.050 |
| 230.0 | 0.52 | 86.23 | 0.684 | 0.777 | 13.584 | 0.710 | 3.796 | 0.684 | 0.052 |
| 240.0 | 0.55 | 89.98 | 0.676 | 0.771 | 14.057 | 0.702 | 3.868 | 0.676 | 0.055 |
| 250.0 | 0.57 | 93.73 | 0.667 | 0.765 | 14.741 | 0.695 | 4.132 | 0.667 | 0.023 |
| 260.0 | 0.59 | 97.48 | 0.659 | 0.760 | 15.297 | 0.687 | 4.278 | 0.659 | 0.015 |
| 270.0 | 0.61 | 101.23 | 0.651 | 0.754 | 15.892 | 0.680 | 4.458 | 0.651 | 0.020 |
| 280.0 | 0.64 | 104.98 | 0.644 | 0.749 | 16.345 | 0.673 | 4.510 | 0.643 | 0.149 |
| 290.0 | 0.66 | 108.73 | 0.636 | 0.744 | 17.015 | 0.666 | 4.756 | 0.635 | 0.092 |
| 300.0 | 0.68 | 112.48 | 0.628 | 0.739 | 17.724 | 0.660 | 5.034 | 0.628 | 0.004 |
| 310.0 | 0.70 | 116.23 | 0.622 | 0.735 | 18.093 | 0.653 | 5.007 | 0.621 | 0.208 |
| 320.0 | 0.73 | 119.97 | 0.614 | 0.730 | 18.874 | 0.647 | 5.346 | 0.614 | 0.063 |
| 330.0 | 0.75 | 123.72 | 0.608 | 0.725 | 19.301 | 0.641 | 5.370 | 0.607 | 0.217 |
| 340.0 | 0.77 | 127.47 | 0.602 | 0.721 | 19.757 | 0.635 | 5.417 | 0.600 | 0.349 |
| 350.0 | 0.80 | 131.22 | 0.595 | 0.717 | 20.440 | 0.629 | 5.664 | 0.593 | 0.291 |
| 360.0 | 0.82 | 134.97 | 0.588 | 0.712 | 21.158 | 0.623 | 5.937 | 0.587 | 0.208 |
| 370.0 | 0.84 | 138.72 | 0.583 | 0.708 | 21.491 | 0.617 | 5.874 | 0.580 | 0.442 |
| 380.0 | 0.86 | 142.47 | 0.577 | 0.704 | 22.057 | 0.612 | 6.012 | 0.574 | 0.486 |
| 390.0 | 0.89 | 146.22 | 0.571 | 0.700 | 22.650 | 0.606 | 6.172 | 0.568 | 0.508 |
| 400.0 | 0.91 | 149.97 | 0.565 | 0.696 | 23.271 | 0.601 | 6.353 | 0.562 | 0.509 |

**Table 3e.** Key properties of the pair correlation function resulting from Langevin dynamics simulations and three integral theory approaches: the hypernetted-chain approximation (HNC), isomorph-based empirically modified hypernetted-chain approximation (IEMHNC) and empirically modified hypernetted-chain approximation (EMHNC). The absolute relative deviation $\epsilon_{\mathrm{r}}$ between the theoretical and the simulation results is also reported. **Results for the position of the first minimum in the case of $\boldsymbol{\kappa = 2}$**. The LD results are adopted from Table 6 of *T. Ott and M. Bonitz, Contrib. Plasma Phys.* **55**, *243 (2015)*.

| $\Gamma$ | $\Gamma/\Gamma_{\mathrm{m}}$ | $\Gamma_{\mathrm{iso}}^{\mathrm{OCP}}$ | $r_{\mathrm{min1}}^{\mathrm{LD}}/d$ | $r_{\mathrm{min1}}^{\mathrm{HNC}}/d$ | $\epsilon_{\mathrm{HNC}}(\%)$ | $r_{\mathrm{min1}}^{\mathrm{IEMHNC}}/d$ | $\epsilon_{\mathrm{IEMHNC}}(\%)$ | $r_{\mathrm{min1}}^{\mathrm{EMHNC}}/d$ | $\epsilon_{\mathrm{EMHNC}}(\%)$ |
|---|---|---|---|---|---|---|---|---|---|
| 30.0 | 0.07 | 11.25 | 2.409 | 2.415 | 0.249 | 2.438 | 1.204 | 2.434 | 1.038 |
| 40.0 | 0.09 | 15.00 | 2.408 | 2.413 | 0.208 | 2.441 | 1.370 | 2.427 | 0.789 |
| 50.0 | 0.11 | 18.75 | 2.414 | 2.415 | 0.041 | 2.439 | 1.036 | 2.427 | 0.539 |
| 60.0 | 0.14 | 22.50 | 2.419 | 2.419 | 0.000 | 2.438 | 0.785 | 2.429 | 0.413 |
| 70.0 | 0.16 | 26.24 | 2.422 | 2.423 | 0.041 | 2.438 | 0.661 | 2.432 | 0.413 |
| 80.0 | 0.18 | 29.99 | 2.427 | 2.427 | 0.000 | 2.439 | 0.494 | 2.434 | 0.288 |
| 90.0 | 0.20 | 33.74 | 2.428 | 2.431 | 0.124 | 2.439 | 0.453 | 2.436 | 0.329 |
| 100.0 | 0.23 | 37.49 | 2.431 | 2.434 | 0.123 | 2.440 | 0.370 | 2.437 | 0.247 |
| 110.0 | 0.25 | 41.24 | 2.432 | 2.436 | 0.164 | 2.440 | 0.329 | 2.438 | 0.247 |
| 120.0 | 0.27 | 44.99 | 2.434 | 2.438 | 0.164 | 2.440 | 0.247 | 2.439 | 0.205 |
| 130.0 | 0.30 | 48.74 | 2.433 | 2.440 | 0.288 | 2.440 | 0.288 | 2.439 | 0.247 |
| 140.0 | 0.32 | 52.49 | 2.434 | 2.442 | 0.329 | 2.440 | 0.247 | 2.439 | 0.205 |
| 150.0 | 0.34 | 56.24 | 2.434 | 2.443 | 0.370 | 2.440 | 0.247 | 2.439 | 0.205 |
| 160.0 | 0.36 | 59.99 | 2.433 | 2.444 | 0.452 | 2.439 | 0.247 | 2.439 | 0.247 |
| 170.0 | 0.39 | 63.74 | 2.435 | 2.445 | 0.411 | 2.438 | 0.123 | 2.438 | 0.123 |
| 180.0 | 0.41 | 67.49 | 2.433 | 2.445 | 0.493 | 2.437 | 0.164 | 2.437 | 0.164 |
| 190.0 | 0.43 | 71.23 | 2.432 | 2.446 | 0.576 | 2.436 | 0.164 | 2.437 | 0.206 |
| 200.0 | 0.45 | 74.98 | 2.433 | 2.446 | 0.534 | 2.435 | 0.082 | 2.436 | 0.123 |
| 210.0 | 0.48 | 78.73 | 2.432 | 2.446 | 0.576 | 2.434 | 0.082 | 2.435 | 0.123 |
| 220.0 | 0.50 | 82.48 | 2.430 | 2.446 | 0.658 | 2.433 | 0.123 | 2.434 | 0.165 |
| 230.0 | 0.52 | 86.23 | 2.429 | 2.446 | 0.700 | 2.432 | 0.124 | 2.433 | 0.165 |
| 240.0 | 0.55 | 89.98 | 2.429 | 2.446 | 0.700 | 2.431 | 0.082 | 2.432 | 0.124 |
| 250.0 | 0.57 | 93.73 | 2.429 | 2.445 | 0.659 | 2.429 | 0.000 | 2.431 | 0.082 |
| 260.0 | 0.59 | 97.48 | 2.426 | 2.445 | 0.783 | 2.428 | 0.082 | 2.429 | 0.124 |
| 270.0 | 0.61 | 101.23 | 2.427 | 2.445 | 0.742 | 2.427 | 0.000 | 2.428 | 0.041 |
| 280.0 | 0.64 | 104.98 | 2.426 | 2.444 | 0.742 | 2.426 | 0.000 | 2.427 | 0.041 |
| 290.0 | 0.66 | 108.73 | 2.423 | 2.444 | 0.867 | 2.424 | 0.041 | 2.426 | 0.124 |
| 300.0 | 0.68 | 112.48 | 2.424 | 2.443 | 0.784 | 2.423 | 0.041 | 2.425 | 0.041 |
| 310.0 | 0.70 | 116.23 | 2.424 | 2.443 | 0.784 | 2.422 | 0.083 | 2.424 | 0.000 |
| 320.0 | 0.73 | 119.97 | 2.421 | 2.442 | 0.867 | 2.421 | 0.000 | 2.423 | 0.083 |
| 330.0 | 0.75 | 123.72 | 2.421 | 2.441 | 0.826 | 2.420 | 0.041 | 2.422 | 0.041 |
| 340.0 | 0.77 | 127.47 | 2.421 | 2.441 | 0.826 | 2.418 | 0.124 | 2.421 | 0.000 |
| 350.0 | 0.80 | 131.22 | 2.419 | 2.440 | 0.868 | 2.417 | 0.083 | 2.420 | 0.041 |
| 360.0 | 0.82 | 134.97 | 2.418 | 2.439 | 0.868 | 2.416 | 0.083 | 2.419 | 0.041 |
| 370.0 | 0.84 | 138.72 | 2.417 | 2.439 | 0.910 | 2.415 | 0.083 | 2.418 | 0.041 |
| 380.0 | 0.86 | 142.47 | 2.417 | 2.438 | 0.869 | 2.414 | 0.124 | 2.417 | 0.000 |
| 390.0 | 0.89 | 146.22 | 2.416 | 2.437 | 0.869 | 2.413 | 0.124 | 2.416 | 0.000 |
| 400.0 | 0.91 | 149.97 | 2.415 | 2.437 | 0.911 | 2.412 | 0.124 | 2.415 | 0.000 |

**Table 3f.** Key properties of the pair correlation function resulting from Langevin dynamics simulations and three integral theory approaches: the hypernetted-chain approximation (HNC), isomorph-based empirically modified hypernetted-chain approximation (IEMHNC) and empirically modified hypernetted-chain approximation (EMHNC). The absolute relative deviation $\epsilon_{\mathrm{r}}$ between the theoretical and the simulation results is also reported. **Results for the magnitude of the second maximum in the case of $\boldsymbol{\kappa = 2}$**. The LD results are adopted from Table 6 of *T. Ott and M. Bonitz, Contrib. Plasma Phys.* **55**, *243 (2015)*.

| $\Gamma$ | $\Gamma/\Gamma_{\mathrm{m}}$ | $\Gamma_{\mathrm{iso}}^{\mathrm{OCP}}$ | $g_{\mathrm{max2}}^{\mathrm{LD}}$ | $g_{\mathrm{max2}}^{\mathrm{HNC}}$ | $\epsilon_{\mathrm{HNC}}(\%)$ | $g_{\mathrm{max2}}^{\mathrm{IEMHNC}}$ | $\epsilon_{\mathrm{IEMHNC}}(\%)$ | $g_{\mathrm{max2}}^{\mathrm{EMHNC}}$ | $\epsilon_{\mathrm{EMHNC}}(\%)$ |
|---|---|---|---|---|---|---|---|---|---|
| 30.0 | 0.07 | 11.25 | 1.008 | 1.005 | 0.304 | 1.007 | 0.126 | 1.009 | 0.062 |
| 40.0 | 0.09 | 15.00 | 1.016 | 1.009 | 0.642 | 1.013 | 0.270 | 1.016 | 0.047 |
| 50.0 | 0.11 | 18.75 | 1.025 | 1.015 | 0.994 | 1.021 | 0.381 | 1.026 | 0.060 |
| 60.0 | 0.14 | 22.50 | 1.034 | 1.021 | 1.292 | 1.030 | 0.399 | 1.036 | 0.148 |
| 70.0 | 0.16 | 26.24 | 1.044 | 1.027 | 1.650 | 1.039 | 0.456 | 1.046 | 0.187 |
| 80.0 | 0.18 | 29.99 | 1.054 | 1.033 | 1.983 | 1.049 | 0.480 | 1.057 | 0.255 |
| 90.0 | 0.20 | 33.74 | 1.064 | 1.040 | 2.300 | 1.059 | 0.487 | 1.068 | 0.340 |
| 100.0 | 0.23 | 37.49 | 1.074 | 1.046 | 2.606 | 1.069 | 0.486 | 1.079 | 0.433 |
| 110.0 | 0.25 | 41.24 | 1.084 | 1.053 | 2.904 | 1.079 | 0.483 | 1.090 | 0.528 |
| 120.0 | 0.27 | 44.99 | 1.093 | 1.059 | 3.110 | 1.089 | 0.391 | 1.101 | 0.714 |
| 130.0 | 0.30 | 48.74 | 1.103 | 1.065 | 3.403 | 1.099 | 0.396 | 1.112 | 0.803 |
| 140.0 | 0.32 | 52.49 | 1.113 | 1.072 | 3.694 | 1.108 | 0.407 | 1.123 | 0.886 |
| 150.0 | 0.34 | 56.24 | 1.122 | 1.078 | 3.899 | 1.118 | 0.338 | 1.134 | 1.050 |
| 160.0 | 0.36 | 59.99 | 1.131 | 1.085 | 4.106 | 1.128 | 0.278 | 1.145 | 1.203 |
| 170.0 | 0.39 | 63.74 | 1.140 | 1.091 | 4.315 | 1.137 | 0.229 | 1.155 | 1.345 |
| 180.0 | 0.41 | 67.49 | 1.149 | 1.097 | 4.527 | 1.147 | 0.191 | 1.166 | 1.475 |
| 190.0 | 0.43 | 71.23 | 1.158 | 1.103 | 4.742 | 1.156 | 0.164 | 1.176 | 1.592 |
| 200.0 | 0.45 | 74.98 | 1.165 | 1.109 | 4.797 | 1.165 | 0.024 | 1.187 | 1.870 |
| 210.0 | 0.48 | 78.73 | 1.173 | 1.115 | 4.938 | 1.174 | 0.113 | 1.197 | 2.047 |
| 220.0 | 0.50 | 82.48 | 1.181 | 1.121 | 5.084 | 1.183 | 0.191 | 1.207 | 2.209 |
| 230.0 | 0.52 | 86.23 | 1.189 | 1.127 | 5.234 | 1.192 | 0.256 | 1.217 | 2.357 |
| 240.0 | 0.55 | 89.98 | 1.196 | 1.133 | 5.309 | 1.201 | 0.394 | 1.227 | 2.576 |
| 250.0 | 0.57 | 93.73 | 1.204 | 1.138 | 5.468 | 1.209 | 0.436 | 1.236 | 2.694 |
| 260.0 | 0.59 | 97.48 | 1.210 | 1.144 | 5.475 | 1.218 | 0.633 | 1.246 | 2.968 |
| 270.0 | 0.61 | 101.23 | 1.217 | 1.149 | 5.565 | 1.226 | 0.734 | 1.255 | 3.142 |
| 280.0 | 0.64 | 104.98 | 1.224 | 1.155 | 5.661 | 1.234 | 0.825 | 1.264 | 3.301 |
| 290.0 | 0.66 | 108.73 | 1.230 | 1.160 | 5.684 | 1.242 | 0.985 | 1.273 | 3.529 |
| 300.0 | 0.68 | 112.48 | 1.236 | 1.165 | 5.713 | 1.250 | 1.134 | 1.282 | 3.742 |
| 310.0 | 0.70 | 116.23 | 1.243 | 1.171 | 5.823 | 1.258 | 1.189 | 1.291 | 3.857 |
| 320.0 | 0.73 | 119.97 | 1.248 | 1.176 | 5.786 | 1.265 | 1.396 | 1.299 | 4.124 |
| 330.0 | 0.75 | 123.72 | 1.254 | 1.181 | 5.830 | 1.273 | 1.511 | 1.308 | 4.294 |
| 340.0 | 0.77 | 127.47 | 1.259 | 1.186 | 5.805 | 1.280 | 1.695 | 1.316 | 4.531 |
| 350.0 | 0.80 | 131.22 | 1.264 | 1.191 | 5.784 | 1.288 | 1.868 | 1.324 | 4.755 |
| 360.0 | 0.82 | 134.97 | 1.270 | 1.196 | 5.844 | 1.295 | 1.950 | 1.332 | 4.882 |
| 370.0 | 0.84 | 138.72 | 1.275 | 1.201 | 5.833 | 1.302 | 2.102 | 1.340 | 5.077 |
| 380.0 | 0.86 | 142.47 | 1.279 | 1.205 | 5.754 | 1.309 | 2.323 | 1.347 | 5.342 |
| 390.0 | 0.89 | 146.22 | 1.283 | 1.210 | 5.680 | 1.315 | 2.533 | 1.355 | 5.592 |
| 400.0 | 0.91 | 149.97 | 1.288 | 1.215 | 5.685 | 1.322 | 2.653 | 1.362 | 5.747 |

**Table 3g.** Key properties of the pair correlation function resulting from Langevin dynamics simulations and three integral theory approaches: the hypernetted-chain approximation (HNC), isomorph-based empirically modified hypernetted-chain approximation (IEMHNC) and empirically modified hypernetted-chain approximation (EMHNC). The absolute relative deviation $\epsilon_{\mathrm{r}}$ between the theoretical and the simulation results is also reported. **Results for the position of the second maximum in the case of $\boldsymbol{\kappa} = \mathbf{2}$**. The LD results are adopted from Table 6 of *T. Ott and M. Bonitz, Contrib. Plasma Phys.* **55**, *243 (2015)*.

| $\Gamma$ | $\Gamma/\Gamma_{\mathrm{m}}$ | $\Gamma_{\mathrm{iso}}^{\mathrm{OCP}}$ | $r_{\mathrm{max2}}^{\mathrm{LD}}/d$ | $r_{\mathrm{max2}}^{\mathrm{HNC}}/d$ | $\epsilon_{\mathrm{HNC}}(\%)$ | $r_{\mathrm{max2}}^{\mathrm{IEMHNC}}/d$ | $\epsilon_{\mathrm{IEMHNC}}(\%)$ | $r_{\mathrm{max2}}^{\mathrm{EMHNC}}/d$ | $\epsilon_{\mathrm{EMHNC}}(\%)$ |
|---|---|---|---|---|---|---|---|---|---|
| 30.0 | 0.07 | 11.25 | 3.213 | 3.230 | 0.529 | 3.255 | 1.307 | 3.244 | 0.965 |
| 40.0 | 0.09 | 15.00 | 3.199 | 3.212 | 0.406 | 3.245 | 1.438 | 3.219 | 0.625 |
| 50.0 | 0.11 | 18.75 | 3.193 | 3.204 | 0.345 | 3.231 | 1.190 | 3.209 | 0.501 |
| 60.0 | 0.14 | 22.50 | 3.192 | 3.200 | 0.251 | 3.220 | 0.877 | 3.205 | 0.407 |
| 70.0 | 0.16 | 26.24 | 3.196 | 3.199 | 0.094 | 3.214 | 0.563 | 3.203 | 0.219 |
| 80.0 | 0.18 | 29.99 | 3.193 | 3.198 | 0.157 | 3.210 | 0.532 | 3.202 | 0.282 |
| 90.0 | 0.20 | 33.74 | 3.194 | 3.198 | 0.125 | 3.208 | 0.438 | 3.203 | 0.282 |
| 100.0 | 0.23 | 37.49 | 3.194 | 3.198 | 0.125 | 3.207 | 0.407 | 3.204 | 0.313 |
| 110.0 | 0.25 | 41.24 | 3.198 | 3.199 | 0.031 | 3.206 | 0.250 | 3.205 | 0.219 |
| 120.0 | 0.27 | 44.99 | 3.198 | 3.200 | 0.063 | 3.206 | 0.250 | 3.207 | 0.281 |
| 130.0 | 0.30 | 48.74 | 3.200 | 3.201 | 0.031 | 3.207 | 0.219 | 3.208 | 0.250 |
| 140.0 | 0.32 | 52.49 | 3.201 | 3.201 | 0.000 | 3.208 | 0.219 | 3.210 | 0.281 |
| 150.0 | 0.34 | 56.24 | 3.201 | 3.202 | 0.031 | 3.209 | 0.250 | 3.212 | 0.344 |
| 160.0 | 0.36 | 59.99 | 3.205 | 3.203 | 0.062 | 3.210 | 0.156 | 3.214 | 0.281 |
| 170.0 | 0.39 | 63.74 | 3.203 | 3.204 | 0.031 | 3.211 | 0.250 | 3.215 | 0.375 |
| 180.0 | 0.41 | 67.49 | 3.207 | 3.205 | 0.062 | 3.213 | 0.187 | 3.217 | 0.312 |
| 190.0 | 0.43 | 71.23 | 3.206 | 3.206 | 0.000 | 3.214 | 0.250 | 3.219 | 0.405 |
| 200.0 | 0.45 | 74.98 | 3.207 | 3.207 | 0.000 | 3.215 | 0.249 | 3.221 | 0.437 |
| 210.0 | 0.48 | 78.73 | 3.209 | 3.209 | 0.000 | 3.217 | 0.249 | 3.223 | 0.436 |
| 220.0 | 0.50 | 82.48 | 3.210 | 3.210 | 0.000 | 3.218 | 0.249 | 3.225 | 0.467 |
| 230.0 | 0.52 | 86.23 | 3.211 | 3.211 | 0.000 | 3.220 | 0.280 | 3.226 | 0.467 |
| 240.0 | 0.55 | 89.98 | 3.211 | 3.212 | 0.031 | 3.221 | 0.311 | 3.228 | 0.529 |
| 250.0 | 0.57 | 93.73 | 3.212 | 3.213 | 0.031 | 3.223 | 0.342 | 3.230 | 0.560 |
| 260.0 | 0.59 | 97.48 | 3.212 | 3.214 | 0.062 | 3.224 | 0.374 | 3.231 | 0.592 |
| 270.0 | 0.61 | 101.23 | 3.213 | 3.215 | 0.062 | 3.226 | 0.405 | 3.233 | 0.622 |
| 280.0 | 0.64 | 104.98 | 3.214 | 3.216 | 0.062 | 3.227 | 0.404 | 3.235 | 0.653 |
| 290.0 | 0.66 | 108.73 | 3.214 | 3.217 | 0.093 | 3.228 | 0.436 | 3.236 | 0.685 |
| 300.0 | 0.68 | 112.48 | 3.216 | 3.218 | 0.062 | 3.230 | 0.435 | 3.238 | 0.684 |
| 310.0 | 0.70 | 116.23 | 3.216 | 3.218 | 0.062 | 3.231 | 0.466 | 3.239 | 0.715 |
| 320.0 | 0.73 | 119.97 | 3.216 | 3.219 | 0.093 | 3.233 | 0.529 | 3.241 | 0.777 |
| 330.0 | 0.75 | 123.72 | 3.218 | 3.220 | 0.062 | 3.234 | 0.497 | 3.242 | 0.746 |
| 340.0 | 0.77 | 127.47 | 3.218 | 3.221 | 0.093 | 3.235 | 0.528 | 3.244 | 0.808 |
| 350.0 | 0.80 | 131.22 | 3.218 | 3.222 | 0.124 | 3.237 | 0.590 | 3.245 | 0.839 |
| 360.0 | 0.82 | 134.97 | 3.220 | 3.223 | 0.093 | 3.238 | 0.559 | 3.246 | 0.807 |
| 370.0 | 0.84 | 138.72 | 3.219 | 3.224 | 0.155 | 3.239 | 0.621 | 3.248 | 0.901 |
| 380.0 | 0.86 | 142.47 | 3.221 | 3.225 | 0.124 | 3.240 | 0.590 | 3.249 | 0.869 |
| 390.0 | 0.89 | 146.22 | 3.221 | 3.226 | 0.155 | 3.242 | 0.652 | 3.250 | 0.900 |
| 400.0 | 0.91 | 149.97 | 3.221 | 3.227 | 0.186 | 3.243 | 0.683 | 3.251 | 0.931 |

**Table 4.** The reduced excess internal energy due to particle-particle interactions $u_{\rm ex}^{\rm pp}$ resulting from molecular dynamics simulations and four integral theory approaches: the soft mean spherical approximation (SMSA), hypernetted-chain approximation (HNC), isomorph-based empirically modified hypernetted-chain approximation (IEMHNC) and empirically modified hypernetted-chain approximation (EMHNC). The absolute relative deviation $\epsilon_{\rm r}$ between the theoretical and the simulation results is also reported. **Results for very low screening parameters**, *i.e.* $\kappa = \{0.0, 0.2, 0.4, 0.6\}$. The MD results are adopted from Table II of *R. T. Farouki and S. Hamaguchi, J. Chem. Phys.* **101***, 9885 (1994)*. Owing to the well-known divergence, the reduced excess internal energy for the OCP includes interaction with the neutralizing background. It should be pointed out that for the OCP, the IEMHNC and EMHNC approaches are identical.

| $\Gamma$ | $\Gamma/\Gamma_{\rm m}$ | $\Gamma_{\rm iso}^{\rm OCP}$ | $u_{\rm ex}^{\rm pp,MD}$ | $u_{\rm ex}^{\rm pp,SMSA}$ | $\epsilon_{\rm r}^{\rm SMSA}(\%)$ | $u_{\rm ex}^{\rm pp,HNC}$ | $\epsilon_{\rm r}^{\rm HNC}(\%)$ | $u_{\rm ex}^{\rm pp,IEMHNC}$ | $\epsilon_{\rm r}^{\rm IEMHNC}(\%)$ | $u_{\rm ex}^{\rm pp,EMHNC}$ | $\epsilon_{\rm r}^{\rm EMHNC}(\%)$ |
|---|---|---|---|---|---|---|---|---|---|---|---|
| $\kappa = 0.0$ | | | | | | | | | | | |
| 10.0 | 0.06 | 10.0 | -7.995 | -8.053 | 0.716 | -7.935 | 0.750 | -7.963 | 0.400 | -7.963 | 0.400 |
| 20.0 | 0.12 | 20.0 | -16.668 | -16.667 | 0.005 | -16.538 | 0.782 | -16.639 | 0.177 | -16.639 | 0.177 |
| 40.0 | 0.23 | 40.0 | -34.259 | -34.125 | 0.394 | -33.999 | 0.759 | -34.221 | 0.111 | -34.221 | 0.111 |
| 60.0 | 0.35 | 60.0 | -51.957 | -51.710 | 0.478 | -51.597 | 0.692 | -51.925 | 0.061 | -51.925 | 0.061 |
| 80.0 | 0.47 | 80.0 | -69.725 | -69.360 | 0.526 | -69.264 | 0.661 | -69.690 | 0.051 | -69.690 | 0.051 |
| 100.0 | 0.58 | 100.0 | -87.519 | -87.053 | 0.536 | -86.974 | 0.623 | -87.486 | 0.038 | -87.486 | 0.038 |
| 120.0 | 0.70 | 120.0 | -105.343 | -104.775 | 0.542 | -104.715 | 0.596 | -105.284 | 0.056 | -105.284 | 0.056 |
| 140.0 | 0.81 | 140.0 | -123.175 | -122.520 | 0.535 | -122.478 | 0.565 | -123.046 | 0.105 | -123.046 | 0.105 |
| 160.0 | 0.93 | 160.0 | -141.698 | -140.282 | 1.009 | -140.256 | 1.017 | -140.727 | 0.685 | -140.727 | 0.685 |
| $\kappa = 0.2$ | | | | | | | | | | | |
| 10.0 | 0.06 | 9.96 | 367.955 | 367.900 | 0.015 | 368.018 | 0.017 | 367.990 | 0.009 | 367.990 | 0.009 |
| 20.0 | 0.12 | 19.91 | 735.243 | 735.243 | 0.000 | 735.373 | 0.018 | 735.272 | 0.004 | 735.272 | 0.004 |
| 40.0 | 0.23 | 39.82 | 1469.574 | 1469.701 | 0.009 | 1469.827 | 0.017 | 1469.605 | 0.002 | 1469.606 | 0.002 |
| 60.0 | 0.35 | 59.74 | 2203.783 | 2204.032 | 0.011 | 2204.145 | 0.016 | 2203.818 | 0.002 | 2203.819 | 0.002 |
| 80.0 | 0.46 | 79.65 | 2937.938 | 2938.298 | 0.012 | 2938.395 | 0.016 | 2937.970 | 0.001 | 2937.972 | 0.001 |
| 100.0 | 0.58 | 99.56 | 3672.056 | 3672.522 | 0.013 | 3672.602 | 0.015 | 3672.084 | 0.001 | 3672.086 | 0.001 |
| 120.0 | 0.69 | 119.47 | 4406.160 | 4406.717 | 0.013 | 4406.779 | 0.014 | 4406.171 | 0.000 | 4406.173 | 0.000 |
| 140.0 | 0.81 | 139.38 | 5140.234 | 5140.889 | 0.013 | 5140.934 | 0.014 | 5140.238 | 0.000 | 5140.241 | 0.000 |
| 160.0 | 0.92 | 159.30 | 5873.712 | 5875.043 | 0.023 | 5875.071 | 0.023 | 5874.292 | 0.010 | 5874.294 | 0.010 |
| $\kappa = 0.4$ | | | | | | | | | | | |
| 10.0 | 0.06 | 9.72 | 87.571 | 87.511 | 0.068 | 87.628 | 0.065 | 87.602 | 0.036 | 87.600 | 0.034 |
| 20.0 | 0.11 | 19.44 | 174.480 | 174.476 | 0.002 | 174.606 | 0.072 | 174.508 | 0.016 | 174.507 | 0.015 |
| 40.0 | 0.22 | 38.89 | 348.064 | 348.182 | 0.034 | 348.308 | 0.070 | 348.091 | 0.008 | 348.091 | 0.008 |
| 60.0 | 0.34 | 58.33 | 521.526 | 521.762 | 0.045 | 521.876 | 0.067 | 521.555 | 0.005 | 521.555 | 0.006 |
| 80.0 | 0.45 | 77.78 | 694.927 | 695.278 | 0.050 | 695.377 | 0.065 | 694.959 | 0.005 | 694.960 | 0.005 |
| 100.0 | 0.56 | 97.22 | 868.304 | 868.753 | 0.052 | 868.835 | 0.061 | 868.325 | 0.002 | 868.327 | 0.003 |
| 120.0 | 0.67 | 116.67 | 1041.667 | 1042.198 | 0.051 | 1042.264 | 0.057 | 1041.665 | 0.000 | 1041.666 | 0.000 |
| 140.0 | 0.78 | 136.11 | 1214.982 | 1215.622 | 0.053 | 1215.670 | 0.057 | 1214.985 | 0.000 | 1214.986 | 0.000 |
| 160.0 | 0.90 | 155.56 | 1387.654 | 1389.027 | 0.099 | 1389.059 | 0.101 | 1388.289 | 0.046 | 1388.290 | 0.046 |
| $\kappa = 0.6$ | | | | | | | | | | | |
| 10.0 | 0.05 | 9.26 | 36.262 | 36.198 | 0.175 | 36.314 | 0.144 | 36.292 | 0.083 | 36.287 | 0.071 |
| 20.0 | 0.11 | 18.51 | 71.877 | 71.869 | 0.010 | 71.998 | 0.169 | 71.906 | 0.040 | 71.902 | 0.036 |
| 40.0 | 0.21 | 37.03 | 142.878 | 142.991 | 0.079 | 143.118 | 0.168 | 142.910 | 0.022 | 142.907 | 0.020 |
| 60.0 | 0.32 | 55.54 | 213.769 | 213.991 | 0.104 | 214.107 | 0.158 | 213.798 | 0.013 | 213.795 | 0.012 |
| 80.0 | 0.43 | 74.05 | 284.608 | 284.927 | 0.112 | 285.029 | 0.148 | 284.627 | 0.007 | 284.624 | 0.006 |
| 100.0 | 0.53 | 92.56 | 355.406 | 355.824 | 0.117 | 355.910 | 0.142 | 355.420 | 0.004 | 355.415 | 0.003 |
| 120.0 | 0.64 | 111.08 | 426.172 | 426.691 | 0.122 | 426.761 | 0.138 | 426.186 | 0.003 | 426.180 | 0.002 |
| 140.0 | 0.75 | 129.59 | 496.928 | 497.537 | 0.123 | 497.591 | 0.133 | 496.932 | 0.001 | 496.926 | 0.000 |
| 160.0 | 0.86 | 148.10 | 567.668 | 568.367 | 0.123 | 568.404 | 0.130 | 567.663 | 0.001 | 567.656 | 0.002 |
| 180.0 | 0.96 | 166.61 | 637.721 | 639.182 | 0.229 | 639.202 | 0.232 | 638.382 | 0.104 | 638.373 | 0.102 |

**Table 5.** The reduced excess internal energy due to particle-particle interactions $u_{\rm ex}^{\rm pp}$ resulting from molecular dynamics simulations and four integral theory approaches: the soft mean spherical approximation (SMSA), hypernetted-chain approximation (HNC), isomorph-based empirically modified hypernetted-chain approximation (IEMHNC) and empirically modified hypernetted-chain approximation (EMHNC). The absolute relative deviation $\epsilon_{\rm r}$ between the theoretical and the simulation results is also reported. **Results for low screening parameters**, *i.e.* $\kappa = \{0.8, 1.0, 1.2\}$. The MD results are adopted from Table II of *R. T. Farouki and S. Hamaguchi, J. Chem. Phys.* **101**, *9885 (1994)* and from Table II of *S. Hamaguchi, R. T. Farouki and D. H. E. Dubin, J. Chem. Phys.* **105**, *7641 (1996)*.

| $\Gamma$ | $\Gamma/\Gamma_{\rm m}$ | $\Gamma_{\rm iso}^{\rm OCP}$ | $u_{\rm ex}^{\rm pp,MD}$ | $u_{\rm ex}^{\rm pp,SMSA}$ | $\epsilon_{\rm r}^{\rm SMSA}(\%)$ | $u_{\rm ex}^{\rm pp,HNC}$ | $\epsilon_{\rm r}^{\rm HNC}(\%)$ | $u_{\rm ex}^{\rm pp,IEMHNC}$ | $\epsilon_{\rm r}^{\rm IEMHNC}(\%)$ | $u_{\rm ex}^{\rm pp,EMHNC}$ | $\epsilon_{\rm r}^{\rm EMHNC}(\%)$ |
|---|---|---|---|---|---|---|---|---|---|---|---|
| | | | | | $\kappa = 0.8$ | | | | | | |
| 10.0 | 0.05 | 8.60 | 18.718 | 18.653 | 0.349 | 18.767 | 0.260 | 18.751 | 0.172 | 18.741 | 0.124 |
| 20.0 | 0.10 | 17.19 | 36.821 | 36.804 | 0.048 | 36.932 | 0.300 | 36.848 | 0.072 | 36.840 | 0.050 |
| 40.0 | 0.20 | 34.38 | 72.801 | 72.892 | 0.124 | 73.020 | 0.300 | 72.826 | 0.033 | 72.817 | 0.021 |
| 60.0 | 0.30 | 51.57 | 108.666 | 108.861 | 0.179 | 108.979 | 0.288 | 108.690 | 0.022 | 108.680 | 0.013 |
| 80.0 | 0.40 | 68.76 | 144.482 | 144.770 | 0.199 | 144.875 | 0.272 | 144.497 | 0.011 | 144.486 | 0.003 |
| 100.0 | 0.50 | 85.95 | 180.249 | 180.639 | 0.216 | 180.730 | 0.267 | 180.269 | 0.011 | 180.255 | 0.003 |
| 120.0 | 0.60 | 103.14 | 216.011 | 216.481 | 0.217 | 216.557 | 0.253 | 216.015 | 0.002 | 215.998 | 0.006 |
| 140.0 | 0.70 | 120.33 | 251.747 | 252.302 | 0.220 | 252.362 | 0.244 | 251.742 | 0.002 | 251.722 | 0.010 |
| 160.0 | 0.80 | 137.52 | 287.472 | 288.106 | 0.220 | 288.151 | 0.236 | 287.454 | 0.006 | 287.431 | 0.014 |
| 180.0 | 0.90 | 154.71 | 322.564 | 323.897 | 0.412 | 323.926 | 0.422 | 323.154 | 0.183 | 323.129 | 0.175 |
| | | | | | $\kappa = 1.0$ | | | | | | |
| 10.0 | 0.05 | 7.80 | 10.890 | 10.818 | 0.659 | 10.930 | 0.366 | 10.920 | 0.278 | 10.906 | 0.146 |
| 20.0 | 0.09 | 15.61 | 21.194 | 21.163 | 0.146 | 21.290 | 0.454 | 21.217 | 0.109 | 21.203 | 0.042 |
| 40.0 | 0.18 | 31.21 | 41.575 | 41.650 | 0.180 | 41.779 | 0.491 | 41.602 | 0.066 | 41.586 | 0.028 |
| 60.0 | 0.28 | 46.82 | 61.854 | 62.022 | 0.271 | 62.143 | 0.467 | 61.877 | 0.037 | 61.859 | 0.008 |
| 80.0 | 0.37 | 62.42 | 82.074 | 82.336 | 0.319 | 82.445 | 0.453 | 82.098 | 0.030 | 82.076 | 0.003 |
| 100.0 | 0.46 | 78.03 | 102.265 | 102.613 | 0.339 | 102.709 | 0.434 | 102.284 | 0.019 | 102.258 | 0.006 |
| 120.0 | 0.55 | 93.63 | 122.429 | 122.862 | 0.353 | 122.945 | 0.422 | 122.446 | 0.014 | 122.415 | 0.011 |
| 140.0 | 0.64 | 109.24 | 142.582 | 143.092 | 0.357 | 143.161 | 0.406 | 142.589 | 0.005 | 142.553 | 0.020 |
| 160.0 | 0.74 | 124.84 | 162.715 | 163.306 | 0.362 | 163.360 | 0.396 | 162.717 | 0.001 | 162.677 | 0.023 |
| 180.0 | 0.83 | 140.45 | 182.839 | 183.507 | 0.364 | 183.546 | 0.387 | 182.834 | 0.002 | 182.789 | 0.027 |
| 200.0 | 0.92 | 156.05 | 202.358 | 203.697 | 0.657 | 203.722 | 0.674 | 202.941 | 0.288 | 202.891 | 0.263 |
| | | | | | $\kappa = 1.2$ | | | | | | |
| 10.0 | 0.04 | 6.94 | 6.831 | 6.762 | 1.018 | 6.870 | 0.574 | 6.867 | 0.522 | 6.848 | 0.248 |
| 20.0 | 0.08 | 13.89 | 13.124 | 13.084 | 0.303 | 13.209 | 0.653 | 13.149 | 0.191 | 13.128 | 0.034 |
| 40.0 | 0.16 | 27.78 | 25.485 | 25.535 | 0.194 | 25.665 | 0.704 | 25.508 | 0.090 | 25.485 | 0.001 |
| 60.0 | 0.25 | 41.67 | 37.734 | 37.877 | 0.379 | 38.001 | 0.708 | 37.762 | 0.074 | 37.735 | 0.004 |
| 80.0 | 0.33 | 55.55 | 49.942 | 50.164 | 0.442 | 50.278 | 0.672 | 49.964 | 0.043 | 49.933 | 0.019 |
| 100.0 | 0.41 | 69.44 | 62.098 | 62.416 | 0.508 | 62.518 | 0.675 | 62.133 | 0.056 | 62.096 | 0.004 |
| 120.0 | 0.49 | 83.33 | 74.273 | 74.641 | 0.494 | 74.731 | 0.617 | 74.279 | 0.008 | 74.235 | 0.050 |
| 140.0 | 0.58 | 97.22 | 86.398 | 86.848 | 0.518 | 86.925 | 0.610 | 86.407 | 0.010 | 86.357 | 0.048 |
| 160.0 | 0.66 | 111.11 | 98.520 | 99.040 | 0.525 | 99.104 | 0.593 | 98.521 | 0.002 | 98.464 | 0.057 |
| 180.0 | 0.74 | 125.00 | 110.606 | 111.219 | 0.551 | 111.270 | 0.600 | 110.624 | 0.016 | 110.559 | 0.042 |
| 200.0 | 0.82 | 138.89 | 122.732 | 123.388 | 0.531 | 123.426 | 0.565 | 122.718 | 0.012 | 122.646 | 0.070 |

**Table 6.** The reduced excess internal energy due to particle-particle interactions $u_{\rm ex}^{\rm pp}$ resulting from molecular dynamics simulations and four integral theory approaches: the soft mean spherical approximation (SMSA), hypernetted-chain approximation (HNC), isomorph-based empirically modified hypernetted-chain approximation (IEMHNC) and empirically modified hypernetted-chain approximation (EMHNC). The absolute relative deviation $\epsilon_{\rm r}$ between the theoretical and the simulation results is also reported. **Results for intermediate screening parameters**, *i.e.* $\kappa = \{1.4,\, 2.0,\, 2.6,\, 3.0\}$. The MD results are adopted from Table III of *S. Hamaguchi, R. T. Farouki, D. H. E. Dubin, Phys. Rev. E* **56**, *4671 (1997)* and from Table II of *S. Hamaguchi, R. T. Farouki and D. H. E. Dubin, J. Chem. Phys.* **105**, *7641 (1996)*.

| $\Gamma$ | $\Gamma/\Gamma_{\rm m}$ | $\Gamma_{\rm iso}^{\rm OCP}$ | $u_{\rm ex}^{\rm pp,MD}$ | $u_{\rm ex}^{\rm pp,SMSA}$ | $\epsilon_{\rm r}^{\rm SMSA}(\%)$ | $u_{\rm ex}^{\rm pp,HNC}$ | $\epsilon_{\rm r}^{\rm HNC}(\%)$ | $u_{\rm ex}^{\rm pp,IEMHNC}$ | $\epsilon_{\rm r}^{\rm IEMHNC}(\%)$ | $u_{\rm ex}^{\rm pp,EMHNC}$ | $\epsilon_{\rm r}^{\rm EMHNC}(\%)$ |
|---|---|---|---|---|---|---|---|---|---|---|---|
| $\kappa = 1.4$ | | | | | | | | | | | |
| 10.0 | 0.04 | 6.08 | 4.533 | 4.457 | 1.704 | 4.561 | 0.623 | 4.561 | 0.618 | 4.541 | 0.178 |
| 20.0 | 0.07 | 12.15 | 8.564 | 8.509 | 0.651 | 8.632 | 0.787 | 8.585 | 0.239 | 8.557 | 0.081 |
| 40.0 | 0.15 | 24.30 | 16.406 | 16.431 | 0.152 | 16.561 | 0.944 | 16.427 | 0.123 | 16.396 | 0.062 |
| 60.0 | 0.22 | 36.45 | 24.153 | 24.252 | 0.410 | 24.378 | 0.932 | 24.168 | 0.062 | 24.134 | 0.080 |
| 80.0 | 0.30 | 48.60 | 31.853 | 32.021 | 0.524 | 32.138 | 0.896 | 31.860 | 0.022 | 31.820 | 0.103 |
| 100.0 | 0.37 | 60.75 | 39.498 | 39.756 | 0.647 | 39.864 | 0.925 | 39.521 | 0.058 | 39.475 | 0.060 |
| 120.0 | 0.45 | 72.90 | 47.135 | 47.467 | 0.698 | 47.564 | 0.910 | 47.160 | 0.054 | 47.106 | 0.062 |
| 140.0 | 0.52 | 85.05 | 54.771 | 55.159 | 0.705 | 55.246 | 0.867 | 54.783 | 0.023 | 54.720 | 0.092 |
| 160.0 | 0.60 | 97.20 | 62.374 | 62.838 | 0.739 | 62.913 | 0.864 | 62.392 | 0.029 | 62.321 | 0.085 |
| 180.0 | 0.67 | 109.36 | 69.991 | 70.505 | 0.729 | 70.568 | 0.824 | 69.991 | 0.000 | 69.911 | 0.115 |
| 200.0 | 0.74 | 121.51 | 77.564 | 78.162 | 0.765 | 78.213 | 0.836 | 77.580 | 0.021 | 77.491 | 0.094 |
| 240.0 | 0.89 | 145.81 | 92.744 | 93.452 | 0.758 | 93.479 | 0.793 | 92.738 | 0.006 | 92.631 | 0.121 |
| $\kappa = 2.0$ | | | | | | | | | | | |
| 20.0 | 0.05 | 7.50 | 2.944 | 2.872 | 2.513 | 2.983 | 1.316 | 2.976 | 1.083 | 2.933 | 0.390 |
| 40.0 | 0.09 | 15.00 | 5.343 | 5.305 | 0.726 | 5.430 | 1.626 | 5.361 | 0.332 | 5.316 | 0.510 |
| 60.0 | 0.14 | 22.50 | 7.630 | 7.657 | 0.358 | 7.785 | 2.036 | 7.662 | 0.420 | 7.614 | 0.211 |
| 80.0 | 0.18 | 29.99 | 9.903 | 9.969 | 0.660 | 10.095 | 1.936 | 9.923 | 0.196 | 9.870 | 0.335 |
| 100.0 | 0.23 | 37.49 | 12.133 | 12.254 | 0.984 | 12.376 | 1.997 | 12.158 | 0.201 | 12.099 | 0.281 |
| 200.0 | 0.45 | 74.98 | 23.107 | 23.466 | 1.530 | 23.554 | 1.936 | 23.137 | 0.132 | 23.034 | 0.316 |
| $\kappa = 2.6$ | | | | | | | | | | | |
| 40.0 | 0.05 | 8.46 | 2.165 | 2.103 | 2.969 | 2.216 | 2.328 | 2.202 | 1.686 | 2.151 | 0.653 |
| 60.0 | 0.08 | 12.68 | 2.986 | 2.941 | 1.513 | 3.062 | 2.548 | 3.012 | 0.888 | 2.963 | 0.772 |
| 80.0 | 0.11 | 16.91 | 3.772 | 3.749 | 0.595 | 3.873 | 2.688 | 3.791 | 0.513 | 3.741 | 0.814 |
| 100.0 | 0.13 | 21.14 | 4.528 | 4.538 | 0.227 | 4.662 | 2.973 | 4.550 | 0.491 | 4.498 | 0.649 |
| 200.0 | 0.26 | 42.28 | 8.181 | 8.325 | 1.734 | 8.438 | 3.142 | 8.194 | 0.156 | 8.121 | 0.739 |
| 400.0 | 0.53 | 84.56 | 15.147 | 15.561 | 2.662 | 15.630 | 3.195 | 15.167 | 0.133 | 15.015 | 0.871 |
| 700.0 | 0.92 | 147.99 | 25.319 | 26.082 | 2.925 | 26.080 | 3.008 | 25.322 | 0.013 | 25.047 | 1.072 |
| $\kappa = 3.0$ | | | | | | | | | | | |
| 40.0 | 0.03 | 5.57 | 1.322 | 1.244 | 6.254 | 1.345 | 1.792 | 1.345 | 1.792 | 1.306 | 1.155 |
| 60.0 | 0.05 | 8.35 | 1.769 | 1.699 | 4.124 | 1.810 | 2.321 | 1.798 | 1.615 | 1.749 | 1.119 |
| 80.0 | 0.07 | 11.13 | 2.189 | 2.130 | 2.757 | 2.247 | 2.636 | 2.211 | 1.004 | 2.165 | 1.114 |
| 100.0 | 0.08 | 13.92 | 2.582 | 2.547 | 1.369 | 2.666 | 3.274 | 2.608 | 1.034 | 2.563 | 0.712 |
| 200.0 | 0.17 | 27.83 | 4.456 | 4.506 | 1.121 | 4.625 | 3.801 | 4.470 | 0.322 | 4.420 | 0.787 |
| 400.0 | 0.34 | 55.67 | 7.928 | 8.157 | 2.812 | 8.253 | 4.097 | 7.938 | 0.122 | 7.846 | 1.030 |
| 700.0 | 0.59 | 97.41 | 12.869 | 13.371 | 3.753 | 13.420 | 4.280 | 12.897 | 0.212 | 12.716 | 1.191 |

**Table 7.** The reduced excess internal energy due to particle-particle interactions $u_{\rm ex}^{\rm pp}$ resulting from molecular dynamics simulations and four integral theory approaches: the soft mean spherical approximation (SMSA), hypernetted-chain approximation (HNC), isomorph-based empirically modified hypernetted-chain approximation (IEMHNC) and empirically modified hypernetted-chain approximation (EMHNC). The absolute relative deviation $\epsilon_{\rm r}$ between the theoretical and the simulation results is also reported. **Results for high screening parameters**, *i.e.* $\kappa = \{3.6, 4.0, 4.6, 5.0\}$. The MD results are adopted from Table III of *S. Hamaguchi, R. T. Farouki, D. H. E. Dubin, Phys. Rev. E* **56**, *4671 (1997)*.

| $\Gamma$ | $\Gamma/\Gamma_{\rm m}$ | $\Gamma_{\rm iso}^{\rm OCP}$ | $u_{\rm ex}^{\rm pp,MD}$ | $u_{\rm ex}^{\rm pp,SMSA}$ | $\epsilon_{\rm r}^{\rm SMSA}(\%)$ | $u_{\rm ex}^{\rm pp,HNC}$ | $\epsilon_{\rm r}^{\rm HNC}(\%)$ | $u_{\rm ex}^{\rm pp,IEMHNC}$ | $\epsilon_{\rm r}^{\rm IEMHNC}(\%)$ | $u_{\rm ex}^{\rm pp,EMHNC}$ | $\epsilon_{\rm r}^{\rm EMHNC}(\%)$ |
|---|---|---|---|---|---|---|---|---|---|---|---|
| $\kappa = 3.6$ | | | | | | | | | | | |
| 80.0 | 0.03 | 5.71 | 1.092 | 1.026 | 6.442 | 1.126 | 3.159 | 1.126 | 3.160 | 1.093 | 0.129 |
| 100.0 | 0.04 | 7.13 | 1.272 | 1.202 | 5.750 | 1.308 | 2.844 | 1.304 | 2.574 | 1.266 | 0.465 |
| 200.0 | 0.08 | 14.27 | 2.035 | 2.004 | 1.523 | 2.119 | 4.158 | 2.062 | 1.317 | 2.032 | 0.126 |
| 400.0 | 0.17 | 28.54 | 3.378 | 3.429 | 1.478 | 3.541 | 4.821 | 3.386 | 0.240 | 3.361 | 0.520 |
| 700.0 | 0.29 | 49.94 | 5.200 | 5.389 | 3.514 | 5.483 | 5.442 | 5.205 | 0.088 | 5.157 | 0.835 |
| 1000.0 | 0.42 | 71.35 | 6.934 | 7.250 | 4.356 | 7.320 | 5.568 | 6.930 | 0.049 | 6.846 | 1.262 |
| 2000.0 | 0.84 | 142.70 | 12.399 | 13.122 | 5.503 | 13.108 | 5.715 | 12.382 | 0.143 | 12.188 | 1.705 |
| $\kappa = 4.0$ | | | | | | | | | | | |
| 200.0 | 0.05 | 8.94 | 1.305 | 1.253 | 4.133 | 1.360 | 4.239 | 1.345 | 3.043 | 1.317 | 0.930 |
| 400.0 | 0.10 | 17.89 | 2.066 | 2.060 | 0.251 | 2.173 | 5.183 | 2.091 | 1.243 | 2.081 | 0.751 |
| 700.0 | 0.18 | 31.30 | 3.054 | 3.139 | 2.699 | 3.245 | 6.237 | 3.077 | 0.741 | 3.075 | 0.684 |
| 1000.0 | 0.26 | 44.72 | 3.971 | 4.142 | 4.123 | 4.236 | 6.664 | 3.991 | 0.497 | 3.984 | 0.331 |
| 2000.0 | 0.52 | 89.44 | 6.824 | 7.238 | 5.719 | 7.282 | 6.710 | 6.810 | 0.209 | 6.757 | 0.975 |
| $\kappa = 4.6$ | | | | | | | | | | | |
| 400.0 | 0.05 | 8.65 | 1.114 | 1.058 | 5.313 | 1.161 | 4.188 | 1.148 | 3.072 | 1.134 | 1.775 |
| 700.0 | 0.08 | 15.13 | 1.553 | 1.538 | 0.983 | 1.645 | 5.900 | 1.586 | 2.117 | 1.594 | 2.618 |
| 1000.0 | 0.12 | 21.62 | 1.947 | 1.969 | 1.110 | 2.075 | 6.527 | 1.973 | 1.301 | 1.997 | 2.563 |
| 2000.0 | 0.23 | 43.24 | 3.119 | 3.250 | 4.040 | 3.338 | 7.037 | 3.110 | 0.290 | 3.165 | 1.480 |
| 3000.0 | 0.35 | 64.85 | 4.126 | 4.412 | 6.471 | 4.477 | 8.497 | 4.136 | 0.239 | 4.204 | 1.870 |
| 4000.0 | 0.46 | 86.47 | 5.118 | 5.510 | 7.122 | 5.551 | 8.460 | 5.104 | 0.262 | 5.180 | 1.220 |
| 5000.0 | 0.58 | 108.09 | 6.047 | 6.568 | 7.923 | 6.583 | 8.861 | 6.035 | 0.204 | 6.122 | 1.241 |
| 6000.0 | 0.70 | 129.71 | 6.969 | 7.596 | 8.251 | 7.586 | 8.858 | 6.939 | 0.429 | 7.044 | 1.073 |
| $\kappa = 5.0$ | | | | | | | | | | | |
| 700.0 | 0.05 | 9.19 | 1.067 | 1.016 | 5.024 | 1.117 | 4.675 | 1.101 | 3.211 | 1.097 | 2.809 |
| 1000.0 | 0.07 | 13.12 | 1.295 | 1.276 | 1.483 | 1.379 | 6.501 | 1.336 | 3.175 | 1.349 | 4.159 |
| 2000.0 | 0.13 | 26.25 | 1.978 | 2.028 | 2.444 | 2.126 | 7.487 | 1.999 | 1.073 | 2.056 | 3.960 |
| 3000.0 | 0.20 | 39.37 | 2.568 | 2.691 | 4.587 | 2.779 | 8.219 | 2.577 | 0.360 | 2.666 | 3.802 |
| 4000.0 | 0.27 | 52.50 | 3.108 | 3.309 | 6.077 | 3.384 | 8.866 | 3.112 | 0.141 | 3.225 | 3.758 |
| 5000.0 | 0.33 | 65.62 | 3.625 | 3.897 | 6.972 | 3.957 | 9.160 | 3.620 | 0.140 | 3.753 | 3.530 |
| 6000.0 | 0.40 | 78.75 | 4.140 | 4.463 | 7.231 | 4.509 | 8.902 | 4.108 | 0.783 | 4.260 | 2.902 |
| 8000.0 | 0.53 | 105.00 | 5.072 | 5.549 | 8.589 | 5.565 | 9.717 | 5.041 | 0.620 | 5.234 | 3.186 |
| 10000.0 | 0.66 | 131.25 | 5.900 | 6.590 | 10.480 | 6.577 | 11.481 | 5.934 | 0.571 | 6.173 | 4.632 |

**Table 8.** The reduced excess pressure due to particle-particle interactions $p_{\mathrm{ex}}^{\mathrm{pp}}$ resulting from Monte Carlo simulations and from five integral theory approaches: the soft mean spherical approximation (SMSA), hypernetted-chain approximation (HNC), discretized Rogers-Young approximation (DRY), isomorph-based empirically modified hypernetted-chain approximation (IEMHNC) and empirically modified hypernetted-chain approximation (EMHNC). The absolute relative deviation $\epsilon_{\mathrm{r}}$ between the theoretical and the simulation results is reported. The MC and DRY results are adopted from Table I of *C. F. Tejero, J. F. Lutsko, J. L. Colot, M. Baus, Phys. Rev. A* **46**, *3373 (1992)*. The corresponding OCP coupling parameters resulting from the isomorph mapping are also provided.

| $\kappa$ | $\Gamma$ | $\Gamma_{\mathrm{iso}}^{\mathrm{OCP}}$ | $p_{\mathrm{ex}}^{\mathrm{pp,MC}}$ | $p_{\mathrm{ex}}^{\mathrm{pp,SMSA}}$ | $\epsilon_{\mathrm{r}}^{\mathrm{SMSA}}(\%)$ | $p_{\mathrm{ex}}^{\mathrm{pp,HNC}}$ | $\epsilon_{\mathrm{r}}^{\mathrm{HNC}}(\%)$ | $p_{\mathrm{ex}}^{\mathrm{pp,DRY}}$ | $\epsilon_{\mathrm{r}}^{\mathrm{DRY}}(\%)$ | $p_{\mathrm{ex}}^{\mathrm{pp,IEMHNC}}$ | $\epsilon_{\mathrm{r}}^{\mathrm{IEMHNC}}(\%)$ | $p_{\mathrm{ex}}^{\mathrm{pp,EMHNC}}$ | $\epsilon_{\mathrm{r}}^{\mathrm{EMHNC}}(\%)$ |
|---|---|---|---|---|---|---|---|---|---|---|---|---|---|
| 1.800 | 396.9 | 176.86 | 101.492 | 102.198 | 0.691 | 102.131 | 0.630 | 101.751 | 0.255 | 101.406 | 0.085 | 101.232 | 0.256 |
| 1.860 | 383.9 | 162.61 | 88.606 | 89.225 | 0.694 | 89.289 | 0.770 | 88.846 | 0.271 | 88.590 | 0.018 | 88.415 | 0.216 |
| 1.923 | 371.4 | 149.00 | 77.148 | 77.787 | 0.821 | 77.809 | 0.856 | 77.387 | 0.310 | 77.137 | 0.014 | 76.961 | 0.242 |
| 1.984 | 360.0 | 136.90 | 67.640 | 68.262 | 0.911 | 68.265 | 0.925 | 67.865 | 0.333 | 67.620 | 0.030 | 67.444 | 0.290 |
| 2.049 | 348.6 | 125.09 | 58.889 | 59.501 | 1.029 | 59.537 | 1.100 | 59.091 | 0.343 | 58.919 | 0.051 | 58.745 | 0.245 |
| 2.117 | 337.5 | 113.84 | 51.133 | 51.732 | 1.158 | 51.752 | 1.211 | 51.307 | 0.340 | 51.162 | 0.057 | 50.991 | 0.277 |
| 2.182 | 327.3 | 103.97 | 44.711 | 45.265 | 1.224 | 45.348 | 1.425 | 44.862 | 0.338 | 44.784 | 0.164 | 44.618 | 0.208 |
| 2.238 | 319.2 | 96.21 | 40.041 | 40.539 | 1.228 | 40.574 | 1.331 | 40.176 | 0.337 | 40.033 | 0.021 | 39.871 | 0.425 |
| 2.306 | 309.7 | 87.50 | 34.954 | 35.412 | 1.293 | 35.509 | 1.589 | 35.072 | 0.338 | 34.995 | 0.117 | 34.840 | 0.327 |
| 2.348 | 304.2 | 82.54 | 32.204 | 32.675 | 1.441 | 32.753 | 1.704 | 32.314 | 0.342 | 32.255 | 0.157 | 32.104 | 0.312 |
| 2.398 | 297.9 | 77.00 | 29.294 | 29.718 | 1.427 | 29.785 | 1.676 | 29.394 | 0.341 | 29.306 | 0.040 | 29.160 | 0.456 |
| 2.532 | 282.1 | 63.87 | 22.780 | 23.144 | 1.573 | 23.230 | 1.973 | 22.855 | 0.329 | 22.801 | 0.090 | 22.672 | 0.476 |
| 2.631 | 271.5 | 55.62 | 19.016 | 19.341 | 1.680 | 19.450 | 2.283 | 19.069 | 0.279 | 19.057 | 0.215 | 18.941 | 0.396 |
| 2.778 | 257.1 | 45.26 | 14.705 | 14.952 | 1.652 | 15.077 | 2.530 | 14.722 | 0.116 | 14.736 | 0.208 | 14.638 | 0.457 |
| 3.050 | 234.2 | 30.88 | 9.400 | 9.444 | 0.466 | 9.688 | 3.061 | 9.343 | 0.606 | 9.437 | 0.391 | 9.368 | 0.344 |

**Table 9a.** Test of the thermodynamic consistency of the isomorph-based empirically modified hypernetted-chain approximation (IEMHNC) and the empirically modified hypernetted-chain approximation (EMHNC); the reduced excess inverse isothermal compressibility due to the particle presence resulting from the statistical route $\mu_{\mathrm{stat}}^{\mathrm{p}}$ and the virial route $\mu_{\mathrm{vir}}^{\mathrm{p}}$. The absolute relative deviation between the two thermodynamic paths is also reported. **Results for $\boldsymbol{\kappa = 0}$**. It should be pointed out that for the OCP, the IEMHNC and the EMHNC approaches are identical.

| $\Gamma$ | $\Gamma/\Gamma_{\mathrm{m}}$ | $\Gamma_{\mathrm{iso}}^{\mathrm{OCP}}$ | $\mu_{\mathrm{stat}}^{\mathrm{p,IEMHNC}}$ | $\mu_{\mathrm{vir}}^{\mathrm{p,IEMHNC}}$ | deviation (%) | $\mu_{\mathrm{stat}}^{\mathrm{p,EMHNC}}$ | $\mu_{\mathrm{vir}}^{\mathrm{p,EMHNC}}$ | deviation (%) |
|---|---|---|---|---|---|---|---|---|
| 10 | 0.06 | 10 | -4.04661 | -3.60863 | 12.137 | -4.04661 | -3.60863 | 12.137 |
| 20 | 0.12 | 20 | -7.28883 | -7.48721 | 2.6497 | -7.28883 | -7.48721 | 2.6497 |
| 30 | 0.17 | 30 | -10.8499 | -11.4009 | 4.8330 | -10.8499 | -11.4009 | 4.8330 |
| 40 | 0.23 | 40 | -14.8044 | -15.3316 | 3.4382 | -14.8044 | -15.3316 | 3.4382 |
| 50 | 0.29 | 50 | -19.0180 | -19.2728 | 1.3224 | -19.0180 | -19.2728 | 1.3224 |
| 60 | 0.35 | 60 | -23.4073 | -23.2216 | 0.7997 | -23.4073 | -23.2216 | 0.7997 |
| 70 | 0.41 | 70 | -27.9246 | -27.1761 | 2.7543 | -27.9246 | -27.1761 | 2.7543 |
| 80 | 0.47 | 80 | -32.5401 | -31.1342 | 4.5156 | -32.5401 | -31.1342 | 4.5156 |
| 90 | 0.52 | 90 | -37.2348 | -35.0939 | 6.1002 | -37.2348 | -35.0939 | 6.1002 |
| 100 | 0.58 | 100 | -41.9950 | -39.0525 | 7.5347 | -41.9950 | -39.0525 | 7.5347 |
| 110 | 0.64 | 110 | -46.8111 | -43.0067 | 8.8462 | -46.8111 | -43.0067 | 8.8462 |
| 120 | 0.70 | 120 | -51.6756 | -46.9526 | 10.059 | -51.6756 | -46.9526 | 10.059 |
| 130 | 0.76 | 130 | -56.5826 | -50.8864 | 11.194 | -56.5826 | -50.8864 | 11.194 |
| 140 | 0.81 | 140 | -61.5276 | -54.8043 | 12.268 | -61.5276 | -54.8043 | 12.268 |
| 150 | 0.87 | 150 | -66.5065 | -58.7026 | 13.294 | -66.5065 | -58.7026 | 13.294 |
| 160 | 0.93 | 160 | -71.5163 | -62.5785 | 14.282 | -71.5163 | -62.5785 | 14.282 |
| 170 | 0.99 | 170 | -76.5540 | -66.4300 | 15.240 | -76.5540 | -66.4300 | 15.240 |

**Table 9b.** Test of the thermodynamic consistency of the isomorph-based empirically modified hypernetted-chain approximation (IEMHNC) and the empirically modified hypernetted-chain approximation (EMHNC); the reduced excess inverse isothermal compressibility due to the particle presence resulting from the statistical route $\mu_{\mathrm{stat}}^{\mathrm{p}}$ and the virial route $\mu_{\mathrm{vir}}^{\mathrm{p}}$. The absolute relative deviation between the two thermodynamic paths is also reported. **Results for $\boldsymbol{\kappa = 0.2}$**.

| $\Gamma$ | $\Gamma/\Gamma_{\mathrm{m}}$ | $\Gamma_{\mathrm{iso}}^{\mathrm{OCP}}$ | $\mu_{\mathrm{stat}}^{\mathrm{p,IEMHNC}}$ | $\mu_{\mathrm{vir}}^{\mathrm{p,IEMHNC}}$ | deviation (%) | $\mu_{\mathrm{stat}}^{\mathrm{p,EMHNC}}$ | $\mu_{\mathrm{vir}}^{\mathrm{p,EMHNC}}$ | deviation (%) |
|---|---|---|---|---|---|---|---|---|
| 10 | 0.06 | 9.96 | -4.02536 | -3.59581 | 11.946 | -4.02223 | -3.59623 | 11.846 |
| 20 | 0.12 | 19.91 | -7.25071 | -7.46476 | 2.8675 | -7.25615 | -7.46651 | 2.8174 |
| 30 | 0.17 | 29.87 | -10.7881 | -11.3693 | 5.1123 | -10.8068 | -11.3702 | 4.9553 |
| 40 | 0.23 | 39.82 | -14.7174 | -15.2907 | 3.7499 | -14.7477 | -15.2921 | 3.5598 |
| 50 | 0.29 | 49.78 | -18.9053 | -19.2229 | 1.6520 | -18.9456 | -19.2245 | 1.4509 |
| 60 | 0.35 | 59.74 | -23.2691 | -23.1626 | 0.4595 | -23.3181 | -23.1646 | 0.6625 |
| 70 | 0.40 | 69.69 | -27.7606 | -27.1082 | 2.4066 | -27.8176 | -27.1105 | 2.6080 |
| 80 | 0.46 | 79.65 | -32.3504 | -31.0582 | 4.1604 | -32.4147 | -31.0610 | 4.3585 |
| 90 | 0.52 | 89.60 | -37.0191 | -35.0118 | 5.7333 | -37.0904 | -35.0148 | 5.9278 |
| 100 | 0.58 | 99.56 | -41.7535 | -38.9679 | 7.1483 | -41.8314 | -38.9636 | 7.3603 |
| 110 | 0.63 | 109.52 | -46.5435 | -42.9259 | 8.4276 | -46.6279 | -42.9254 | 8.6254 |
| 120 | 0.69 | 119.47 | -51.3820 | -46.8849 | 9.5917 | -51.4724 | -46.8890 | 9.7750 |
| 130 | 0.75 | 129.43 | -56.2629 | -50.8390 | 10.669 | -56.3594 | -50.8435 | 10.849 |
| 140 | 0.81 | 139.38 | -61.1817 | -54.7972 | 11.651 | -61.2840 | -54.8077 | 11.816 |
| 150 | 0.86 | 149.34 | -66.1345 | -58.7543 | 12.561 | -66.2425 | -58.7537 | 12.746 |
| 160 | 0.92 | 159.30 | -71.1180 | -62.7096 | 13.408 | -71.2315 | -62.7216 | 13.568 |
| 170 | 0.98 | 169.25 | -76.1294 | -66.6626 | 14.201 | -76.2485 | -66.6755 | 14.358 |

**Table 9c.** Test of the thermodynamic consistency of the isomorph-based empirically modified hypernetted-chain approximation (IEMHNC) and the empirically modified hypernetted-chain approximation (EMHNC); the reduced excess inverse isothermal compressibility due to the particle presence resulting from the statistical route $\mu^{\mathrm{p}}_{\mathrm{stat}}$ and the virial route $\mu^{\mathrm{p}}_{\mathrm{vir}}$. The absolute relative deviation between the two thermodynamic paths is also reported. **Results for $\boldsymbol{\kappa = 0.4}$**.

| $\Gamma$ | $\Gamma/\Gamma_{\mathrm{m}}$ | $\Gamma_{\mathrm{iso}}^{\mathrm{OCP}}$ | $\mu_{\mathrm{stat}}^{\mathrm{p,IEMHNC}}$ | $\mu_{\mathrm{vir}}^{\mathrm{p,IEMHNC}}$ | deviation (%) | $\mu_{\mathrm{stat}}^{\mathrm{p,EMHNC}}$ | $\mu_{\mathrm{vir}}^{\mathrm{p,EMHNC}}$ | deviation (%) |
|---|---|---|---|---|---|---|---|---|
| 10 | 0.06 | 9.72 | -3.97859 | -3.55672 | 11.861 | -3.95056 | -3.55658 | 11.078 |
| 20 | 0.11 | 19.44 | -7.18108 | -7.39577 | 2.9030 | -7.15975 | -7.39541 | 3.1866 |
| 30 | 0.17 | 29.17 | -10.6607 | -11.2715 | 5.4190 | -10.6794 | -11.2709 | 5.2480 |
| 40 | 0.22 | 38.89 | -14.5246 | -15.1646 | 4.2198 | -14.5800 | -15.1638 | 3.8504 |
| 50 | 0.28 | 48.61 | -18.6457 | -19.0685 | 2.2172 | -18.7316 | -19.0677 | 1.7623 |
| 60 | 0.34 | 58.33 | -22.9421 | -22.9783 | 0.1578 | -23.0542 | -22.9758 | 0.3414 |
| 70 | 0.39 | 68.06 | -27.3657 | -26.8978 | 1.7395 | -27.5011 | -26.8968 | 2.2466 |
| 80 | 0.45 | 77.78 | -31.8871 | -30.8201 | 3.4621 | -32.0438 | -30.8190 | 3.9739 |
| 90 | 0.50 | 87.50 | -36.4870 | -34.7427 | 5.0206 | -36.6634 | -34.7415 | 5.5320 |
| 100 | 0.56 | 97.22 | -41.1520 | -38.6751 | 6.4045 | -41.3471 | -38.6739 | 6.9123 |
| 110 | 0.62 | 106.95 | -45.8724 | -42.6069 | 7.6643 | -46.0854 | -42.6057 | 8.1674 |
| 120 | 0.67 | 116.67 | -50.6408 | -46.5410 | 8.8089 | -50.8711 | -46.5396 | 9.3070 |
| 130 | 0.73 | 126.39 | -55.4513 | -50.4701 | 9.8695 | -55.6984 | -50.4687 | 10.362 |
| 140 | 0.78 | 136.11 | -60.2993 | -54.4153 | 10.813 | -60.5629 | -54.4139 | 11.300 |
| 150 | 0.84 | 145.83 | -65.1810 | -58.3534 | 11.700 | -65.4607 | -58.3617 | 12.164 |
| 160 | 0.90 | 155.56 | -70.0931 | -62.2935 | 12.521 | -70.3888 | -62.2919 | 12.998 |
| 170 | 0.95 | 165.28 | -75.0330 | -66.2345 | 13.284 | -75.3442 | -66.2329 | 13.757 |

**Table 9d.** Test of the thermodynamic consistency of the isomorph-based empirically modified hypernetted-chain approximation (IEMHNC) and the empirically modified hypernetted-chain approximation (EMHNC); the reduced excess inverse isothermal compressibility due to the particle presence resulting from the statistical route $\mu^{\mathrm{p}}_{\mathrm{stat}}$ and the virial route $\mu^{\mathrm{p}}_{\mathrm{vir}}$. The absolute relative deviation between the two thermodynamic paths is also reported. **Results for $\boldsymbol{\kappa = 0.6}$**.

| $\Gamma$ | $\Gamma/\Gamma_{\mathrm{m}}$ | $\Gamma_{\mathrm{iso}}^{\mathrm{OCP}}$ | $\mu_{\mathrm{stat}}^{\mathrm{p,IEMHNC}}$ | $\mu_{\mathrm{vir}}^{\mathrm{p,IEMHNC}}$ | deviation (%) | $\mu_{\mathrm{stat}}^{\mathrm{p,EMHNC}}$ | $\mu_{\mathrm{vir}}^{\mathrm{p,EMHNC}}$ | deviation (%) |
|---|---|---|---|---|---|---|---|---|
| 10 | 0.05 | 9.26 | -3.91432 | -3.49060 | 12.139 | -3.83589 | -3.49060 | 9.8918 |
| 20 | 0.11 | 18.51 | -7.10734 | -7.27950 | 2.3649 | -7.00440 | -7.27907 | 3.7734 |
| 30 | 0.16 | 27.77 | -10.5066 | -11.1059 | 5.3958 | -10.4735 | -11.1052 | 5.6886 |
| 40 | 0.21 | 37.03 | -14.2735 | -14.9513 | 4.5337 | -14.3084 | -14.9505 | 4.2946 |
| 50 | 0.27 | 46.28 | -18.2939 | -18.8076 | 2.7312 | -18.3850 | -18.8065 | 2.2416 |
| 60 | 0.32 | 55.54 | -22.4882 | -22.6717 | 0.8095 | -22.6263 | -22.6707 | 0.1959 |
| 70 | 0.37 | 64.79 | -26.8090 | -26.5420 | 1.0058 | -26.9877 | -26.5410 | 1.6831 |
| 80 | 0.43 | 74.05 | -31.2267 | -30.4174 | 2.6607 | -31.4418 | -30.4163 | 3.3717 |
| 90 | 0.48 | 83.31 | -35.7220 | -34.2963 | 4.1571 | -35.9707 | -34.2952 | 4.8854 |
| 100 | 0.53 | 92.56 | -40.2815 | -38.1787 | 5.5079 | -40.5616 | -38.1776 | 6.2445 |
| 110 | 0.59 | 101.82 | -44.8955 | -42.0638 | 6.7318 | -45.2055 | -42.0628 | 7.4715 |
| 120 | 0.64 | 111.08 | -49.5565 | -45.9514 | 7.8456 | -49.8955 | -45.9503 | 8.5857 |
| 130 | 0.69 | 120.33 | -54.2590 | -49.8411 | 8.8639 | -54.6260 | -49.8401 | 9.6026 |
| 140 | 0.75 | 129.59 | -58.9982 | -53.7329 | 9.7989 | -59.3927 | -53.7319 | 10.535 |
| 150 | 0.80 | 138.84 | -63.7705 | -57.6257 | 10.663 | -64.1920 | -57.6247 | 11.397 |
| 160 | 0.86 | 148.10 | -68.5726 | -61.5191 | 11.465 | -69.0209 | -61.5181 | 12.196 |
| 170 | 0.91 | 157.36 | -73.4018 | -65.4145 | 12.210 | -73.8765 | -65.4135 | 12.938 |
| 180 | 0.96 | 166.61 | -78.2560 | -69.3109 | 12.906 | -78.7569 | -69.3100 | 13.630 |

**Table 9e.** Test of the thermodynamic consistency of the isomorph-based empirically modified hypernetted-chain approximation (IEMHNC) and the empirically modified hypernetted-chain approximation (EMHNC); the reduced excess inverse isothermal compressibility due to the particle presence resulting from the statistical route $\mu_{\mathrm{stat}}^{\mathrm{p}}$ and the virial route $\mu_{\mathrm{vir}}^{\mathrm{p}}$. The absolute relative deviation between the two thermodynamic paths is also reported. **Results for $\boldsymbol{\kappa = 0.8}$**.

| $\Gamma$ | $\Gamma/\Gamma_{\mathrm{m}}$ | $\Gamma_{\mathrm{iso}}^{\mathrm{OCP}}$ | $\mu_{\mathrm{stat}}^{\mathrm{p,IEMHNC}}$ | $\mu_{\mathrm{vir}}^{\mathrm{p,IEMHNC}}$ | deviation (%) | $\mu_{\mathrm{stat}}^{\mathrm{p,EMHNC}}$ | $\mu_{\mathrm{vir}}^{\mathrm{p,EMHNC}}$ | deviation (%) |
|---|---|---|---|---|---|---|---|---|
| 20 | 0.10 | 17.19 | -7.02965 | -7.11767 | 1.2366 | -6.79747 | -7.11705 | 4.4904 |
| 30 | 0.15 | 25.79 | -10.3339 | -10.8764 | 4.9874 | -10.1978 | -10.8759 | 6.2351 |
| 40 | 0.20 | 34.38 | -13.9763 | -14.6536 | 4.6223 | -13.9441 | -14.6531 | 4.8386 |
| 50 | 0.25 | 42.98 | -17.8658 | -18.4430 | 3.1299 | -17.9194 | -18.4425 | 2.8363 |
| 60 | 0.30 | 51.57 | -21.9270 | -22.2387 | 1.4016 | -22.0514 | -22.2389 | 0.8434 |
| 70 | 0.35 | 60.17 | -26.1134 | -26.0449 | 0.2632 | -26.2978 | -26.0447 | 0.9716 |
| 80 | 0.40 | 68.76 | -30.3955 | -29.8541 | 1.8135 | -30.6327 | -29.8542 | 2.6077 |
| 90 | 0.45 | 77.36 | -34.7540 | -33.6675 | 3.2272 | -35.0391 | -33.6678 | 4.0729 |
| 100 | 0.50 | 85.95 | -39.1754 | -37.4844 | 4.5113 | -39.5050 | -37.4849 | 5.3890 |
| 110 | 0.55 | 94.55 | -43.6500 | -41.3041 | 5.6796 | -44.0218 | -41.3050 | 6.5775 |
| 120 | 0.60 | 103.14 | -48.1706 | -45.1264 | 6.7458 | -48.5829 | -45.1275 | 7.6570 |
| 130 | 0.65 | 111.74 | -52.7314 | -48.9508 | 7.7231 | -53.1830 | -48.9521 | 8.6429 |
| 140 | 0.70 | 120.33 | -57.3279 | -52.7770 | 8.6229 | -57.8180 | -52.7785 | 9.5484 |
| 150 | 0.75 | 128.93 | -61.9565 | -56.6049 | 9.4542 | -62.4845 | -56.6066 | 10.384 |
| 160 | 0.80 | 137.52 | -66.6139 | -60.4336 | 10.227 | -67.1795 | -60.4360 | 11.158 |
| 170 | 0.85 | 146.12 | -71.2978 | -64.2647 | 10.944 | -71.9005 | -64.2667 | 11.878 |
| 180 | 0.90 | 154.71 | -76.0058 | -68.0966 | 11.615 | -76.6455 | -68.0988 | 12.550 |
| 190 | 0.95 | 163.31 | -80.7360 | -71.9293 | 12.243 | -81.4126 | -71.9316 | 13.180 |

**Table 9f.** Test of the thermodynamic consistency of the isomorph-based empirically modified hypernetted-chain approximation (IEMHNC) and the empirically modified hypernetted-chain approximation (EMHNC); the reduced excess inverse isothermal compressibility due to the particle presence resulting from the statistical route $\mu_{\mathrm{stat}}^{\mathrm{p}}$ and the virial route $\mu_{\mathrm{vir}}^{\mathrm{p}}$. The absolute relative deviation between the two thermodynamic paths is also reported. **Results for $\boldsymbol{\kappa = 1.0}$**.

| $\Gamma$ | $\Gamma/\Gamma_{\mathrm{m}}$ | $\Gamma_{\mathrm{iso}}^{\mathrm{OCP}}$ | $\mu_{\mathrm{stat}}^{\mathrm{p,IEMHNC}}$ | $\mu_{\mathrm{vir}}^{\mathrm{p,IEMHNC}}$ | deviation (%) | $\mu_{\mathrm{stat}}^{\mathrm{p,EMHNC}}$ | $\mu_{\mathrm{vir}}^{\mathrm{p,EMHNC}}$ | deviation (%) |
|---|---|---|---|---|---|---|---|---|
| 20 | 0.09 | 15.61 | -6.93756 | -6.91163 | 0.3750 | -6.54806 | -6.91173 | 5.2617 |
| 30 | 0.14 | 23.41 | -10.1413 | -10.5823 | 4.1673 | -9.86335 | -10.5827 | 6.7970 |
| 40 | 0.18 | 31.21 | -13.6370 | -14.2736 | 4.4602 | -13.5008 | -14.2741 | 5.4172 |
| 50 | 0.23 | 39.01 | -17.3685 | -17.9774 | 3.3868 | -17.3523 | -17.9783 | 3.4820 |
| 60 | 0.28 | 46.82 | -21.2685 | -21.6901 | 1.9438 | -21.3505 | -21.6915 | 1.5720 |
| 70 | 0.32 | 54.62 | -25.2918 | -25.4096 | 0.4634 | -25.4563 | -25.4115 | 0.1764 |
| 80 | 0.37 | 62.42 | -29.4095 | -29.1344 | 0.9441 | -29.6456 | -29.1371 | 1.7454 |
| 90 | 0.41 | 70.22 | -33.6021 | -32.8637 | 2.2469 | -33.9024 | -32.8670 | 3.1503 |
| 100 | 0.46 | 78.03 | -37.8563 | -36.5967 | 3.4418 | -38.2156 | -36.6007 | 4.4123 |
| 110 | 0.51 | 85.83 | -42.1622 | -40.3327 | 4.5360 | -42.5771 | -40.3374 | 5.5522 |
| 120 | 0.55 | 93.63 | -46.5127 | -44.0715 | 5.5391 | -46.9805 | -44.0768 | 6.5878 |
| 130 | 0.60 | 101.43 | -50.9021 | -47.8126 | 6.4616 | -51.4212 | -47.8186 | 7.5340 |
| 140 | 0.64 | 109.24 | -55.3259 | -51.5557 | 7.3129 | -55.8952 | -51.5623 | 8.4033 |
| 150 | 0.69 | 117.04 | -59.7806 | -55.3005 | 8.1013 | -60.3992 | -55.3077 | 9.2058 |
| 160 | 0.74 | 124.84 | -64.2631 | -59.0469 | 8.8339 | -64.9305 | -59.0546 | 9.9499 |
| 170 | 0.78 | 132.64 | -68.7709 | -62.7947 | 9.5171 | -69.4868 | -62.8030 | 10.643 |
| 180 | 0.83 | 140.45 | -73.3020 | -66.5437 | 10.156 | -74.0661 | -66.5525 | 11.290 |
| 190 | 0.87 | 148.25 | -77.8543 | -70.2938 | 10.756 | -78.6666 | -70.3030 | 11.896 |
| 200 | 0.92 | 156.05 | -82.4263 | -74.0449 | 11.319 | -83.2867 | -74.0545 | 12.467 |
| 210 | 0.97 | 163.85 | -87.0166 | -77.7968 | 11.851 | -87.9251 | -77.8068 | 13.004 |

**Table 9g.** Test of the thermodynamic consistency of the isomorph-based empirically modified hypernetted-chain approximation (IEMHNC) and the empirically modified hypernetted-chain approximation (EMHNC); the reduced excess inverse isothermal compressibility due to the particle presence resulting from the statistical route $\mu_{\mathrm{stat}}^{\mathrm{p}}$ and the virial route $\mu_{\mathrm{vir}}^{\mathrm{p}}$. The absolute relative deviation between the two thermodynamic paths is also reported. **Results for $\boldsymbol{\kappa = 1.2}$**.

| $\Gamma$ | $\Gamma/\Gamma_{\mathrm{m}}$ | $\Gamma_{\mathrm{iso}}^{\mathrm{OCP}}$ | $\mu_{\mathrm{stat}}^{\mathrm{p,IEMHNC}}$ | $\mu_{\mathrm{vir}}^{\mathrm{p,IEMHNC}}$ | deviation (%) | $\mu_{\mathrm{stat}}^{\mathrm{p,EMHNC}}$ | $\mu_{\mathrm{vir}}^{\mathrm{p,EMHNC}}$ | deviation (%) |
|---|---|---|---|---|---|---|---|---|
| 20 | 0.08 | 13.89 | -6.81650 | -6.66484 | 2.2755 | -6.26617 | -6.66557 | 5.9920 |
| 30 | 0.12 | 20.83 | -9.92585 | -10.2289 | 2.9628 | -9.48219 | -10.2307 | 7.3162 |
| 40 | 0.16 | 27.78 | -13.2605 | -13.8157 | 4.0190 | -12.9940 | -13.8180 | 5.9635 |
| 50 | 0.21 | 34.72 | -16.8122 | -17.4160 | 3.4665 | -16.7028 | -17.4191 | 4.1123 |
| 60 | 0.25 | 41.67 | -20.5266 | -21.0257 | 2.3733 | -20.5473 | -21.0298 | 2.2947 |
| 70 | 0.29 | 48.61 | -24.3620 | -24.6426 | 1.1386 | -24.4916 | -24.6480 | 0.6345 |
| 80 | 0.33 | 55.55 | -28.2901 | -28.2653 | 0.0878 | -28.5137 | -28.2720 | 0.8547 |
| 90 | 0.37 | 62.50 | -32.2917 | -31.8927 | 1.2511 | -32.5987 | -31.9008 | 2.1878 |
| 100 | 0.41 | 69.44 | -36.3535 | -35.5241 | 2.3347 | -36.7365 | -35.5336 | 3.3854 |
| 110 | 0.45 | 76.39 | -40.4656 | -39.1588 | 3.3372 | -40.9195 | -39.1697 | 4.4673 |
| 120 | 0.49 | 83.33 | -44.6209 | -42.7965 | 4.2630 | -45.1420 | -42.8087 | 5.4505 |
| 130 | 0.53 | 90.28 | -48.8136 | -46.4366 | 5.1188 | -49.3995 | -46.4502 | 6.3495 |
| 140 | 0.58 | 97.22 | -53.0395 | -50.0790 | 5.9117 | -53.6884 | -50.0938 | 7.1757 |
| 150 | 0.62 | 104.16 | -57.2949 | -53.7233 | 6.6482 | -58.0056 | -53.7394 | 7.9388 |
| 160 | 0.66 | 111.11 | -61.5770 | -57.3693 | 7.3344 | -62.3487 | -57.3866 | 8.6469 |
| 170 | 0.70 | 118.05 | -65.8832 | -61.0168 | 7.9756 | -66.7156 | -61.0352 | 9.3067 |
| 180 | 0.74 | 125.00 | -70.2116 | -64.6657 | 8.5762 | -71.1042 | -64.6851 | 9.9236 |
| 190 | 0.78 | 131.94 | -74.5602 | -68.3157 | 9.1407 | -75.5130 | -68.3362 | 10.502 |
| 200 | 0.82 | 138.89 | -78.9276 | -71.9669 | 9.6722 | -79.9406 | -71.9883 | 11.047 |
| 210 | 0.86 | 145.83 | -83.3125 | -75.6190 | 10.174 | -84.3856 | -75.6413 | 11.560 |
| 220 | 0.90 | 152.77 | -87.7135 | -79.2721 | 10.649 | -88.8470 | -79.2953 | 12.046 |
| 230 | 0.95 | 159.72 | -92.1297 | -82.9259 | 11.099 | -93.3235 | -82.9499 | 12.506 |
| 240 | 0.99 | 166.66 | -96.5600 | -86.5804 | 11.526 | -97.8143 | -86.6052 | 12.943 |

**Table 9h.** Test of the thermodynamic consistency of the isomorph-based empirically modified hypernetted-chain approximation (IEMHNC) and the empirically modified hypernetted-chain approximation (EMHNC); the reduced excess inverse isothermal compressibility due to the particle presence resulting from the statistical route $\mu_{\mathrm{stat}}^{\mathrm{p}}$ and the virial route $\mu_{\mathrm{vir}}^{\mathrm{p}}$. The absolute relative deviation between the two thermodynamic paths is also reported. **Results for $\boldsymbol{\kappa = 1.4}$.**

| $\Gamma$ | $\Gamma/\Gamma_{\mathrm{m}}$ | $\Gamma_{\mathrm{iso}}^{\mathrm{OCP}}$ | $\mu_{\mathrm{stat}}^{\mathrm{p,IEMHNC}}$ | $\mu_{\mathrm{vir}}^{\mathrm{p,IEMHNC}}$ | deviation (%) | $\mu_{\mathrm{stat}}^{\mathrm{p,EMHNC}}$ | $\mu_{\mathrm{vir}}^{\mathrm{p,EMHNC}}$ | deviation (%) |
|---|---|---|---|---|---|---|---|---|
| 20 | 0.07 | 12.15 | -6.65075 | -6.38174 | 4.2153 | -5.96176 | -6.38363 | 6.6086 |
| 30 | 0.11 | 18.23 | -9.68342 | -9.82177 | 1.4086 | -9.06647 | -9.82564 | 7.7263 |
| 40 | 0.15 | 24.30 | -12.8539 | -13.2869 | 3.2591 | -12.4390 | -13.2920 | 6.4171 |
| 50 | 0.19 | 30.38 | -16.2116 | -16.7668 | 3.3111 | -15.9905 | -16.7733 | 4.6668 |
| 60 | 0.22 | 36.45 | -19.7221 | -20.2569 | 2.6401 | -19.6659 | -20.2651 | 2.9570 |
| 70 | 0.26 | 42.53 | -23.3496 | -23.7546 | 1.7050 | -23.4327 | -23.7649 | 1.3979 |
| 80 | 0.30 | 48.60 | -27.0679 | -27.2586 | 0.6996 | -27.2710 | -27.2710 | 0.0002 |
| 90 | 0.33 | 54.68 | -30.8582 | -30.7676 | 0.2945 | -31.1673 | -30.7823 | 1.2506 |
| 100 | 0.37 | 60.75 | -34.7072 | -34.2809 | 1.2438 | -35.1124 | -34.2979 | 2.3746 |
| 110 | 0.41 | 66.83 | -38.6054 | -37.7978 | 2.1366 | -39.0993 | -37.8172 | 3.3902 |
| 120 | 0.45 | 72.90 | -42.5453 | -41.3179 | 2.9708 | -43.1229 | -41.3396 | 4.3138 |
| 130 | 0.48 | 78.98 | -46.5215 | -44.8407 | 3.7485 | -47.1791 | -44.8648 | 5.1584 |
| 140 | 0.52 | 85.05 | -50.5295 | -48.3659 | 4.4734 | -51.2645 | -48.3923 | 5.9353 |
| 150 | 0.56 | 91.13 | -54.5658 | -51.8932 | 5.1500 | -55.3764 | -51.9218 | 6.6534 |
| 160 | 0.60 | 97.20 | -58.6274 | -55.4225 | 5.7827 | -59.5125 | -55.4533 | 7.3202 |
| 170 | 0.63 | 103.28 | -62.7121 | -58.9534 | 6.3758 | -63.6708 | -58.9862 | 7.9418 |
| 180 | 0.67 | 109.36 | -66.8179 | -62.4859 | 6.9328 | -67.8496 | -62.5206 | 8.5235 |
| 190 | 0.71 | 115.43 | -70.9428 | -66.0197 | 7.4571 | -72.0474 | -66.0564 | 9.0696 |
| 200 | 0.74 | 121.51 | -75.0856 | -69.5547 | 7.9519 | -76.2629 | -69.5932 | 9.5840 |
| 210 | 0.78 | 127.58 | -79.2449 | -73.0908 | 8.4197 | -80.4950 | -73.1310 | 10.070 |
| 220 | 0.82 | 133.66 | -83.4195 | -76.6280 | 8.8629 | -84.7425 | -76.6698 | 10.529 |
| 230 | 0.86 | 139.73 | -87.6084 | -80.1660 | 9.2837 | -89.0044 | -80.2094 | 10.965 |
| 240 | 0.89 | 145.81 | -91.8107 | -83.7049 | 9.6838 | -93.2800 | -83.7497 | 11.379 |
| 250 | 0.93 | 151.88 | -96.0257 | -87.2446 | 10.065 | -97.5684 | -87.2908 | 11.774 |
| 260 | 0.97 | 157.96 | -100.253 | -90.7849 | 10.429 | -101.869 | -90.8324 | 12.150 |

**Table 9i.** Test of the thermodynamic consistency of the isomorph-based empirically modified hypernetted-chain approximation (IEMHNC) and the empirically modified hypernetted-chain approximation (EMHNC); the reduced excess inverse isothermal compressibility due to the particle presence resulting from the statistical route $\mu_{\mathrm{stat}}^{\mathrm{p}}$ and the virial route $\mu_{\mathrm{vir}}^{\mathrm{p}}$. The absolute relative deviation between the two thermodynamic paths is also reported. **Results for $\boldsymbol{\kappa = 2.0}$.**

| $\Gamma$ | $\Gamma/\Gamma_{\mathrm{m}}$ | $\Gamma_{\mathrm{iso}}^{\mathrm{OCP}}$ | $\mu_{\mathrm{stat}}^{\mathrm{p,IEMHNC}}$ | $\mu_{\mathrm{vir}}^{\mathrm{p,IEMHNC}}$ | deviation (%) | $\mu_{\mathrm{stat}}^{\mathrm{p,EMHNC}}$ | $\mu_{\mathrm{vir}}^{\mathrm{p,EMHNC}}$ | deviation (%) |
|---|---|---|---|---|---|---|---|---|
| 20 | 0.05 | 7.50 | -5.79051 | -5.36037 | 8.0245 | -4.99905 | -5.39104 | 7.2712 |
| 40 | 0.09 | 15.00 | -11.4886 | -11.3845 | 0.9143 | -10.6249 | -11.4020 | 6.8156 |
| 60 | 0.14 | 22.50 | -17.1755 | -17.4730 | 1.7028 | -16.7737 | -17.4983 | 4.1408 |
| 80 | 0.18 | 29.99 | -23.1653 | -23.6021 | 1.8509 | -23.1936 | -23.6369 | 1.8754 |
| 100 | 0.23 | 37.49 | -29.4054 | -29.7561 | 1.1785 | -29.7863 | -29.8022 | 0.0535 |
| 120 | 0.27 | 44.99 | -35.8262 | -35.9279 | 0.2832 | -36.5046 | -35.9866 | 1.4394 |
| 140 | 0.32 | 52.49 | -42.3800 | -42.1135 | 0.6329 | -43.3212 | -42.1852 | 2.6928 |
| 160 | 0.36 | 59.99 | -49.0359 | -48.3101 | 1.5022 | -50.2184 | -48.3950 | 3.7678 |
| 180 | 0.41 | 67.49 | -55.7728 | -54.5158 | 2.3059 | -57.1841 | -54.6137 | 4.7065 |
| 200 | 0.45 | 74.98 | -62.5764 | -60.7288 | 3.0424 | -64.2088 | -60.8395 | 5.5379 |
| 220 | 0.50 | 82.48 | -69.4361 | -66.9483 | 3.7160 | -71.2854 | -67.0712 | 6.2832 |
| 240 | 0.55 | 89.98 | -76.3438 | -73.1730 | 4.3333 | -78.4083 | -73.3078 | 6.9577 |
| 260 | 0.59 | 97.48 | -83.2936 | -79.4024 | 4.9005 | -85.5725 | -79.5483 | 7.5730 |
| 280 | 0.64 | 104.98 | -90.2804 | -85.6358 | 5.4237 | -92.7742 | -85.7922 | 8.1382 |
| 300 | 0.68 | 112.48 | -97.3004 | -91.8720 | 5.9087 | -100.010 | -92.0389 | 8.6602 |
| 320 | 0.73 | 119.97 | -104.350 | -98.1124 | 6.3579 | -107.276 | -98.2879 | 9.1447 |
| 340 | 0.77 | 127.47 | -111.427 | -104.355 | 6.7773 | -114.571 | -104.539 | 9.5962 |
| 360 | 0.82 | 134.97 | -118.529 | -110.600 | 7.1696 | -121.891 | -110.792 | 10.018 |
| 380 | 0.86 | 142.47 | -125.654 | -116.847 | 7.5376 | -129.236 | -117.046 | 10.414 |
| 400 | 0.91 | 149.97 | -132.800 | -123.095 | 7.8836 | -136.602 | -123.301 | 10.787 |
| 420 | 0.95 | 157.47 | -139.965 | -129.345 | 8.2099 | -143.988 | -129.558 | 11.138 |
| 440 | 1.00 | 164.97 | -147.148 | -135.597 | 8.5183 | -151.393 | -135.814 | 11.471 |

**Table 9j.** Test of the thermodynamic consistency of the isomorph-based empirically modified hypernetted-chain approximation (IEMHNC) and the empirically modified hypernetted-chain approximation (EMHNC); the reduced excess inverse isothermal compressibility due to the particle presence resulting from the statistical route $\mu_{\mathrm{stat}}^{\mathrm{p}}$ and the virial route $\mu_{\mathrm{vir}}^{\mathrm{p}}$. The absolute relative deviation between the two thermodynamic paths is also reported. **Results for $\boldsymbol{\kappa} = \mathbf{2.6}$**.

| $\Gamma$ | $\Gamma/\Gamma_{\mathrm{m}}$ | $\Gamma_{\mathrm{iso}}^{\mathrm{OCP}}$ | $\mu_{\mathrm{stat}}^{\mathrm{p,IEMHNC}}$ | $\mu_{\mathrm{vir}}^{\mathrm{p,IEMHNC}}$ | deviation (%) | $\mu_{\mathrm{stat}}^{\mathrm{p,EMHNC}}$ | $\mu_{\mathrm{vir}}^{\mathrm{p,EMHNC}}$ | deviation (%) |
|---|---|---|---|---|---|---|---|---|
| 60 | 0.08 | 12.68 | -14.6585 | -14.3817 | 1.9246 | -13.8667 | -14.4187 | 3.8283 |
| 80 | 0.11 | 16.91 | -19.5314 | -19.5120 | 0.0991 | -19.1074 | -19.5600 | 2.3142 |
| 100 | 0.13 | 21.14 | -24.4809 | -24.6734 | 0.7803 | -24.4649 | -24.7365 | 1.0982 |
| 120 | 0.16 | 25.37 | -29.5388 | -29.8556 | 1.0612 | -29.9081 | -29.9313 | 0.0776 |
| 140 | 0.18 | 29.60 | -34.6975 | -35.0531 | 1.0144 | -35.4188 | -35.1460 | 0.7764 |
| 160 | 0.21 | 33.83 | -39.9416 | -40.2627 | 0.7975 | -40.9853 | -40.3744 | 1.5130 |
| 180 | 0.24 | 38.05 | -45.2564 | -45.4825 | 0.4971 | -46.5991 | -45.6140 | 2.1596 |
| 200 | 0.26 | 42.28 | -50.6298 | -50.7107 | 0.1595 | -52.2541 | -50.8629 | 2.7352 |
| 220 | 0.29 | 46.51 | -56.0526 | -55.9464 | 0.1898 | -57.9457 | -56.1197 | 3.2538 |
| 240 | 0.32 | 50.74 | -61.5172 | -61.1885 | 0.5372 | -63.6699 | -61.3831 | 3.7255 |
| 260 | 0.34 | 54.97 | -67.0181 | -66.4364 | 0.8756 | -69.4236 | -66.6522 | 4.1580 |
| 280 | 0.37 | 59.19 | -72.5505 | -71.6893 | 1.2013 | -75.2043 | -71.9262 | 4.5575 |
| 300 | 0.40 | 63.42 | -78.1108 | -76.9468 | 1.5128 | -81.0096 | -77.2046 | 4.9285 |
| 320 | 0.42 | 67.65 | -83.6959 | -82.2084 | 1.8094 | -86.8378 | -82.4866 | 5.2750 |
| 340 | 0.45 | 71.88 | -89.3033 | -87.4736 | 2.0917 | -92.6870 | -87.7719 | 5.5998 |
| 360 | 0.47 | 76.11 | -94.9309 | -92.7422 | 2.3600 | -98.5558 | -93.0601 | 5.9056 |
| 380 | 0.50 | 80.33 | -100.577 | -98.0139 | 2.6151 | -104.443 | -98.3507 | 6.1943 |
| 400 | 0.53 | 84.56 | -106.240 | -103.288 | 2.8578 | -110.347 | -103.644 | 6.4677 |
| 420 | 0.55 | 88.79 | -111.919 | -108.565 | 3.0889 | -116.267 | -108.938 | 6.7274 |
| 440 | 0.58 | 93.02 | -117.612 | -113.845 | 3.3091 | -122.202 | -114.235 | 6.9746 |
| 460 | 0.61 | 97.25 | -123.318 | -119.126 | 3.5193 | -128.151 | -119.532 | 7.2103 |
| 480 | 0.63 | 101.48 | -129.038 | -124.409 | 3.7201 | -134.113 | -124.832 | 7.4355 |
| 500 | 0.66 | 105.70 | -134.768 | -129.695 | 3.9122 | -140.088 | -130.132 | 7.6510 |
| 520 | 0.69 | 109.93 | -140.511 | -134.981 | 4.0962 | -146.075 | -135.433 | 7.8576 |
| 540 | 0.71 | 114.16 | -146.263 | -140.270 | 4.2726 | -152.072 | -140.735 | 8.0558 |
| 560 | 0.74 | 118.39 | -152.025 | -145.560 | 4.4420 | -158.080 | -146.038 | 8.2462 |
| 580 | 0.76 | 122.62 | -157.797 | -150.851 | 4.6048 | -164.098 | -151.341 | 8.4294 |
| 600 | 0.79 | 126.84 | -163.578 | -156.143 | 4.7614 | -170.126 | -156.645 | 8.6058 |
| 620 | 0.82 | 131.07 | -169.367 | -161.437 | 4.9122 | -176.162 | -161.950 | 8.7758 |
| 640 | 0.84 | 135.30 | -175.164 | -166.731 | 5.0576 | -182.207 | -167.255 | 8.9398 |
| 660 | 0.87 | 139.53 | -180.969 | -172.027 | 5.1979 | -188.260 | -172.560 | 9.0980 |
| 680 | 0.90 | 143.76 | -186.781 | -177.323 | 5.3334 | -194.320 | -177.866 | 9.2509 |
| 700 | 0.92 | 147.99 | -192.600 | -182.621 | 5.4643 | -200.387 | -183.172 | 9.3987 |
| 720 | 0.95 | 152.21 | -198.425 | -187.919 | 5.5910 | -206.462 | -188.478 | 9.5416 |
| 740 | 0.98 | 156.44 | -204.258 | -193.218 | 5.7137 | -212.542 | -193.784 | 9.6800 |

**Table 9k.** Test of the thermodynamic consistency of the isomorph-based empirically modified hypernetted-chain approximation (IEMHNC) and the empirically modified hypernetted-chain approximation (EMHNC); the reduced excess inverse isothermal compressibility due to the particle presence resulting from the statistical route $\mu_{\mathrm{stat}}^{\mathrm{p}}$ and the virial route $\mu_{\mathrm{vir}}^{\mathrm{p}}$. The absolute relative deviation between the two thermodynamic paths is also reported. **Results for $\boldsymbol{\kappa = 3.0}$**.

| $\Gamma$ | $\Gamma/\Gamma_{\mathrm{m}}$ | $\Gamma_{\mathrm{iso}}^{\mathrm{OCP}}$ | $\mu_{\mathrm{stat}}^{\mathrm{p,IEMHNC}}$ | $\mu_{\mathrm{vir}}^{\mathrm{p,IEMHNC}}$ | deviation (%) | $\mu_{\mathrm{stat}}^{\mathrm{p,EMHNC}}$ | $\mu_{\mathrm{vir}}^{\mathrm{p,EMHNC}}$ | deviation (%) |
|---|---|---|---|---|---|---|---|---|
| 50 | 0.04 | 6.96 | -10.6062 | -10.1233 | 4.7698 | -9.85302 | -10.2214 | 3.6042 |
| 100 | 0.08 | 13.92 | -21.6063 | -21.3799 | 1.0590 | -21.2047 | -21.4328 | 1.0645 |
| 150 | 0.13 | 20.87 | -32.5732 | -32.7274 | 0.4713 | -32.9877 | -32.8126 | 0.5337 |
| 200 | 0.17 | 27.83 | -43.8313 | -44.1501 | 0.7222 | -45.0177 | -44.2790 | 1.6683 |
| 250 | 0.21 | 34.79 | -55.3467 | -55.6195 | 0.4905 | -57.2212 | -55.8004 | 2.5463 |
| 300 | 0.25 | 41.75 | -67.0525 | -67.1229 | 0.1048 | -69.5586 | -67.3602 | 3.2636 |
| 350 | 0.30 | 48.71 | -78.9001 | -78.6528 | 0.3144 | -82.0046 | -78.9483 | 3.8713 |
| 400 | 0.34 | 55.67 | -90.8567 | -90.2041 | 0.7235 | -94.5417 | -90.5577 | 4.3994 |
| 450 | 0.38 | 62.62 | -102.900 | -101.773 | 1.1077 | -107.157 | -102.184 | 4.8669 |
| 500 | 0.42 | 69.58 | -115.015 | -113.357 | 1.4633 | -119.839 | -113.822 | 5.2866 |
| 550 | 0.46 | 76.54 | -127.190 | -124.953 | 1.7908 | -132.581 | -125.470 | 5.6674 |
| 600 | 0.51 | 83.50 | -139.417 | -136.559 | 2.0925 | -145.376 | -137.126 | 6.0159 |
| 650 | 0.55 | 90.46 | -151.688 | -148.175 | 2.3708 | -158.217 | -148.788 | 6.3371 |
| 700 | 0.59 | 97.41 | -163.999 | -159.799 | 2.6284 | -171.100 | -160.454 | 6.6346 |
| 750 | 0.63 | 104.37 | -176.345 | -171.430 | 2.8674 | -184.020 | -172.124 | 6.9115 |
| 800 | 0.68 | 111.33 | -188.724 | -183.067 | 3.0901 | -196.975 | -183.796 | 7.1701 |
| 850 | 0.72 | 118.29 | -201.131 | -194.709 | 3.2983 | -209.960 | -195.470 | 7.4126 |
| 900 | 0.76 | 125.25 | -213.564 | -206.355 | 3.4933 | -222.973 | -207.146 | 7.6403 |
| 950 | 0.80 | 132.21 | -226.022 | -218.006 | 3.6767 | -236.011 | -218.822 | 7.8549 |
| 1000 | 0.84 | 139.16 | -238.502 | -229.661 | 3.8496 | -249.072 | -230.499 | 8.0575 |
| 1050 | 0.89 | 146.12 | -251.002 | -241.320 | 4.0124 | -262.154 | -242.177 | 8.2490 |
| 1100 | 0.93 | 153.08 | -263.522 | -252.979 | 4.1675 | -275.255 | -253.854 | 8.4303 |
| 1150 | 0.97 | 160.04 | -276.060 | -264.642 | 4.3143 | -288.374 | -265.532 | 8.6024 |

**Table 9l.** Test of the thermodynamic consistency of the isomorph-based empirically modified hypernetted-chain approximation (IEMHNC) and the empirically modified hypernetted-chain approximation (EMHNC); the reduced excess inverse isothermal compressibility due to the particle presence resulting from the statistical route $\mu_{\mathrm{stat}}^{\mathrm{p}}$ and the virial route $\mu_{\mathrm{vir}}^{\mathrm{p}}$. The absolute relative deviation between the two thermodynamic paths is also reported. **Results for $\boldsymbol{\kappa = 3.6}$**.

| $\Gamma$ | $\Gamma/\Gamma_{\mathrm{m}}$ | $\Gamma_{\mathrm{iso}}^{\mathrm{OCP}}$ | $\mu_{\mathrm{stat}}^{\mathrm{p,IEMHNC}}$ | $\mu_{\mathrm{vir}}^{\mathrm{p,IEMHNC}}$ | deviation (%) | $\mu_{\mathrm{stat}}^{\mathrm{p,EMHNC}}$ | $\mu_{\mathrm{vir}}^{\mathrm{p,EMHNC}}$ | deviation (%) |
|---|---|---|---|---|---|---|---|---|
| 200 | 0.08 | 14.27 | -35.5545 | -35.3087 | 0.6964 | -35.7083 | -35.3559 | 0.9967 |
| 300 | 0.13 | 21.40 | -53.6839 | -53.8255 | 0.2631 | -54.9263 | -53.9240 | 1.8586 |
| 400 | 0.17 | 28.54 | -72.1410 | -72.4438 | 0.4180 | -74.4191 | -72.6179 | 2.4804 |
| 500 | 0.21 | 35.67 | -90.8727 | -91.1267 | 0.2788 | -94.1077 | -91.3911 | 2.9725 |
| 600 | 0.25 | 42.81 | -109.805 | -109.857 | 0.0475 | -113.948 | -110.219 | 3.3831 |
| 700 | 0.29 | 49.94 | -128.886 | -128.625 | 0.2031 | -133.910 | -129.086 | 3.7375 |
| 800 | 0.34 | 57.08 | -148.082 | -147.423 | 0.4472 | -153.973 | -147.981 | 4.0490 |
| 900 | 0.38 | 64.21 | -167.370 | -166.246 | 0.6762 | -174.123 | -166.898 | 4.3292 |
| 1000 | 0.42 | 71.35 | -186.733 | -185.090 | 0.8879 | -194.347 | -185.830 | 4.5837 |
| 1100 | 0.46 | 78.48 | -206.160 | -203.951 | 1.0829 | -214.636 | -204.773 | 4.8168 |
| 1200 | 0.50 | 85.62 | -225.641 | -222.828 | 1.2625 | -234.982 | -223.724 | 5.0319 |
| 1300 | 0.55 | 92.75 | -245.170 | -241.717 | 1.4284 | -255.377 | -242.681 | 5.2315 |
| 1400 | 0.59 | 99.89 | -264.741 | -260.618 | 1.5820 | -275.816 | -261.641 | 5.4176 |
| 1500 | 0.63 | 107.02 | -284.349 | -279.528 | 1.7248 | -296.295 | -280.604 | 5.5918 |
| 1600 | 0.67 | 114.16 | -303.992 | -298.447 | 1.8579 | -316.810 | -299.568 | 5.7554 |
| 1700 | 0.71 | 121.29 | -323.665 | -317.373 | 1.9825 | -337.391 | -318.533 | 5.9204 |
| 1800 | 0.76 | 128.43 | -343.366 | -336.306 | 2.0992 | -357.931 | -337.497 | 6.0547 |
| 1900 | 0.80 | 135.56 | -363.093 | -355.244 | 2.2093 | -378.533 | -356.460 | 6.1922 |
| 2000 | 0.84 | 142.70 | -382.843 | -374.188 | 2.3131 | -399.158 | -375.422 | 6.3224 |
| 2100 | 0.88 | 149.83 | -402.616 | -393.136 | 2.4114 | -419.805 | -394.383 | 6.4461 |
| 2200 | 0.93 | 156.97 | -422.409 | -412.088 | 2.5046 | -440.472 | -413.342 | 6.5637 |
| 2300 | 0.97 | 164.10 | -442.222 | -431.044 | 2.5931 | -461.158 | -432.299 | 6.6757 |

**Table 9m.** Test of the thermodynamic consistency of the isomorph-based empirically modified hypernetted-chain approximation (IEMHNC) and the empirically modified hypernetted-chain approximation (EMHNC); the reduced excess inverse isothermal compressibility due to the particle presence resulting from the statistical route $\mu_{\mathrm{stat}}^{\mathrm{p}}$ and the virial route $\mu_{\mathrm{vir}}^{\mathrm{p}}$. The absolute relative deviation between the two thermodynamic paths is also reported. **Results for $\boldsymbol{\kappa = 4.0}$**.

| $\Gamma$ | $\Gamma/\Gamma_{\mathrm{m}}$ | $\Gamma_{\mathrm{iso}}^{\mathrm{OCP}}$ | $\mu_{\mathrm{stat}}^{\mathrm{p,IEMHNC}}$ | $\mu_{\mathrm{vir}}^{\mathrm{p,IEMHNC}}$ | deviation (%) | $\mu_{\mathrm{stat}}^{\mathrm{p,EMHNC}}$ | $\mu_{\mathrm{vir}}^{\mathrm{p,EMHNC}}$ | deviation (%) |
|---|---|---|---|---|---|---|---|---|
| 200 | 0.05 | 8.94 | -30.8309 | -30.2954 | 1.7674 | -30.5828 | -30.3106 | 0.8981 |
| 400 | 0.10 | 17.89 | -62.3707 | -62.3167 | 0.0865 | -63.4726 | -62.3467 | 1.8057 |
| 600 | 0.16 | 26.83 | -94.3097 | -94.5898 | 0.2961 | -96.9431 | -94.7115 | 2.3562 |
| 800 | 0.21 | 35.77 | -126.720 | -126.996 | 0.2172 | -130.763 | -127.246 | 2.7641 |
| 1000 | 0.26 | 44.72 | -159.454 | -159.492 | 0.0239 | -164.831 | -159.884 | 3.0941 |
| 1200 | 0.31 | 53.66 | -192.411 | -192.054 | 0.1857 | -199.090 | -192.590 | 3.3751 |
| 1400 | 0.36 | 62.61 | -225.532 | -224.668 | 0.3845 | -233.499 | -225.339 | 3.6208 |
| 1600 | 0.42 | 71.55 | -258.780 | -257.323 | 0.5662 | -268.026 | -258.119 | 3.8383 |
| 1800 | 0.47 | 80.49 | -292.130 | -290.011 | 0.7306 | -302.659 | -290.917 | 4.0362 |
| 2000 | 0.52 | 89.44 | -325.565 | -322.727 | 0.8794 | -337.379 | -323.727 | 4.2169 |
| 2200 | 0.57 | 98.38 | -359.072 | -355.465 | 1.0146 | -372.173 | -356.544 | 4.3834 |
| 2400 | 0.63 | 107.32 | -392.641 | -388.223 | 1.1380 | -407.030 | -389.363 | 4.5375 |
| 2600 | 0.68 | 116.27 | -426.264 | -420.996 | 1.2514 | -441.944 | -422.183 | 4.6809 |
| 2800 | 0.73 | 125.21 | -459.937 | -453.783 | 1.3560 | -476.908 | -455.000 | 4.8149 |
| 3000 | 0.78 | 134.16 | -493.651 | -486.582 | 1.4527 | -511.915 | -487.814 | 4.9406 |
| 3200 | 0.83 | 143.10 | -527.405 | -519.391 | 1.5430 | -546.961 | -520.624 | 5.0588 |
| 3400 | 0.89 | 152.04 | -561.195 | -552.208 | 1.6274 | -582.043 | -553.429 | 5.1702 |
| 3600 | 0.94 | 160.99 | -595.017 | -585.033 | 1.7066 | -617.157 | -586.230 | 5.2757 |
| 3800 | 0.99 | 169.93 | -628.869 | -617.864 | 1.7810 | -652.301 | -619.024 | 5.3757 |

**Table 9n.** Test of the thermodynamic consistency of the isomorph-based empirically modified hypernetted-chain approximation (IEMHNC) and the empirically modified hypernetted-chain approximation (EMHNC); the reduced excess inverse isothermal compressibility due to the particle presence resulting from the statistical route $\mu_{\mathrm{stat}}^{\mathrm{p}}$ and the virial route $\mu_{\mathrm{vir}}^{\mathrm{p}}$. The absolute relative deviation between the two thermodynamic paths is also reported. **Results for $\boldsymbol{\kappa = 4.6}$**.

| $\Gamma$ | $\Gamma/\Gamma_{\mathrm{m}}$ | $\Gamma_{\mathrm{iso}}^{\mathrm{OCP}}$ | $\mu_{\mathrm{stat}}^{\mathrm{p,IEMHNC}}$ | $\mu_{\mathrm{vir}}^{\mathrm{p,IEMHNC}}$ | deviation (%) | $\mu_{\mathrm{stat}}^{\mathrm{p,EMHNC}}$ | $\mu_{\mathrm{vir}}^{\mathrm{p,EMHNC}}$ | deviation (%) |
|---|---|---|---|---|---|---|---|---|
| 500 | 0.06 | 10.81 | -63.2701 | -62.7412 | 0.8430 | -63.5179 | -62.6423 | 1.3978 |
| 1000 | 0.12 | 21.62 | -127.645 | -127.750 | 0.0824 | -129.960 | -127.644 | 1.8142 |
| 1500 | 0.17 | 32.43 | -192.764 | -193.110 | 0.1792 | -197.106 | -193.102 | 2.0740 |
| 2000 | 0.23 | 43.24 | -258.448 | -258.656 | 0.0805 | -264.668 | -258.788 | 2.2723 |
| 2500 | 0.29 | 54.05 | -324.490 | -324.331 | 0.0491 | -332.518 | -324.607 | 2.4373 |
| 3000 | 0.35 | 64.85 | -390.777 | -390.099 | 0.1738 | -400.585 | -390.505 | 2.5813 |
| 3500 | 0.41 | 75.66 | -457.244 | -455.939 | 0.2863 | -468.816 | -456.452 | 2.7087 |
| 4000 | 0.46 | 86.47 | -523.852 | -521.835 | 0.3866 | -537.184 | -522.427 | 2.8249 |
| 4500 | 0.52 | 97.28 | -590.574 | -587.775 | 0.4762 | -605.664 | -588.414 | 2.9316 |
| 5000 | 0.58 | 108.09 | -657.392 | -653.752 | 0.5568 | -674.238 | -654.407 | 3.0305 |
| 5500 | 0.64 | 118.90 | -724.292 | -719.759 | 0.6298 | -742.892 | -720.397 | 3.1226 |
| 6000 | 0.70 | 129.71 | -791.263 | -785.789 | 0.6965 | -811.615 | -786.380 | 3.2089 |
| 6500 | 0.76 | 140.52 | -858.295 | -851.840 | 0.7579 | -880.399 | -852.355 | 3.2902 |
| 7000 | 0.81 | 151.33 | -925.384 | -917.907 | 0.8146 | -949.237 | -918.318 | 3.3670 |
| 7500 | 0.87 | 162.14 | -992.518 | -983.988 | 0.8669 | -1018.12 | -984.268 | 3.4398 |
| 8000 | 0.93 | 172.95 | -1059.70 | -1050.08 | 0.9160 | -1087.06 | -1050.20 | 3.5090 |
| 8500 | 0.99 | 183.76 | -1126.92 | -1116.18 | 0.9620 | -1156.03 | -1116.13 | 3.5751 |

**Table 9o.** Test of the thermodynamic consistency of the isomorph-based empirically modified hypernetted-chain approximation (IEMHNC) and the empirically modified hypernetted-chain approximation (EMHNC); the reduced excess inverse isothermal compressibility due to the particle presence resulting from the statistical route $\mu_{\rm stat}^{\rm p}$ and the virial route $\mu_{\rm vir}^{\rm p}$. The absolute relative deviation between the two thermodynamic paths is also reported. **Results for $\boldsymbol{\kappa = 5.0}$**.

| $\Gamma$ | $\Gamma/\Gamma_{\rm m}$ | $\Gamma_{\rm iso}^{\rm OCP}$ | $\mu_{\rm stat}^{\rm p,IEMHNC}$ | $\mu_{\rm vir}^{\rm p,IEMHNC}$ | deviation (%) | $\mu_{\rm stat}^{\rm p,EMHNC}$ | $\mu_{\rm vir}^{\rm p,EMHNC}$ | deviation (%) |
|---|---|---|---|---|---|---|---|---|
| 1000 | 0.07 | 13.12 | -111.101 | -110.655 | 0.4033 | -111.896 | -110.423 | 1.3336 |
| 1500 | 0.10 | 19.69 | -167.316 | -167.301 | 0.0093 | -169.461 | -167.010 | 1.4678 |
| 2000 | 0.13 | 26.25 | -223.835 | -224.104 | 0.1201 | -227.306 | -223.802 | 1.5659 |
| 2500 | 0.17 | 32.81 | -280.628 | -281.008 | 0.1353 | -285.344 | -280.725 | 1.6454 |
| 3000 | 0.20 | 39.37 | -337.626 | -337.987 | 0.1068 | -343.526 | -337.739 | 1.7135 |
| 3500 | 0.23 | 45.94 | -394.778 | -395.025 | 0.0627 | -401.823 | -394.819 | 1.7740 |
| 4000 | 0.27 | 52.50 | -452.049 | -452.112 | 0.0141 | -460.213 | -451.947 | 1.8290 |
| 4500 | 0.30 | 59.06 | -509.415 | -509.240 | 0.0343 | -518.682 | -509.112 | 1.8797 |
| 5000 | 0.33 | 65.62 | -566.859 | -566.402 | 0.0807 | -577.218 | -566.304 | 1.9271 |
| 5500 | 0.37 | 72.19 | -624.369 | -623.593 | 0.1244 | -635.812 | -623.517 | 1.9718 |
| 6000 | 0.40 | 78.75 | -681.936 | -680.810 | 0.1653 | -694.457 | -680.745 | 2.0142 |
| 6500 | 0.43 | 85.31 | -739.551 | -738.049 | 0.2036 | -753.151 | -737.984 | 2.0552 |
| 7000 | 0.46 | 91.87 | -797.211 | -795.307 | 0.2394 | -811.877 | -795.231 | 2.0932 |
| 7500 | 0.50 | 98.43 | -854.909 | -852.581 | 0.2730 | -870.643 | -852.483 | 2.1302 |
| 8000 | 0.53 | 105.00 | -912.643 | -909.871 | 0.3046 | -929.441 | -909.737 | 2.1660 |
| 8500 | 0.56 | 111.56 | -970.408 | -967.173 | 0.3344 | -988.270 | -966.992 | 2.2004 |
| 9000 | 0.60 | 118.12 | -1028.20 | -1024.49 | 0.3626 | -1047.13 | -1024.25 | 2.2336 |
| 9500 | 0.63 | 124.68 | -1086.02 | -1081.81 | 0.3893 | -1106.01 | -1081.50 | 2.2658 |
| 10000 | 0.66 | 131.25 | -1143.87 | -1139.15 | 0.4147 | -1164.91 | -1138.75 | 2.2969 |
| 10500 | 0.70 | 137.81 | -1201.74 | -1196.49 | 0.4389 | -1223.83 | -1196.00 | 2.3272 |
| 11000 | 0.73 | 144.37 | -1259.63 | -1253.84 | 0.4620 | -1282.78 | -1253.25 | 2.3565 |
| 11500 | 0.76 | 150.93 | -1317.54 | -1311.19 | 0.4841 | -1341.74 | -1310.49 | 2.3851 |
| 12000 | 0.80 | 157.49 | -1375.47 | -1368.55 | 0.5053 | -1400.72 | -1367.72 | 2.4129 |
| 12500 | 0.83 | 164.06 | -1433.41 | -1425.92 | 0.5254 | -1459.72 | -1424.95 | 2.4401 |
| 13000 | 0.86 | 170.62 | -1491.37 | -1483.29 | 0.5449 | -1518.73 | -1482.18 | 2.4665 |
| 13500 | 0.90 | 177.18 | -1549.35 | -1540.67 | 0.5637 | -1577.76 | -1539.40 | 2.4923 |
| 14000 | 0.93 | 183.74 | -1607.34 | -1598.05 | 0.5818 | -1636.80 | -1596.61 | 2.5175 |
| 14500 | 0.96 | 190.31 | -1665.35 | -1655.43 | 0.5993 | -1695.86 | -1653.82 | 2.5422 |
| 15000 | 1.00 | 196.87 | -1723.37 | -1712.82 | 0.6161 | -1754.93 | -1711.02 | 2.5664 |
